# Supplementary material for: Gradient-free optimization of highly smooth functions: improved analysis and a new algorithm
Source: arXiv:2306.02159 source file (2023-06-03)
Supplement: Supplementary file 1 [file appendixV2.tex]

\clearpage
\appendix
% \setcounter{page}{1}
\begin{center}
    {\LARGE\bf Supplementary material}
\end{center}

\paragraph{Additional notation for appendix.} Let $\bW_1, \bW_2$ be two random variables, we write $\bW_1 \stackrel{d}{=} \bW_2$ to denote their equality in distribution.

% \startcontents[appendices]
% \printcontents[appendices]{l}{1}{\setcounter{tocdepth}{1}}
% % \begin{center}
% %     \Large Supplementary material
% % \end{center}

\section{Consequences of smoothness assumption}

\begin{remark}
One can verify that for all $k \in \bbN \setminus \{0\}$ and all $\bh \in \bbR^d$ it holds that
\begin{align*}
    f^{(k)}(\bx)[\bh]^k
    &= 
    \sum_{|\bm_1| = \ldots = |\bm_k| = 1} D^{\bm_1 + \ldots + \bm_k}f(\bx) h^{\bm_1 + \ldots + \bm_k}
    =
    \sum_{|\bm| = k} \frac{k!}{\bm!}D^{\bm}f(\bx) h^{\bm}\enspace.
\end{align*}
\end{remark}


\begin{lemma}
\label{lem:f_to_grad}
Assume that $f \in \mathcal{F}_{\beta}(L)$ for some $\beta \geq 2$ and $L > 0$.
% continuously differentiable and that there exist $\alpha \in [0, 1]$ and $L > 0$ such that for all $x, y \in \bbR^d$
% \begin{align}
%     \norm{f^{(\ell)}(x) - f^{(\ell)}(y)} \leq L \|x - y\|^\alpha \enspace.\label{eq:holder_alternative}
% \end{align}
Then, for any $\bv \in \bbR^d$ with $\|\bv\| = 1$ the function $g_{\bv}(\bx) \equiv \scalar{\bv}{\nabla f(\bx)} \in \mathcal{F}_{\beta - 1}(L)$.
% % Then,
% \begin{align*}
%     \norm{g^{(\ell - 1)}_v(x) - g^{(\ell - 1)}_v(y)} \leq L \|x - y\|^\alpha\enspace.
% \end{align*}
\end{lemma}
\begin{proof}
Set $\ell \triangleq \floor{\beta}$.
Note that since $f$ is $\ell$ times continuously differentiable, then $g_{\bv}$ is $\ell - 1$ times continuously differentiable.
Furthermore, for any $\bh^1, \ldots, \bh^{\ell - 1} \in \bbR^d$
\begin{align*}
    g^{(\ell - 1)}_{\bv}(\bx)[\bh^1, \ldots, &\bh^{\ell - 1}]
    =
    \sum_{|\bm_1| = \ldots = |\bm_{\ell - 1}| = 1} D^{\bm_1 + \ldots + \bm_{\ell-1}} g_{\bv}(\bx) h_1^{\bm_1} \cdot \ldots \cdot \bh_{\ell - 1}^{m_{\ell - 1}}\\
    &=
    \sum_{|\bm_1| = \ldots = |\bm_{\ell - 1}| = 1} D^{\bm_1 + \ldots + \bm_{\ell-1}} \parent{\sum_{|\bm_\ell| = 1}D^{\bm_\ell}f(\bx)v^{\bm_\ell}} \bh_1^{\bm_1} \cdot \ldots \cdot \bh_{\ell - 1}^{\bm_{\ell - 1}}\\
    &=
     \sum_{|\bm_1| = \ldots = |\bm_{\ell}| = 1} D^{\bm_1 + \ldots + \bm_\ell} f(\bx) h_1^{\bm_1} \cdot \ldots \cdot \bh_{\ell - 1}^{\bm_{\ell - 1}}\bv^{\bm_\ell}\\
    &=
    f^{(\ell)}(\bx)[\bh^1, \ldots, \bh^{\ell - 1}, \bv]\enspace.
\end{align*}
Hence, for any $\bx, \bz \in \bbR^d$ we can write by definition of the norm of a $\ell{-}1$-linear form
\begin{align*}
    (*) &= \norm{g^{(\ell - 1)}_{\bv}(\bx) - g^{(\ell - 1)}_{\bv}(\bz)}\\
        &= \sup\enscond{\abs{g^{(\ell - 1)}_v(\bx)[\bh^1, \ldots, \bh^{\ell-1}] - g^{(\ell - 1)}_{\bv}(\bz)[\bh^1, \ldots, \bh^{\ell-1}]}}{\|\bh^j\| = 1\,\,j \in [\ell-1]}\\
        &=
        \sup\enscond{\abs{f^{(\ell)}(\bx)[\bh^1, \ldots, \bh^{\ell - 1}, \bv] - f^{(\ell)}(\bz)[\bh^1, \ldots, \bh^{\ell - 1}, \bv]}}{\|\bh^j\| = 1\,\,j \in [\ell-1]}\\
        &\leq
        \sup\enscond{\abs{f^{(\ell)}(\bx)[\bh^1, \ldots, \bh^{\ell - 1}, \bh^\ell] - f^{(\ell)}(\bz)[\bh^1, \ldots, \bh^{\ell - 1}, \bh^\ell]}}{\|\bh^j\| = 1\,\,j \in [\ell]}\\
        &=
        \norm{f^{(\ell)}(\bx) - f^{(\ell)}(\bz)} \leq L \|\bx - \bz\|^{\beta - \ell}\enspace.
\end{align*}
The proof is concluded.
\end{proof}



\begin{lemma}
\label{lem:holder_to_taylor}
Fix some real $\beta \geq 2$.
Assume that $f : \bbR^d \to \bbR$ is $(\beta, L)$-(modified) H\"older.
Then, for all $\bx, \bz \in \bbR^d$ it holds that
\begin{equation*}
\bigg|f(\bx)-\sum_{0\le |\bm|\leq \ell} \frac{1}{\bm!}D^{\bm}f(\bz)(\bx-\bz)^{\bm} \bigg|\leq \frac{L}{\ell!} \|\bx-\bz\|^{\beta},
\end{equation*}
\end{lemma}
\begin{proof}
Fix some $\bx, \bz \in \bbR^d$. By Taylor's theorem there exists $c \in (0, 1)$ such that
\begin{align*}
    f(\bx) = \sum_{0\le |\bm|\leq \ell -1} \frac{1}{\bm!}D^{\bm}f(\bz)(\bx-\bz)^{\bm} + \sum_{|\bm| = \ell} \frac{1}{\bm!}D^{\bm}f(\bz + c(\bx - \bz))(\bx-\bz)^{\bm}\enspace.
\end{align*}
Thus, we can write
\begin{align*}
    \bigg|f(\bx)-\sum_{|\bm|\leq \ell} \frac{1}{\bm!}D^{\bm}f(\bz)(\bx-\bz)^{m} \bigg|
    &=
    \abs{\sum_{ |\bm| = \ell} \frac{1}{\bm!}\left(D^{\bm}f(\bz + c(\bx - \bz)) - D^{\bm}f(\bz)\right)(\bx-\bz)^{\bm}}\\
    &=
    \frac{1}{\ell!}\abs{f^{(\ell)}(\bz + c(\bx - \bz))[\bx - \bz]^{\ell} - f^{(\ell)}(\bz)[\bx - \bz]^\ell}\\
    &\leq
    \frac{L}{\ell!} \norm{\bx - \bz}^{\ell} \norm{c(\bx - 
    \bz)}^{\beta - \ell} \leq \frac{L}{\ell!}\norm{\bx - \bz}^\beta
\end{align*}

% \begin{align*}
%     f(x) = \sum_{k = 0}^\ell \frac{1}{k!}f^{(k)}(y)[x - y]^k
% \end{align*}

\end{proof}



\section{A descent lemma for stochastic gradient}

% All methods considered in this work are based on the iteration of the following type
% \begin{align}
%     \label{eq:algo_general}
%     \bx_1 \in \bbR^d\,,\qquad \bx_{t+1} = \bx_t - \eta_t {\bg}_t\enspace,
% \end{align}
% where $\bx_1$ is an initialization, $\eta_t$ is a (possibly varying) step-size, and $\hat{g}_t$ is a vector determining the (anti) direction of the update. Typically, and, as is the case here, $\bg_t$ is built to estimate $\nabla f(\bx_t)$---mimicking the gradient descent update rule.
% The next result is elementary. It allows us to present the derived results in a unified plug-and-play fashion.

\begin{proof}[Proof of Lemma~\ref{lem:general}]
    For compactness we write $\Exp_t[\cdot]$ in place of $\Exp[\cdot \mid \bx_t]$.
    Using Lipschitz continuity of $\nabla f$ and the update of the algorithm in Eq.~\eqref{eq:algo_general} we can write
    \begin{align*}
        \Exp_t[f(\bx_{t+1})]
        &\leq
        f(\bx_t) - \eta_t \scalar{\nabla f(\bx_t)}{\Exp_t[\bg_t]} + \frac{\bL\eta_t^2}{2}\Exp_t\left[\norm{\bg_t}^2\right]\\
        &\leq
        f(\bx_t) - \eta_t \norm{\nabla f(\bx_t)}^2 + \eta_t\norm{\nabla f(\bx_t)}\norm{\Exp_t[\bg_t] - \nabla f(\bx_t)}
        +
        \frac{\bL\eta_t^2}{2}\Exp_t\left[\norm{\bg_t}^2 \right]\enspace.
    \end{align*}
    Furthermore, invoking the assumption of the bias and the variance of $\bg_t$ and using the fact that $2ab \leq a^2 + b^2$ we deduce
    \begin{align*}
        \Exp_t[f(\bx_{t+1})]
        &\leq
        f(\bx_t) - \eta_t \norm{\nabla f(\bx_t)}^2 + \eta_tb_t\norm{\nabla f(\bx_t)}
        +
        \frac{\bL\eta_t^2}{2}\parent{v_t + m \norm{\nabla f(\bx_t)}^2}\\
        &\leq
        f(\bx_t) - \eta_t \norm{\nabla f(\bx_t)}^2 + \frac{\eta_t}{2}\parent{b_t^2 + \norm{\nabla f(\bx_t)}^2}
        +
        \frac{\bL\eta_t^2}{2}\parent{v_t + m \norm{\nabla f(\bx_t)}^2}\\
        &=
        f(\bx_t) - \frac{\eta_t}{2}\parent{1 - \bL\eta_tm}\norm{\nabla f(\bx_t)}^2 + \frac{\eta_t}{2}\parent{b_t^2 + \bL\eta_t v_t}\enspace.
    \end{align*}
    Taking total expectation yields the desired claim.

\end{proof}

% Summing up all the inequalities in Lemma~\ref{lem:general} for $t \leq T$ and using the fact that $f(\bx_{T + 1}) \geq f^{\star}$ we arrive at the following corollary.
% \begin{corollary}[Highly smooth functions]\label{HighSF}
%     Let assumptions of Lemma~\ref{lem:general} be fulfilled.
%     Assume that $\eta_t$ in Eq.~\eqref{eq:algo_general} is chosen to satisfy $\bL \eta_t m < 1$ and that $f^{\star} > -\infty$.
%     Let $S$ be a random variable with values in $\{1, \ldots, T\}$, which is independent from $\bx_1, \ldots, \bx_T, \bg_1, \ldots, \bg_T$ and such that
%     \begin{align*}
%         \Prob(S = t) = \frac{\eta_t\parent{1 - \bL\eta_tm}}{\sum_{t = 1}^T\eta_t\parent{1 - \bL\eta_tm}}\enspace.
%     \end{align*}
%     Then, it holds that
%     \begin{align*}
%         \Exp\left[\norm{\nabla f(\bx_S)}^2\right] \leq \frac{2(\Exp[f(\bx_1)] - f^{\star}) + \sum_{t = 1}^T\eta_t\parent{b_t^2 + \bL\eta_t v_t}}{\sum_{t = 1}^T\eta_t\parent{1 - \bL\eta_tm}}\enspace.
%     \end{align*}
% \end{corollary}

\newpage


\newpage
\section{On biases and variances}



Let us first recall the following result, which can be found in~\cite[Section 13.3.5, Exercise 14a]{zorich2016}. It was often used without a reference in the context of zero-order optimization with noisy Oracle~\cite{flaxman2004,BP2016,NY1983}.

\begin{theorem}[Integration by parts in a multiple integral]
\label{thm:ipp}
    Let $D$ be an open connected subset of $\bbR^d$ with a piecewise smooth boundary $\partial D$ oriented by the outward unit normal $\bn = (n_1, \ldots, n_m)^\top$. Let $f$ be a smooth function in $D \cup \partial D$, then
    \begin{align*}
        \int_{D} \nabla f(\bx) \d \bx = \int_{\partial D} f(\bx) \bn(\bx) \d S(\bx)\enspace.
    \end{align*}
\end{theorem}
% \evg[inline]{Added the above result. In Zorich $D$ should be an open set, it seems to me that it is not an issue to replace $D$ by its closure (since $\d\bx$ is the Lebesgue measure). Zorich calls the above formula as: Integration by parts in a multiple integral and not Stokes' theorem.}
\begin{remark}
We refer to~\cite[Section 12.3.2, Definitions 4 and 5]{zorich2016} for the definition of piecewise smooth surfaces and their orientations respectively.
\end{remark}






\subsection{\texorpdfstring{$\ell_2$}{}-randomization}

This section of Appendix is devoted to the analysis of bias and variance of $\ell_2$-randomization algorithm. It is split into two parts, with the first one focused on the bias and the second one focused on the variance.
\subsubsection{Control of the bias}

\begin{lemma}
\label{tru}
Let $f : \mathbb{R}^d \to \mathbb{R}$ be a continuously differentiable function.
% has a directional derivative which belongs to $\mathcal{F}_{\beta-1}$(L), for $\beta \geq 2$.
Let $r, \bU^{\circ}, \bzeta^{\circ}$ be uniformly distributed on $[-1,1], \ball_d^2$, and $\sphere_{d}^2$, respectively. Then, for any $h >0$, we have 
\[
\Exp[\nabla f(\bx+hr\bU^{\circ})rK(r)]=\frac{d}{h}\Exp[f(\bx + hr\bzeta^{\circ})\bzeta^{\circ} K(r)]\enspace.
\]
\end{lemma}
\begin{proof}
Fix $r \in [-1,1] \setminus \{0\}$. Define $\phi:\mathbb{R}^d \to \mathbb{R}$ as $\phi (\bu) = f(\bx + hr\bu) K(r)$ and note that $\nabla \phi(\bu) = hr\nabla f(\bx + hr\bu)K(r)$. Hence, we have
\begin{align*}
    \Exp[\nabla f(\bx+hr\bU^{\circ})K(r) \mid r] = \frac{1}{hr}\Exp[\nabla \phi(\bU^{\circ}) \mid r]
    &=
    \frac{d}{hr}\Exp[\phi(\bzeta^{\circ})\bzeta^{\circ} \mid r]\\
    &=
    \frac{d}{hr}K(r)\Exp[f(\bx+hr\bzeta^{\circ})\bzeta^{\circ} \mid r]\enspace,
\end{align*}
where the second equality is obtained from Theorem~\ref{thm:ipp}. Multiplying by $hr$ from both sides, using the fact that $r$ follows continuous distribution, and taking total expectation concludes the proof.
\end{proof}

\begin{proof}[Proof of Lemma~\ref{lem:bias_sphere}]
Using Lemma~\ref{tru}, the fact that $\int_{-1}^{1} rK(r)\d r = 1$, and the variational representation of the Euclidiean norm, we can write 
\begin{align}
    \label{eq:bias_new1}
    \norm{\Exp[\bg_t^{\circ} \mid \bx_t]-\nabla f(\bx_{t})} = \sup_{\bv \in \sphere_{d}^2}\Exp[\big(\nabla_{\bv} f(\bx+h_tr_t\bU^{\circ}) - \nabla_{\bv}f(\bx)\big)r_tK(r_t)]\enspace,
\end{align}
where we recall that $\bU^{\circ}$ is uniformly distributed on $\ball_d^2$. Lemma~\ref{lem:f_to_grad} asserts that for any $\bv \in \sphere_d^2$ the directional gradient $\nabla_{\bv}f(\cdot)$ is $(\beta-1, L)$-H\"older.
Thus, thanks to Lemma~\ref{lem:holder_to_taylor}, the following Taylor's expansion holds
\begin{align}
    \label{eq:taylor_grad}
    \nabla_{\bv}f(\bx_t+h_tr_t\bU^{\circ}) = \nabla_{\bv} f(\bx_t) +\sum_{1\leq|\bm|\leq \ell -1}\frac{(r_th_t)^{|\bm|}}{\bm!}D^{\bm}\nabla_{\bv}f(\bx_t)({\bU^{\circ}})^{\bm}+R(h_tr_t\bU^{\circ})\enspace,
\end{align}
where the residual term $R(\cdot)$ satisfies $|R(\bx)|\leq \tfrac{L}{(\ell - 1)!} \norm{\bx}^{\beta - 1}$.

Substituting Eq.~\eqref{eq:taylor_grad} into Eq.~\eqref{eq:bias_new1} and using the ``zeroing-out'' properties of the kernel $K$, we deduce that
\begin{align*}
    \norm{\Exp[\bg_t^{\circ} \mid \bx_t]- \nabla f(\bx_{t})}\leq \kappa_{\beta}h_{t}^{\beta-1}\frac{L}{(\ell - 1)!}\Exp\norm{\bU^{\circ}}^{\beta-1} = \kappa_{\beta}h_{t}^{\beta-1} \frac{L}{(\ell - 1)!} \frac{d}{d+\beta-1}\enspace,
\end{align*}
where the last equality is obtained from the fact that $\Exp\norm{\bU^{\circ}}^q = \frac{d}{d+q}$, for any $q \geq0$.
\end{proof}


{
% \color{black} TODO: incorporate in the main body

% \evg[inline]{Arya, I added the bounds we discussed on 11 oct. Doublecheck pls}
% \subsubsection{Control of the variance}
% \begin{theorem}
% \label{thm:conc_sphere}
% Assume that $g : \sphere_d^2 \to \bbR$ is such that $\abs{g(\bu) - g(\bu')} \leq \norm{\bu - \bu'}$ for all $\bu, \bu' \in \sphere_d^2$.
% % \begin{align*}
% %     \Exp\norm{\nabla g(\bzeta^{\diamond})} \leq L
% % \end{align*}
% If $\bzeta^{\circ}$ distributed uniformly on $\sphere_d^2$, then
% \evg[inline]{Should replace $d$ by $d-1$ in the exponent and consequently everywhere else! To take care!}
% \begin{align*}
%     \mathbf{P}\parent{\abs{g(\bzeta^{\circ}) - \med(g)} > t} \leq 2\exp\parent{-\frac{dt^2}{2}}\qquad\forall \,\, t > 0\enspace,
% \end{align*}
% where $\med(g)$ is the median of $g(\bzeta^{\circ})$.
% \end{theorem}


% \begin{proof}[Proof of Lemma~\ref{lem:shamir_like}]
% The proof follows similar lines as that of~\cite[Lemma 9]{Shamir17}.
% Define $g: \sphere_d^2 \to \bbR$ as $ g(\bu) = f(\bx + hr \bu)$ for all $\bu \in \sphere_d^2$. Then, for all $\bu, \bu' \in \sphere_d^2$, by the fact that $f$ is continuously differentiable (note that $f$ is defined on $\bbR^d$, hence $g$ can be extended to $\bbR^d$ in a natural way) and the mean value theorem we obtain for some $\alpha \in (0, 1)$ that
% \begin{align*}
%     |g(\bu) - g(\bu')|
%     =
%     \scalar{\nabla g(\alpha \bu + (1 - \alpha) \bu')}{\bu - \bu'}
%     \leq
%     h \underbrace{\parent{\sup_{\norm{\bv} \leq 1} \norm{\nabla f(\bx + hr \bv)}}}_{=:G(\bx)} \norm{\bu - \bu'}\enspace.
% \end{align*}
% % One can verify that thanks to the fact that $\bzeta^{\circ}$ equals in distribution to $-\bzeta^{\circ}$ it holds that $\med(g) = 0$.
% Thus, using the fact that $\Exp[|X|] = \int_{0}^{\infty}\Prob(|X| > t) \d t$ for all integrable $X$ and applying spherical concentration in Theorem~\ref{thm:conc_sphere} we deduce that
% \begin{align*}
%     \Exp\parent{g(\bzeta^{\circ}) - \med(g)}^2
%     % =
%     % \int_{0}^{\infty}\mathbf{P}\parent{\abs{g(\bzeta^{\circ}) - \med(g)} > t^{\frac{1}{2}}} \d t
%     &\leq 
%     2\int_{0}^{\infty}\exp\parent{-\frac{dt}{2h^2G(\bx)^2}} \d t
%     =
%     \frac{4h^2G(\bx)^2}{d}\enspace.
% \end{align*}
% Finally, since $f \in \mathcal{F}_2(\bar L)$, then it holds that $G(\bx) \leq \bar{L}h + \norm{\nabla f(\bx)}$, which concludes the proof.
% \end{proof}



 


}





% \newpage
\subsection{\texorpdfstring{$\ell_1$}{}-randomization}
% \evg[inline]{This section is finished.}
This part of Appendix is devoted to the analysis of bias and variance of $\ell_2$-randomization algorithm. It is split into two parts, with the first one focused on the bias and the second one focused on the variance.
Let us first introduce additional notation.
\paragraph{Additional notation} We denote by $\Gamma : \bbR_+ \to \bbR_+$ the gamma function defined
\begin{align*}
    \Gamma(z) = \int_{0}^\infty x^{z - 1} \exp(-x) \d x, \qquad z > 0\enspace.
\end{align*}
Given two vectors $\ba = (a_1, \ldots, a_d)^\top, \bb = (b_1, \ldots, b_d)^\top \in \bbR^d$ we denote by $\ba \odot \bb = (a_1b_1, \ldots, a_d b_d)^\top \in \bbR^d$ their Hadamard product. We define the probability simplex on $d$ atoms as
\begin{align*}
    \Delta_{d - 1} = \enscond{\bx \in \bbR^d}{\norm{\bx}_1 = 1,\,\, \bx \geq 0}\enspace,
\end{align*}
where the inequality in the definition of $\Delta_{d-1}$ is component-wise.
% We will additionally need the following fact which we borrowed from \cite[Remark 2.1.1]{fengqi}.
% \begin{lemma}
%     \label{lem:gamma_inequality}
% % [\cite[Remark 2.1.1]{fengqi}]
%     For all $z > 0$ and all $s \in (0, 1]$ it holds that
%     \begin{align*}
%         \frac{\Gamma(z + 1)}{\Gamma(z + s)} \leq (z + s)^{1 - s}\enspace.
%     \end{align*}
% \end{lemma}


Let $\bzeta^{\diamond}$ be distributed uniformly on $\sphere_d^1$. In our analysis we will make use of the following intuitive fact
\begin{align}
    \label{eq:orthant+signs}
    \bzeta^{\diamond} \stackrel{d}{=} \bepsilon \odot \bZ\enspace,
\end{align}
where $\bepsilon$ distributed uniformly on $\{-1, 1\}^d$ and $\bZ$ distributed uniformly on $\Delta_{d-1}$ (note that $\bZ$ follows the Dirichlet distribution with parameter vector $(1, \ldots, 1)$). Intuitively, the above states that in order to sample $\bzeta^{\diamond}$ we can first sample the absolute values of $\bzeta^{\diamond}$ from the probability simplex (realized by $\bZ$) and then select uniformly at random an orthant by $\bepsilon$.

In this section we analyse the gradient estimator considered in Algorithm~\ref{algo:simplex}.
Let $\bepsilon$ be distributed uniformly on $\{-1, 1\}^d$, $\bZ$ be distributed uniformly on $\Delta_{d-1}$, and $r$ be distributed uniformly on $[-1, 1]$. Assume that $\bepsilon$, $\bZ$, and $r$ are independent.
Consider the following gradient estimate at a point $\bx \in \bbR^d$

\begin{align}
    \label{eq:grad_simplex}
    \bg_{\bx, h}^{\diamond} = \frac{d}{2h}\parent{f(\bx + hr\bepsilon \odot \bZ) - f(\bx - hr\bepsilon \odot \bZ) + \zeta}\bepsilon K(r)\enspace,
\end{align}
where $\zeta$ is such that $\Exp[\zeta^2] \leq 2 \sigma^2$ and $\zeta$ is independent from $\bepsilon, Z, r$. Note that the gradient estimator in Eq.~\eqref{eq:grad_simplex} is exactly the one used by Algorithm~\ref{algo:simplex} at time $t = 1, \ldots, T$ with $\zeta = \xi_t - \xi'_t$. 

% \subsubsection{Variance}


\subsubsection{Control of bias}

\begin{lemma}
\label{lem:stokes_l1}
Let $f: \bbR^d \to \bbR$ be continuously differentiable function. Let $\bU^{\diamond}$ be uniformly distributed on $\ball^1_d$ and $\bzeta^{\diamond}$ be uniformly distributed on $\sphere_d^1$, then
\begin{align*}
    \Exp[\nabla f(\bU^{\diamond})] = d \Exp[f(\bzeta^{\diamond})\sign(\bzeta^{\diamond})]\enspace,
\end{align*}
where $\bepsilon$ and $\bZ$ are defined in the beginning of the present section.
\end{lemma}
\begin{proof}
Theorem~\ref{thm:ipp} implies that
\begin{align*}
    \int_{\ball_d^1} \nabla f(\bx) \d \bx = \frac{1}{\sqrt{d}}\int_{\sphere_d^1} f(\bx) \sign(\bx) \d S(\bx)\enspace.
\end{align*}
Furthermore, we recall that
\begin{align*}
    \vol_{d}\parent{\ball_d^1} = \frac{2^d}{d!}\qquad\text{and}\qquad\vol_{d-1}\parent{\sphere_d^1} = \frac{2^d \sqrt{d}}{(d-1)!}\enspace,
\end{align*}
where $\vol_d(\cdot)$ is the Lebesgue volume and $\vol_{d-1}(\cdot)$ denotes the surface area. The above implies the desired result.
% \begin{align*}
%     \Exp[\nabla f(\bV)] = d \Exp[f(\bU)\sign(\bU)]\enspace,
% \end{align*}
% where $\bU$ distributed uniformly on $\enscond{\bx \in \bbR^d}{\norm{\bx}_1 = 1}$. We conclude by observing that $\bU \stackrel{d}{=} \bepsilon \odot \bZ$.
\end{proof}

\begin{corollary}
    \label{cor:simplex_unbiased}
    Consider notation of Lemma~\ref{lem:stokes_l1}.
    Fix some $\bx \in \bbR^d$ and $h > 0$, and let Assumption~\ref{ass1} be fulfilled, then the estimator in Eq.~\eqref{eq:grad_simplex} satisfies
    \begin{align*}
    \Exp[\bg_{\bx, h}^{\diamond}] = \Exp[\nabla f(\bx + hr\bU^{\diamond})rK(r)]\enspace.
    \end{align*}
\end{corollary}
\begin{proof}
The proof is analogous to that of Lemma~\ref{tru}.
\end{proof}

In order to control the bias of the estimator in Eq.~\eqref{eq:grad_simplex}, we need the following result, which controls the moments of the Euclidean norm of $\bU^{\diamond}$.


% \evg[inline]{Here there is a mild inaccuracy. Need to consider the case of $\beta \in [2, 1)$ separately from $\beta > 2$. For $\beta \in [2, 1)$ Jensen's inequality will give the result. To come back!}
\begin{lemma}
\label{lem:moments_l1}
Let $\bU^{\diamond} \in \bbR^d$ be distributed uniformly on $\ball_d^1$, then for any $\beta \geq 2$ it holds that
\begin{align*}
    \Exp \norm{\bU^{\diamond}}^\beta \leq \frac{d^{\frac{\beta}{2}}\Gamma(\beta + 1)\Gamma(d + 1)}{\Gamma(d + \beta + 1)}\enspace.
\end{align*}
\end{lemma}
\begin{proof}
% \evg{I modified here a bit to make it cleaner}
Let $\bW = (W_1, \ldots, W_d), W_{d+1}$ be \iid random variables following Laplace distribution with mean $0$ and scale parameter $1$.
% and $W \sim \exp(1)$ being independent from $U_1, \ldots, U_d$.
Then, following \cite[Theorem 1]{Barthe_Guedon_Mendelson_Naor05} we have
\begin{align*}
    \bU^{\diamond}\stackrel{d}{=} \frac{\bW}{\norm{\bW}_1 + |W_{d+1}|}\enspace,
\end{align*}
where the above equality holds in distribution. Furthermore, \cite[Theorem 2]{Barthe_Guedon_Mendelson_Naor05} (see also~\cite{Rachev_Ruschendorf91,Schechtman_Zinn90}) states that
\begin{align*}
    \frac{(\bW, |W_{d+1}|)}{\norm{\bW}_1 + |W_{d+1}|}\qquad\text{and}\qquad \norm{\bW}_1 + |W_{d+1}|\enspace,
\end{align*}
are independent.
Hence, we can write that $\Exp \norm{\bU^{\diamond}}^\beta$ equals to
\begin{align}
    \label{eq:moment_l1_1}
    \Exp \left[\parent{\frac{\sum_{j = 1}^d W_j^2}{\parent{\norm{\bW}_1 + |W_{d+1}|}^2}}^{\beta / 2}\right]
    % \leq
    % \Exp \left[\frac{\norm{\bW}^{\beta}}{\norm{(\bW, W_{d+1})}_1^{\beta}}\right]
    = \frac{\Exp\norm{\bW}^\beta}{\Exp\norm{(\bW, W_{d+1})}_1^\beta}\enspace,
\end{align}
where the equality follows by the independence recalled above. Note that for any $j = 1, \ldots, d$ it holds that $|W_j|$ is $\exp(1)$ random variable.
Thus, since $\beta \geq 2$, we can write by Jensen's inequality
\begin{align}
\label{eq:moment_l1_2}
    \Exp\norm{\bW}^\beta = d^{\frac{\beta}{2}}\Exp\parent{\frac{1}{d}\sum_{j  = 1}^d W_j^2}^{\beta / 2} \leq d^{\frac{\beta}{2} - 1} \sum_{j = 1}^d \Exp[W_j^\beta] = d^{\frac{\beta}{2}} \Exp[W_1^\beta] = d^{\frac{\beta}{2}} \Gamma(\beta + 1)\enspace.
\end{align}
It remains to provide a suitable expression (or lower bound) for $\Exp\norm{(\bW, W_{d+1})}_1^\beta$. We observe that $\norm{(\bW, W_{d+1})}_1$ follows Erlang distribution with parameters $(d+1, 1)$ (as a sum of $d+1$ \iid $\exp(1)$ random variables).
Hence, recalling the expression for the density of the Erlang distribution
\begin{align}
\label{eq:moment_l1_3}
    \Exp\norm{(\bW, W_{d+1})}_1^\beta = \frac{1}{\Gamma(d+1)}\int_{0}^{\infty}x^{d + \beta}\exp(-x) \d x =  \frac{\Gamma(d + \beta + 1)}{\Gamma(d + 1)}\enspace.
\end{align}
Substituting Eqs.~\eqref{eq:moment_l1_2}--\eqref{eq:moment_l1_3} into Eq.~\eqref{eq:moment_l1_1} we conclude.
\end{proof}


We are in position to derive an upper bound on the bias of the gradient estimator in Eq.~\eqref{eq:grad_simplex}.

\begin{proof}[Proof of Lemma~\ref{lem:bias_l1}]
Invoking Corollary~\ref{cor:simplex_unbiased} and following the same lines as in the proof of Lemma~\ref{lem:bias_sphere}, we deduce that
% \evg{here also modified accordingly.}
\begin{align*}
    \norm{\Exp[\bg_t^{\diamond} \mid \bx_t]- \nabla f(\bx_{t})}
    \leq
    \kappa_{\beta}h_{t}^{\beta-1} \frac{L}{(\ell - 1)!}\Exp \norm{\bU^{\diamond}}^{\beta-1}
    \leq
    \kappa_{\beta}h_{t}^{\beta-1} \frac{L}{(\ell - 1)!}\frac{d^{\frac{\beta - 1}{2}}\Gamma(\beta)\Gamma(d + 1)}{\Gamma(d + \beta)}\enspace,
\end{align*}
where the last inequality is thanks to Lemma~\ref{lem:moments_l1}. {
% \color{black}
Recall the following property of Gamma function: for any $z>0$ we have $\Gamma(z+1) = z\Gamma(z)$. Therefore, applying this property iteratively and recalling the definition of $\ell$, we deduce that
\begin{align*}
    \frac{\Gamma(d + 1)}{\Gamma(d+\beta)}
    &= \frac{\Gamma(d+1)}{\Gamma\big(d+\underbrace{(\beta-\ell)}_{\in (0, 1]}\big)\prod_{i = 1}^{\ell}\big(d+\beta-i\big) }
    \leq
    \frac{(d + \beta - \ell)^{1 - (\beta -\ell)}}{\prod_{i = 1}^{\ell}\big(d+\beta-i\big) }
    % \leq
    % \frac{(d + \beta - \ell)^{\beta - \ell}}{\prod_{i = 1}^{\ell - 1}\big(d+\beta-i\big) }
    % \frac{\Gamma(d+1)}{d^{\ell}\Gamma\big(d+\underbrace{\beta-\ell}_{\in (0, 1]}\big)}
    \leq \frac{1}{d^{\beta-1}}\enspace,
\end{align*}
where the first inequality is obtained from \cite[Remark 2.1.1]{fengqi}. Finally, for the term $\frac{\Gamma(\beta)}{(\ell-1)!}$, we can write
\begin{align*}
    \frac{\Gamma(\beta)}{(\ell-1)!} = \frac{\Gamma(\beta)}{\Gamma(\ell)}= \frac{\ell \Gamma(\ell + (\beta-\ell))}{\Gamma(\ell+1)}\leq \ell^{\beta-\ell} \leq \ell\enspace,
\end{align*}
where we again used \cite[Remark 2.1.1]{fengqi} for the first inequality. Combining the above derived bounds we conclude.
% \begin{align*}
%     \norm{\Exp[\bg_t \mid \bx_t]- \nabla f(\bx_{t})}\leq \kappa_{\beta}h_{t}^{\beta-1} \ell{L} d^{\frac{1-\beta }{2}}\enspace.
% \end{align*}
}
\end{proof}



{
\subsubsection{Control of variance}
% \color{black}
% \evg[inline]{Better variance for $\ell_1$}


\begin{proof}[Proof of Lemma~\ref{lem:Poincare_like}]
% The proof is largely inspired by~\citep[Lemma 3, Theorem 5, Proposition 9]{barthe2009remarks}.
Let $\bW = \left(W_1, \dots, W_d\right)$ be i.i.d. zero mean unit variance Laplace random variables and define $\bT(\bw) = \bw / \norm{\bw}_1$ with the sgreement that $0/0 = 0$.
Poincaré inequality for the exponential measure~\cite[see, for instance][]{talagrand1991new,bobkov1997poincare} states that for any continuously differentiable function $F:\mathbb{R}^d\to \mathbb{R}$ with $\Exp [F(\bW)] = 0$
\begin{align}\label{PoinInq}
    \Exp\left[F^2(\bW)\right]\leq 4\Exp\norm{\nabla F(\bW)}^2\enspace. 
\end{align}
Lemma~1 of~\cite{Schechtman_Zinn90} stated that
\begin{align}
    \label{eq:SZ90}
    \bT(\bW) \stackrel{d}{=} \bzeta^{\diamond}\qquad\text{and}\qquad \bT(\bW), \bW \text{ are independent}\enspace.
\end{align}
We would like to apply the above inequality for $G' \equiv G \circ \bT$, but $G'$ is not continuously differentiable. Instead, we proceed by the standard approximation argument then pass to the limit by dominated convergence theorem.

\paragraph{Approximation.}
Fix some $\epsilon>0$ and consider $\bT_{\epsilon} (\bw)= \frac{\bx}{h_{\epsilon}(\bw)}$, where $h_{\epsilon}:\mathbb{R}^d\to\mathbb{R}$ is defined as 
\begin{equation*}
   h_{\epsilon}(\bw) = \sum_{i = 1}^d\begin{cases}
      \frac{1}{2\epsilon}w^2_i + \epsilon & \text{if  $|w_i|< \epsilon$}\\
      |w_i| + \frac{\epsilon}{2} & \text{if  $|w_i| \geq \epsilon$}
    \end{cases}\enspace,
\end{equation*}
for any $\bw \in \mathbb{R}^d$.
For all $\epsilon > 0$, the introduced $\bT_{\epsilon} : \bbR^d \to \bbR^d$, is continuously differentiable and for all $\bw \in \bbR^d$ we have $h_{\epsilon}(\bw) \geq \norm{\bw}_1$ leading to
\begin{align}
    \label{eq:bounded_T}
    \norm{\bT_{\epsilon}(\bx)} \leq \frac{\norm{\bw}}{\norm{\bw}_1} \leq 1 \qquad\forall \bw \in \bbR^d\enspace.
\end{align}
Set $G'_{\epsilon} \equiv G\circ \bT_{\epsilon}$, and note that $G_{\epsilon}$ is continuously differentiable for all $\epsilon > 0$, hence since $\Exp[G_{\epsilon}'(\bW) - G_{\epsilon}'(-\bW)] = 0$, we apply Eq.~\eqref{PoinInq} to deduce
\begin{align}
    \label{eq:poincare_like1}
    \Exp\left(G'_{\epsilon}\left(\bW\right)-G'_{\epsilon}\left(-\bW\right)\right)^2
    \leq
    4\Exp\left[\norm{\nabla G'_{\epsilon}(\bW) + \nabla G'_{\epsilon}(-\bW)}^2\norm{\jac_{\bT_{\epsilon}}\left(\bW\right)}^2\right]\enspace,
\end{align}
where $\jac_{\bT_{\epsilon}}(\bw)$ is the Jacobi matrix of $\bT_{\epsilon}(\bw)$ and $\norm{\jac_{\bT_{\epsilon}}\left(\bw\right)}$ is its operator norm (as an operator from $(\bbR^d, \norm{\cdot})$ to itself).
Let us provide a bound on this norm, which follows similar reasoning as in~\cite[Lemma 2]{barthe2009remarks}. For any $\bw = (w_1, \ldots, w_d)^\top \in \mathbb{R}^d$ and $j \neq i$, we have
\begin{align*}
    \frac{\partial \left(\bT_{\epsilon}\right)_i}{\partial w_j} (\bw)
    &=
    \frac{\partial}{\partial w_j}\left(\frac{w_i}{h_{\epsilon}(\bw)}\right)
    =
    -\frac{w_i\left(\frac{w_j}{\epsilon}\ind{|w_j|<\epsilon}+\sign(w_j)\ind{|w_j|\geq\epsilon}\right)}{h^2_{\epsilon}(\bw)}\enspace,
\end{align*}
and for each $i = 1, \ldots, d$, we can write
\begin{align*}
    \frac{\partial \left(\bT_{\epsilon}\right)_i}{\partial w_i} \left(\bw\right)
    &=\frac{\partial}{\partial w_i}\left(\frac{w_i}{h_{\epsilon}(\bw)}\right)
    = \frac{1}{h_{\epsilon}(\bw)}\parent{1-\frac{w_i\left(\frac{w_i}{\epsilon}\ind{|w_i|<\epsilon}+\sign(w_i)\ind{|w_j|\geq\epsilon}\right)}{h_{\epsilon}(\bw)}}\enspace.
\end{align*}
Let $\bA_{\epsilon}(\bw) \in \mathbb{R}^d$ be defined component-wise as $\left(\textbf{A}_{\epsilon}(\bw)\right)_{i} = \sign(w_i)\ind{|w_i|\geq \epsilon}$ and  $\bB_{\epsilon}(\bw) \in \mathbb{R}^d$ as $\left(\bB_{\epsilon}(\bw)\right)_{i} = \frac{w_i}{\epsilon}\ind{|w_i|< \epsilon}$ for $1 \leq i \leq d$. In this notation, the Jacobi matrix can be expressed as
\begin{align*}
    \jac_{\bT_{\epsilon}}(\bw) = \frac{1}{h_{\epsilon}(\bw)}\left(\bfI - \bT_{\epsilon}(\bw) \bA^{\top}_{\epsilon}(\bw)  - \frac{\bw \bB_{\epsilon}^{\top}(\bw) }{h_{\epsilon}(\bw)}\right)\enspace,
\end{align*}
where $\bfI$ is the identity matrix.
Since, $\norm{\ba' \ba^{\top}} \leq \norm{\ba'} \cdot \norm{\ba}$ for all $\ba, \ba' \in \bbR^d$, then
\begin{align*}
    \norm{\jac_{\bT_{\epsilon}}(\bw)}\leq \frac{1}{h_{\epsilon}(\bw)}\left(1 + \sqrt{d}\norm{\bT_{\epsilon}(\bw)} + R_{\epsilon}(\bw)\right)\enspace,
\end{align*}
where we introduced $R_{\epsilon}(\bw) = \tfrac{\norm{\bw}\sqrt{\sum_{k = 1}^d 1_{|w_i| < \epsilon}}}{h_{\epsilon}(\bw)}$.
Thus, in view of the above bound and Eq.~\eqref{eq:poincare_like1} for any $\epsilon > 0$
\begin{small}
\begin{align}
    \label{eq:dominated}
    \underbrace{\Exp\left(G'_{\epsilon}\left(\bW\right)-G'_{\epsilon}\left({-}\bW\right)\right)^2}_{\text{left hand side}}
    {\leq}
    4\underbrace{\Exp\left[\frac{\norm{\nabla G(\bT_{\epsilon}(\bW)) + \nabla G(\bT_{\epsilon}({-}\bW))}^2}{h_{\epsilon}^2(\bW)}\left(1 {+} \sqrt{d}\norm{\bT_{\epsilon}(\bW)} {+} R_{\epsilon}(\bW)\right)^2\right]}_{\text{right hand side}}\,.
\end{align}
\end{small}
Our goal is to take the limit on both sides of the above inequality and exchange this limit with the integration. To do so, we will utilize the dominated convergence theorem for both left and right hand sides which will lead to
\begin{small}
\begin{align}
    \label{eq:dominated1}
    {\Exp\left(G'\left(\bW\right){-}G'\left(-\bW\right)\right)^2} \leq 4{\Exp\left[{\norm{\nabla G(\bT(\bW)) + \nabla G(\bT(-\bW))}^2}\frac{\left(1 {+} \sqrt{d}\norm{\bT(\bW)}\right)^2}{\norm{\bW}_1^2}\right]}\enspace,
\end{align}
\end{small}
and the statement of the lemma follows by application of~\cite[Lemma 1]{Schechtman_Zinn90} recalled in Eq.~\eqref{eq:SZ90}, and $\Exp\norm{\bW}_1^{-2} = 1 / ((d-1)(d-2))$ for all $d\geq 3$ (since $\norm{\bW}_1$ follows Erlang distribution with parameters $(d, 1)$).

The rest of the proof is devoted to the justification of the limiting argument and, in particular, to checking conditions of dominated convergence theorem.
In what follows $B > 0$ will denote a generic constant which can differ from line to line (for the limiting argument we do not care about its value).

\paragraph{Left hand side of Eq.~\eqref{eq:dominated}.}
Note that for all $\bw \in \bbR^d \setminus \{0\}$ we have
\begin{align*}
    \left(G'_{\epsilon}\left(\bw\right)-G'_{\epsilon}\left(-\bw\right) \right)^2 \longrightarrow \left(G'\left(\bw\right)-G'\left(-\bw\right) \right)^2 \qquad \text{as} \qquad \epsilon \rightarrow 0\enspace.
\end{align*}
By the assumption, $G$ is continuously differential and by Eq.~\eqref{eq:bounded_T}  we have $\norm{\bT_{\epsilon}(\bw)} \leq 1$, then there exists $B > 0$ such that for all $\bw \in \bbR^d$
\begin{align*}
    |G'_{\epsilon}\left(\bw\right)-G'_{\epsilon}\left(-\bw\right)| = |G\left(\bT_{\epsilon}(\bw)\right)-G\left(\bT_{\epsilon}(-\bw)\right)| \leq B\norm{\bT_{\epsilon}(\bw) - \bT_{\epsilon}(-\bw)} \leq 2B\enspace.
\end{align*}
% Thus, we have taken care of the left hand side by dominant convergence theorem. 

\paragraph{Right hand side of Eq.~\eqref{eq:dominated}.}
Since $G$ is assumed to be continuously differentiable and $\norm{\bT_{\epsilon}(\bw)} \leq 1$ on $\bbR^d$, then $\norm{\nabla G(\bT_{\epsilon}(\bw)) + \nabla G(\bT_{\epsilon}(-\bw))}^2 \leq B$ for some $B > 0$. Furthermore, by continuity of $\nabla G$, we have for all $\bw \in \bbR^d \setminus \{0\}$
\[
\norm{\nabla G(\bT_{\epsilon}(\bw)) + \nabla G(\bT_{\epsilon}(-\bw))}^2 \longrightarrow \norm{\nabla G(\bT(\bw)) + \nabla G(\bT(-\bw))}^2 \qquad\text{as}\qquad \epsilon \rightarrow 0\enspace.
\] 
Finally, for any $\bw$ such that $w_i \neq 0$ for all $i = 1, \ldots, d$ (\ie almost everywhere \wrt the distribution of $\bW$) we have
\begin{align*}
    \frac{1}{h^2_{\epsilon}(\bw)}\left(1 + \sqrt{d}\norm{\bT_{\epsilon}(\bw)} + R_{\epsilon}(\bw)\right)^2 \longrightarrow \frac{1}{\norm{\bw}_1}\left(1 + \sqrt{d}\norm{\bT(\bw)}\right) \qquad \text{as} \qquad \epsilon \rightarrow 0\enspace,
\end{align*}
and, recalling that $h_{\epsilon}(\bw) \geq \norm{\bw}_1$ and the expression for $R_{\epsilon}(\cdot)$, the following  bound holds
\begin{align*}
    \frac{1}{h^2_{\epsilon}(\bw)}\left(1 + \sqrt{d}\norm{\bT_{\epsilon}(\bw)} + R_{\epsilon}(\bw)\right)^2 \leq \frac{1}{\norm{\bw}_{1}^2}\left(1+2\sqrt{d}\right)^2\enspace.
\end{align*}
% with $\jac_{T}(\bx)$ as the Jacobi matrix of $T(\bx)$. Furthermore, by letting \begin{align*}
%     H_{\epsilon}(\bx) = \frac{1}{\sum_{k=1}^{d}\left(|x_k|_\epsilon +\epsilon\right)}\left(1 + \sqrt{d}\norm{\bT_{\epsilon}(\bx)} + \frac{\norm{\bx}\sqrt{\sum_{k = 1}^d 1_{|x_i| < \epsilon}}}{\sum_{k=1}^{d}\left(|x_k|_\epsilon +\epsilon\right)}\right),
% \end{align*}
% and 
% \begin{align*}
%     H(\bx) = \frac{1}{\norm{\bx}_1}\left(1 + \sqrt{d}\norm{\bT(\bx)}\right),
% \end{align*}
% we have $H_{\epsilon}(\bx) \to H_{\bx}$ as $\epsilon \to 0$, for all $\bx \in \mathbb{R}^d$ except a set of zero Lebesgue measure (more formally, everywhere except the set $\{\bx \in \bbR^d \,:\, \exists\,\, i = 1, \ldots, d \text{ s.t. } x_i = 0\}$). Also, by the definition of Huber function, we can see 
% $$\sum_{k=1}^{d}\left(|x_{k}|_{\epsilon}+\epsilon\right) \geq \norm{\bx}_{1}.$$ Thus,
% \begin{align*}
%     H_{\epsilon}(\bx) 
%     &\leq \frac{1}{\norm{\bx}_{1}}\left(1+\frac{\sqrt{d}\norm{\bx}}{\norm{\bx}_{1}} + \frac{\norm{\bx}\sqrt{\sum_{k = 1}^d 1_{|x_i| < \epsilon}}}{\norm{\bx}_{1}}\right)
%     \leq
%     \frac{1}{\norm{\bx}_{1}}\parent{\left(1+2\sqrt{d}\right)}\enspace.
% \end{align*}
% and thus
% \begin{align*}
%     H^2_{\epsilon}\left(\bW\right) \leq \frac{1}{\norm{\bx}_{1}^2}\left(1+2\sqrt{d}\right)^2\enspace.
% \end{align*}
For all $d \geq 3$ the function on the right hand side of the above inequality is integrable against the exponential measure (the distribution of $\bW$).


Taking $\epsilon = 1/n$ and applying the dominated convergence theorem to both sides of Eq.~\eqref{eq:dominated} we deduce Eq.~\eqref{eq:dominated1} and conclude.
\end{proof}




\begin{lemma}
\label{lem:moments_of_strange_things}
For all $d \geq 3$ it holds that
\begin{align*}
    &\Exp\left[{(1 + \sqrt{d}\norm{\bzeta^{\diamond}})^2}\right] \leq {\parent{1 + \sqrt{\frac{2d}{d+1}}}^2}\enspace,\\
    &\Exp\left[{(1 + \sqrt{d}\norm{\bzeta^{\diamond}})^2\norm{\bzeta^{\diamond}}^2}\right] \leq
    \frac{2}{(d+1)}\parent{3 + \sqrt{{8 + \frac{592}{(d+3)^2}}} + \frac{22}{d}}
    % \frac{12+\frac{88}{d}}{(d-1)(d-2)(d+1)}\enspace.
\end{align*}

\end{lemma}
\begin{proof}
% We start the proof with some preparations.
% Lemma 1 of~\cite{Schechtman_Zinn90} states that $\bT(\bW)$ and $\bW$ are indepedent and that $\bT(\bW) \stackrel{d}{=} \bzeta^{\diamond}$. Thus, for any $H_0, H_1 : \bbR \to \bbR$ we have
% \begin{align}
%     \label{eq:strange_moment1}
%     \Exp[H_0(\bT(\bW))H_1(\bW)] = \Exp[H_0(\bzeta^{\diamond})]\Exp[H_1(\bW)] \enspace.
% \end{align}
% Also, since $\norm{\bW}_1$ follows Erlang distribution with parameters $(d, 1)$, then if $d \geq 3$
%     \begin{align}
%         \label{eq:var_l1_v3_intermediate3}
%         \Exp\left[\frac{1}{\norm{\bW}_1^2}\right] = \frac{1}{(d - 1)(d-2)}\enspace.
%     \end{align}
In what follows we will make use of the following expression for the moments of Dirichlet distribution
\begin{align}
    \label{eq:moments_dirichlet}
    \Exp[(\bzeta^{\diamond})^{\bm}] = \frac{\Gamma(d)}{\Gamma(d + |\bm|)}\prod_{i = 1}^d\Gamma(m_i + 1) = \frac{(d-1)!\bm!}{(d - 1 + |\bm|)!}\enspace,
\end{align}
for any multi-index $\bm = (m_1, \ldots, m_d) \in \bbN^d$ with even coordinates.

    
\paragraph{First bound.}
The expression for second moments of Dirichlet distribution in Eq.~\eqref{eq:moments_dirichlet} yields
    \begin{align*}
        \Exp[(1 + \sqrt{d}\norm{\bzeta^{\diamond}})^2] \leq 1 + 2\sqrt{d\Exp\norm{\bzeta^{\diamond}}^2 }+ d\Exp\norm{\bzeta^{\diamond}}^2 \leq 1 + 2\sqrt{\frac{2d}{d+1}} + \frac{2d}{d+1} = \parent{1 + \sqrt{\frac{2d}{d+1}}}^2\enspace.
    \end{align*}
    % where, to evaluate $\|\bzeta^{\diamond}\|^2$, we . 
    % In view of Eq.~\eqref{eq:strange_moment1} and Eq.~\eqref{eq:var_l1_v3_intermediate3},
    The proof of the first claimed bound is concluded.
    % \begin{align*}
    %     \Exp\left[\frac{(1 + \sqrt{d}\norm{\bT(\bW)})^2}{\norm{\bW}_1^2}\right]
    %     % =
    %     % \Exp\left[\frac{1}{\norm{\bW}_1^2}\right]\Exp[(1 + \sqrt{d}\norm{\bzeta^{\diamond}})^2]
    %     \leq
    %     \frac{\parent{1 + \sqrt{\frac{2d}{d+1}}}^2}{(d-1)(d-2)}\enspace.
    %     % = \frac{(\sqrt{d+1} + \sqrt{2d})^2}{(d-1)(d-2)(d+1)}\enspace.
    % \end{align*}
    
    
\paragraph{Second bound.}

 We repeat similar argument for $\Exp[(1 + \sqrt{d}\norm{\bzeta^{\diamond}})^2\norm{\bzeta^{\diamond}}^2]$. By Jensen's inequality, it holds that
    \begin{align*}
        \Exp[(1 + \sqrt{d}\norm{\bzeta^{\diamond}})^2\norm{\bzeta^{\diamond}}^2]
        &\leq
        \Exp\norm{\bzeta^{\diamond}}^2 +
        2\sqrt{d\Exp\norm{\bzeta^{\diamond}}^6} +
        d\Exp\norm{\bzeta^{\diamond}}^4\enspace.\\
        % &\leq
        % \frac{2}{d+1} + 2\sqrt{d\Exp\norm{\bzeta^{\diamond}}^6} + d\Exp\norm{\bzeta^{\diamond}}^4\enspace,
        % &=
        % \frac{2}{d(d+1)} + 2\sqrt{d}\sqrt{\frac{3!(d-1)!}{(d+2)!}\binom{d+2}{d-1}} + d!\sum_{i, j}^3\frac{(2i-1)!(2j-1)!}{(d + 2i + 2j - 1)!}
    \end{align*}
    % where we again used the fact that $\Exp\norm{\bzeta^{\diamond}}^2 = 2/(d + 1)$.
    We already know that $\Exp\norm{\bzeta^{\diamond}}^2 = 2/(d + 1)$ and
    it remains to evaluate $\Exp\norm{\bzeta^{\diamond}}^6$ and  $\Exp\norm{\bzeta^{\diamond}}^4$.
    Using multinomial identity and the expression for the moments in Eq.~\eqref{eq:moments_dirichlet}, we deduce
    \begin{align*}
        \Exp\norm{\bzeta^{\diamond}}^6 = \sum_{|\bm|=3}\frac{6}{\bm!}\Exp[(\bzeta^{\diamond})^{2\bm}] = \sum_{|\bm|=3}\frac{6}{\bm!}\cdot \frac{(d-1)!(2\bm)!}{(d+5)!} = 6\frac{(d-1)!}{(d+5)!} \sum_{|\bm| = 3} \frac{(2\bm)!}{\bm!}\enspace,
    \end{align*}
    and
    \begin{align*}
        \Exp\norm{\bzeta^{\diamond}}^4 = \sum_{|\bm|=2}\frac{2}{\bm!}\Exp[(\bzeta^{\diamond})^{2\bm}] = \sum_{|\bm|=3}\frac{2}{\bm!}\cdot \frac{(d-1)!(2\bm)!}{(d+3)!} = 2\frac{(d-1)!}{(d+3)!} \sum_{|\bm| = 2} \frac{(2\bm)!}{\bm!}\enspace.
    \end{align*}
  Direct calculations show that
% $\sum_{|\bm| = 2} \frac{(2\bm)!}{\bm!} = 2d(d + 11)$.
    \begin{align*}
        &\sum_{|\bm| = 3} \frac{(2\bm)!}{\bm!} = \frac{4}{3}d((d + 3)^2 + 74)\qquad\text{and}\qquad
        \sum_{|\bm| = 2} \frac{(2\bm)!}{\bm!} = 2d(d + 11)\enspace.
    \end{align*}
    Thus, after some basic algebraic simplifications, we get the following expressions for all $d \geq 1$
    \begin{align*}
        &\Exp\norm{\bzeta^{\diamond}}^6 = \frac{8d!(d+3)^2}{(d+5)!}\parent{1 + \frac{74}{(d+3)^2}}\qquad\text{and}\qquad
        % \leq \frac{8d!(d+3)^2}{(d+5)!}\parent{1 + \frac{74}{36}}\enspace,\\
        \Exp\norm{\bzeta^{\diamond}}^4 = \frac{4d!d}{(d+3)!} \parent{1 + \frac{11}{d}}\enspace.
    \end{align*}
    Therefore, we have the following upper bound
    \begin{equation*}
        % \label{eq:starnge_moments2}
    \begin{aligned}
        \Exp[(1 + \sqrt{d}\norm{\bzeta^{\diamond}})^2\norm{\bzeta^{\diamond}}^2]
        &\leq
        % \frac{4}{d + 1} + \frac{8d!d}{(d+3)!}\parent{1 + \frac{11}{d}}
        % \leq
        % \frac{4}{d+1}\parent{3 + \frac{22}{d}}\enspace.
        \Exp[\norm{\bzeta^{\diamond}}^2] + 2\sqrt{d\Exp\norm{\bzeta^{\diamond}}^6} + d\Exp\norm{\bzeta^{\diamond}}^4\\
        % &=
        % \frac{2}{d+1} + 2\sqrt{8\frac{d!d}{(d+4)!}((d+3)^2 + 74)} + \frac{4d!d^2}{(d+3)!}\parent{1 + \frac{11}{d}}\\
        &=
        \frac{2}{d+1} + 2\sqrt{\frac{8d!d(d+3)^2}{(d+5)!}\parent{1 + \frac{74}{(d+3)^2}}} + \frac{4d!d^2}{(d+3)!} \parent{1 + \frac{11}{d}}\\
        &\leq
        \frac{2}{d+1} + 2\sqrt{\frac{8}{(d+1)^2}\parent{1 + \frac{74}{(d+3)^2}}} + \frac{4}{d + 1} \parent{1 + \frac{11}{d}}\\
        &=
        \frac{2}{d+1}\parent{1 + \sqrt{\parent{8 + \frac{592}{(d+3)^2}}} +  \parent{2 + \frac{22}{d}}}\enspace.
        % &\leq
        % \frac{2}{d+1} + 2\sqrt{\frac{8}{(d+1)^2}\parent{1 + \frac{74}{36}}} + \frac{4}{d + 1} \parent{1 + \frac{11}{3}}\\
        % &\leq
        % \frac{2}{d+1}\underbrace{\parent{1 + \sqrt{8 + 592/36} + 2 + 22/3}}_{\leq 15.28}\enspace,
        % &=
        % \frac{2}{d(d+1)} + 2\sqrt{d}\sqrt{\frac{3!(d-1)!}{(d+2)!}\binom{d+2}{d-1}} + d!\sum_{i, j}^3\frac{(2i-1)!(2j-1)!}{(d + 2i + 2j - 1)!}
    \end{aligned}
    \end{equation*}
    % where in the last inequality we used the assumption that $d \geq 3$.
    % Note that the above constant is rather large, however, asymptotically, the leading constant is much smaller ($1 + \sqrt{8} + 2 \leq 5.83$), since the terms $592/(d+3)^2$ and $22/d$ are negligible.
    The proof of the second claimed bound is concluded.
\end{proof}


}








% We compliment the bound on the bias by a bound on the variance of the estimator in Eq.~\eqref{eq:grad_simplex}.

% \begin{proof}[Proof of Lemma~\ref{lem:var_l1}]
%     For simplicity, we drop the index $t$ for $\bx_t, h_t, t_t, \bepsilon_t$, $\bZ_t$ and set $\zeta = \xi_t - \xi_t'$.
%     The proof follows similar arguments developed by~\cite{akhavan2020}, yet the exact computations are different due to the different choice of randomization.
%     Fix some $\bx \in \bbR^d$ and $h > 0$. Using Eq.~\eqref{eq:orthant+signs} and Eq.~\eqref{eq:grad_simplex} we can write
%     \begin{align}
%         \label{eq:var_l1:1}
%         \Exp\|\bg_{t}^{\diamond}\|^2 
%         &=
%         \frac{d^3}{4h^2}\Exp[\parent{f(\bx + hr\bepsilon \odot \bZ) - f(\bx - hr\bepsilon \odot \bZ) + \zeta}^2K^2(r)]
%         % \\
%         % &\leq
%         % \frac{d^3}{2h^2}\Exp\left[\parent{f(\bx + hr\bepsilon \odot \bZ) - f(\bx - hr\bepsilon \odot \bZ)}^2K^2(r) +  2\sigma^2\int_{-1}^1K^2(r)\d r\right]\enspace.
%     \end{align}
%     Let us introduce the following shorthand notation
%     \begin{align*}
%         &R_1 = f(\bx + hr\bepsilon \odot \bZ) - f(\bx) - hr\scalar{\nabla f(\bx)}{\bepsilon \odot \bZ}\enspace,\\
%         &R_2 = - f(\bx - hr\bepsilon \odot \bZ) + f(\bx) - hr\scalar{\nabla f(\bx)}{\bepsilon \odot \bZ}\enspace,\\
%         &R_3 = 2hr\scalar{\nabla f(\bx)}{\bepsilon \odot \bZ}\enspace.
%     \end{align*}
%     Using the above and starting from Eq.~\eqref{eq:var_l1:1} we deduce that
%     \begin{align*}
%         \Exp\|\bg_{t}^{\diamond}\|^2 
%         &=
%         \frac{d^3}{4h^2}\Exp[\parent{R_1 + R_2 + R_3 + \zeta}^2K^2(r)]
%         \leq
%         \frac{d^3}{h^2}\Exp\left[\parent{R_1^2 + R_2^2 + R_3^2 + \zeta^2}K^2(r)\right]\enspace.
%     \end{align*}
%     Furthermore, since $f \in \mathcal{F}_2(\bar{L})$ we deduce that
%     \begin{align*}
%         R_1^2 + R_2^2 \leq \bar{L}^2h^4r^4 \norm{\bZ}^4\enspace.
%     \end{align*}
%     Thus, we have shown that
%     \begin{align}
%         \label{eq:var_l1_2}
%         \Exp\|\bg_{t}^{\diamond}\|^2  \leq  \frac{d^3}{h^2}\Exp\left[\parent{\bar{L}^2h^4\kappa \norm{\bZ}^4 + 4h^2\kappa\scalar{\nabla f(\bx)}{\bepsilon \odot \bZ}^2 + 2\sigma^2\kappa}\right]
%     \end{align}
%      where we recall that $\kappa = \int_{-1}^1  K^{2}(r) \d r$.
%     % Hence, it holds that
%     % \begin{align*}
%     %     \Exp \parent{f(\bx + hr\bepsilon \odot \bZ) - f(\bx - hr\bepsilon \odot \bZ)}^2K^2(r) \leq 3h^4\bar{L}\kappa_{4, 2} \Exp \norm{\bZ}^4 + 12 h^2 \kappa_{2, 2} \Exp\scalar{\nabla f(\bx)}{\bepsilon \odot \bZ}^2\enspace,
%     % \end{align*}
%     Using the independence of $\bepsilon = (\epsilon_1, \ldots, \epsilon_d)^\top$ and $\bZ = (Z_1, \ldots, Z_d)^\top$ and the fact that $\bepsilon$ is an \iid Rademacher vector, we can write for the second term
%     \begin{equation}
%     \label{eq:var_l1_3}
%     \begin{aligned}
%         \Exp\scalar{\nabla f(\bx)}{\bepsilon \odot \bZ}^2
%         &=
%         \Exp\parent{\sum_{i, j = 1}^d \parent{\nabla f(\bx)}_i\parent{\nabla f(\bx)}_j\epsilon_i\epsilon_j Z_iZ_j}\\
%         &=
%         \sum_{j = 1}^d \parent{\nabla f(\bx)}_j^2 \Exp[Z_j^2]
%         % \Exp\scalar{\nabla f(\bx) \odot \bZ}{\bepsilon}^2 = \Exp\norm{\nabla f(\bx) \odot \bZ}^2\\
%         % &= \Exp\scalar{\nabla f(\bx)}{\bZ}^2
%         = \frac{2}{d(d+1)}\norm{\nabla f(\bx)}^2\enspace,
%     \end{aligned}
%     \end{equation}
%     where for the last equality we used the expression for the second moment of Dirichlet distribution.
%     % where the second equality is due to the fact that $$
%     % Furthermore, (again utilizing Theorem 2 in~\cite{Barthe_Guedon_Mendelson_Naor05} and following similar arguments as in the proof of Lemma~\ref{lem:moments_l1}), we have
%     % \begin{align}
%     %     \label{eq:var_l1_Z4}
%     %     \Exp\norm{\bZ}^4 \leq \frac{4! d^2 (d - 1)!}{(d + 3)!} =  \frac{24d}{(d+1)(d+2)(d+3)}\enspace.
%     % \end{align}
%     {
%     % \color{black}
%     We recall the following property of $\bZ = (Z_1, \ldots, Z_d)^\top$:
% \begin{align*}
%     \Exp[Z_j^4] = \frac{24(d-1)!}{(d+3)!}\qquad\text{and}\qquad \Exp[Z_j^2Z_i^2] = \frac{4(d-1)!}{(d+3)!}\qquad i\neq j\enspace.
% \end{align*}
%     Using the above expressions for moments, we deduce that
%     \begin{align}
%     \label{eq:var_l1_Z4}
%         \Exp\norm{\bZ}^4
%         &=
%         \sum_{i,j = 1}^d \Exp[Z_i^2Z_j^2]
%         =
%         \frac{(d-1)!}{(d+3)!}\parent{22 d + 2d^2}
%         \leq
%         % \frac{24}{(d+1)(d+2)(d+3)} + \frac{4(d-1)}{(d+1)(d+2)(d+3)}\\
%         % &\leq
%         \frac{2}{d^2}\parent{\frac{11}{d} + 1}\enspace.
%     \end{align}
%      Combining Eq.~\eqref{eq:var_l1_2} with Eqs.~\eqref{eq:var_l1_3}--\eqref{eq:var_l1_Z4} we deduce the desired result:
%     \begin{align*}
%         \Exp\|\bg_{t}^{\diamond}\|^2 
%         &\leq 
%         8\kappa\frac{d^2}{d+1}\norm{\nabla f(\bx)}_2^2 + 2\parent{d+11}\bar{L}^2h^2\kappa + \frac{2\sigma^2\kappa d^3}{h^2}\\
%         &\leq
%         8d\kappa \norm{\nabla f(\bx)}_2^2 + 2\parent{d+11}\bar{L}^2h^2\kappa + \frac{2\sigma^2 d^3\kappa}{h^2}\enspace.
%     \end{align*}
    
%     }
%     \evg[inline]{The bound above is better, but more annoying to work with than the previous one: it replaces $24d$ by $2(d + 11)$. If it is too annoying to use the above, simply bound $2(d + 11)$ by $24d$ which is always true }
    
%     % Combining Eq.~\eqref{eq:var_l1_2} with Eqs.~\eqref{eq:var_l1_3}--\eqref{eq:var_l1_Z4} we deduce the desired result:
%     % \begin{align*}
%     %     \Exp\|\bg_{t}^{\diamond}\|^2  \leq  \frac{24d^4\bar{L}^2h^2\kappa}{(d+1)(d+2)(d+3)} + 8\kappa\frac{d^2}{d+1}\norm{\nabla f(\bx)}_2^2 + \frac{2\sigma^2\kappa d^3}{h^2}\enspace.
%     % \end{align*}
% \end{proof}





\newpage
\section{Technical lemmas}
In our proof we will often need to deal with various recursive relations. In this section we provide a result, which are used extensively in nearly every single proof. The next result is a direct adaptations of~\cite[Lemma D.1]{akhavan2020}.
\begin{comment}
\begin{lemma}[Lemma D.1 of \cite{akhavan2020}]

\label{lemma:bis}
    Let $\{\delta_{t}\}_{t \geq 1}$ be a sequence of real numbers such that for all integers $t \geq t_{0} \geq 4$, 
    \begin{equation}
    \label{ch:00}
        \delta_{t+1} \leq \left(1 - \frac{3}{t} \right)\delta_{t} + \sum_{i=1}^{N}\frac{a_{i}}{t^{p_{i}+1}}\enspace,
    \end{equation}
where $p_{i} \in (0, 3)$ and $a_{i}\geq0$ for $i \in [N] $. Then for $t \geq t_{0} \geq 4$, we have
\begin{equation}
\label{ch:res0}
        \delta_{t} \leq \frac{(t_{0}-1)\delta_{t_{0}}}{t}+\sum_{i=1}^{N}\frac{a_{i}}{(3-p_{i})t^{p_{i}}}\enspace.
    \end{equation}
\end{lemma}
\end{comment}
% \begin{proof}
% For any fixed $t > 0$ the convexity of the mapping $u\mapsto g(u)=(t+u)^{-p}$ implies that  $g(1)-g(0)\ge g'(0)$, i.e.,  
% %\begin{eqnarray}
% %\nonumber
% %(t+1)^{p}&=& t^{p} + pt^{p-1} + \sum_{i=2}^{\infty}\frac{p\dots (p-i+1)}{i!}t^{p-i}\\
% %\nonumber
% %&\leq& t^{p} + pt^{p-1} + t^{p-2}\left(\sum_{i=2}^{\infty}\frac{p\dots (p-i+1)}{i!}+(1+p)-(1+p)\right)\\
% %\nonumber
% %&=&t^{p} + pt^{p-1} + (2^{p}-1-p)t^{p-2} \leq t^{p} + pt^{p-1},
% %\end{eqnarray}
% %where the last inequality follows from the fact that $2^{p}-p-1<0$, for $0<p<1.$ Now due to the last display, we obtain 
% \begin{eqnarray*}
% % \label{ch:1}
% \frac{1}{t^{p}}-\frac{1}{(t+1)^{p}}
% \leq \frac{p}{t^{p+1}}\enspace.
% \end{eqnarray*}
% Thus, since $\tfrac{1}{t^p} - \tfrac{p}{t^{p+1}} = \tfrac{(1 - p) + (t - 1)}{t^{p+1}} \leq \tfrac{1}{(t+1)^p}$ we deduce that
% \begin{eqnarray}
% \label{ch:20}
% \frac{a_i}{t^{p+1}}\leq \frac{a_i}{1-p}\left(\frac{1}{(t+1)^{p}} - \Big(1-\frac{1}{t}\Big)\frac{1}{t^{p}} \right)\enspace.
% \end{eqnarray}
% Using Eq.~\eqref{ch:00} and Eq.~\eqref{ch:20} and rearranging terms, for any $t \geq t_{0}$ we get 
% \begin{eqnarray}
% \nonumber
% \delta_{t+1}-\sum_{i=1}^{N}\frac{a_{i}}{(1-p_{i})(t+1)^{p_{i}}}\le\Big(1-\frac{1}{t}\Big)\left[\delta_{t} - \sum_{i=1}^{N}\frac{a_{i}}{(1-p_{i})t^{p_{i}}}\right]\enspace.
% \end{eqnarray}
% Letting $\tau_{t} = \delta_{t} - \sum_{i=1}^{N}\tfrac{a_{i}}{(1-p_{i})t^{p_{i}}}$ we have $\tau_{t+1}\leq (1-\frac{1}{t}) \tau_{t}$. Now, if $\tau_{t_{0}} \leq 0$ then $\tau_{t} \leq 0$ for any $t \geq t_{0}$ and thus
% (\ref{ch:res0}) holds. Otherwise, if $\tau_{t_0}>0$ then for $t\ge t_{0}+1$ we have
% \[
% \tau_{t}\leq \tau_{t_{0}}\prod_{i={t_{0}}}^{t-1}\Big(1-\frac{1}{i}\Big)\leq \frac{2(t_{0}-1)\tau_{t_{0}}}{t}\le \frac{2(t_{0}-1)\delta_{t_{0}}}{t}\enspace.
% \]
% Thus, (\ref{ch:res0}) holds in this case as well.
% \end{proof}
\begin{lemma}
\label{lemma:bisev}
    Let $\{\delta_{t}\}_{t \geq 1}$ be a sequence of real numbers such that for all integers $t > t_{0} \geq 1$, 
    \begin{equation}
    \label{ch:0}
        \delta_{t+1} \leq \left(1 - \frac{2}{t} \right)\delta_{t} + \sum_{i=1}^{N}\frac{a_{i}}{t^{p_{i}+1}}\enspace,
    \end{equation}
where $p_{i} \in (0,2)$ and $a_{i}\geq0$ for $i \in [N] $. Then for $t \geq t_{0} \geq 3$, we have
\begin{equation}
\label{ch:res}
        \delta_{t} \leq \frac{2(t_{0}-1)\delta_{t_{0}}}{t}+\sum_{i=1}^{N}\frac{a_{i}}{(2-p_{i})t^{p_{i}}}\enspace.
    \end{equation}
\end{lemma}
\begin{proof}
For any fixed $t > 0$ the convexity of the mapping $u\mapsto g(u)=(t+u)^{-p}$ implies that  $g(1)-g(0)\ge g'(0)$, i.e.,  
%\begin{eqnarray}
%\nonumber
%(t+1)^{p}&=& t^{p} + pt^{p-1} + \sum_{i=2}^{\infty}\frac{p\dots (p-i+1)}{i!}t^{p-i}\\
%\nonumber
%&\leq& t^{p} + pt^{p-1} + t^{p-2}\left(\sum_{i=2}^{\infty}\frac{p\dots (p-i+1)}{i!}+(1+p)-(1+p)\right)\\
%\nonumber
%&=&t^{p} + pt^{p-1} + (2^{p}-1-p)t^{p-2} \leq t^{p} + pt^{p-1},
%\end{eqnarray}
%where the last inequality follows from the fact that $2^{p}-p-1<0$, for $0<p<1.$ Now due to the last display, we obtain 
\begin{eqnarray*}
% \label{ch:1}
\frac{1}{t^{p}}-\frac{1}{(t+1)^{p}}
\leq \frac{p}{t^{p+1}}\enspace.
\end{eqnarray*}
Thus, using the fact that $\tfrac{1}{t^p} - \tfrac{p}{t^{p+1}} = \tfrac{(2 - p) + (t - 2)}{t^{p+1}} \leq \tfrac{1}{(t+1)^p}$,
\begin{eqnarray}
\label{ch:2}
\frac{a_i}{t^{p+1}}\leq \frac{a_i}{2-p}\left(\frac{1}{(t+1)^{p}} - \Big(1-\frac{2}{t}\Big)\frac{1}{t^{p}} \right)\enspace.
\end{eqnarray}
Using Eq.~\eqref{ch:0} and Eq.~\eqref{ch:2} and rearranging terms, for any $t \geq t_{0}$ we get 
\begin{eqnarray}
\nonumber
\delta_{t+1}-\sum_{i=1}^{N}\frac{a_{i}}{(2-p_{i})(t+1)^{p_{i}}}\le\Big(1-\frac{2}{t}\Big)\left[\delta_{t} - \sum_{i=1}^{N}\frac{a_{i}}{(2-p_{i})t^{p_{i}}}\right]\enspace.
\end{eqnarray}
Letting $\tau_{t} = \delta_{t} - \sum_{i=1}^{N}\tfrac{a_{i}}{(2-p_{i})t^{p_{i}}}$ we have $\tau_{t+1}\leq (1-\tfrac{2}{t}) \tau_{t}$. Now, if $\tau_{t_{0}} \leq 0$ then $\tau_{t} \leq 0$ for any $t \geq t_{0}$ and thus
(\ref{ch:res}) holds. Otherwise, if $\tau_{t_0}>0$ then for $t\ge t_{0}+1$ we have
\[
\tau_{t}\leq \tau_{t_{0}}\prod_{i={t_{0}}}^{t-1}\Big(1-\frac{2}{i}\Big)\leq \tau_{t_{0}}\prod_{i={t_{0}}}^{t-1}\Big(1-\frac{1}{i}\Big)\le \frac{(t_{0}-1)\tau_{t_{0}}}{t}\le \frac{2(t_{0}-1)\delta_{t_{0}}}{t}\enspace.
\]
Thus, (\ref{ch:res}) holds in this case as well.
\end{proof}








\newpage
\section{Upper bounds: only smoothness}
In this section we provide the proof of Theorem~\ref{nonc} and Theorem~\ref{nonc:simp} for Algorithms~\ref{algose} ($\ell_2$-randomization) and~\ref{algo:simplex} ($\ell_1$-randomization) respectively.

Both of these proof follow the same pattern and can be seen as corollaries to Lemma \ref{HighSF}, which states that
\begin{align*}
        \Exp\left[\norm{\nabla f(\bx_S)}^2\right] \leq \frac{2\delta_1+ \sum_{t = 1}^T\eta_t\parent{b_t^2 + \bL\eta_t v_t}}{\sum_{t = 1}^T\eta_t\parent{1 - \bL\eta_tm}}\enspace.
\end{align*}
In particular, using corresponding bounds on the variance and bias, we substitute these values in the above inequality and focus on deriving an upper bound for the resulting sequences. 


{\color{black}
\begin{proof}[Proof of Theorem~\ref{nonc} ($\ell_2$-randomization)]
% Corollary \ref{HighSF} yields
% \begin{align}\label{noncal0}
%         \Exp\left[\norm{\nabla f(\bx_S)}^2\right] \leq \frac{2\delta_1+ \sum_{t = 1}^T\eta_t\parent{b_t^2 + \bL\eta_t v_t}}{\sum_{t = 1}^T\eta_t\parent{1 - \bL\eta_tm}}\enspace.
%     \end{align}
Let $\delta_1 = \Exp[f(\bx_1)] - f^{\star}$, then in the notation of Lemma~\ref{HighSF}, recalled above in the beginning of this part of the appendix, Lemma \ref{lem:bias_sphere} (for the bias) with Lemma \ref{lem:var_sphere_v2} (more precisely, Eq.~\eqref{eq:var_l2_for_proofs} for the variance) yield
% Thanks to Lemma \ref{lem:bias_sphere} and Lemma \ref{lem:var_sphere_v2}, we have
\begin{align*}
    &b_t^2 \leq \left(\frac{\kappa_\beta L}{(\ell-1)!}\right)^2h_{t}^{2(\beta-1)}\quad\text{and}\quad
    v_t = 4d\kappa\bL^2 h_t^{2}+\frac{d^2\sigma^2\kappa}{2h_t^2}
    \quad\text{and}\quad
    m = 4d\kappa\enspace.
\end{align*}
Substituting the above into Lemma~\ref{HighSF}, we deduce that
   \begin{align}\label{noncal1}
        \Exp\left[\norm{\nabla f(\bx_S)}^2\right] \leq \frac{2\delta_1 + \sum_{t = 1}^T\eta_t\parent{\cst_3h_{t}^{2(\beta-1)} + d^2\eta_t\big(\cst_4d^{-1}h_t^2+\cst_5h_t^{-2}\big)}}{\sum_{t = 1}^T\eta_t\parent{1 - 4d\kappa\bL \eta_t}}\enspace,
    \end{align}
    where $\cst_3 = \Big(\tfrac{\kappa_\beta L}{(\ell-1)!}\Big)^2$, $\cst_4 = 4\kappa \bL^3$, and $\cst_5 = \frac{\kappa \sigma^2\bL}{2}$. Since $\eta_t \leq \tfrac{1}{8\kappa \bar{L}d}$, we have $1-4\kappa \bar{L}d\eta_t \geq \tfrac{1}{2}$, for all $t \geq 1$, leading to
    \begin{equation}
    \label{noncal2}
    \begin{aligned}
        \Exp\left[\norm{\nabla f(\bx_S)}^2\right] &\leq
        \frac{4\delta_1}{\sum_{t=1}^{T}\eta_t} + \frac{\sum_{t = 1}^T2\eta_t\parent{\cst_3h_{t}^{2(\beta-1)} + d^2\eta_t\big(\cst_4d^{-1}h_t^2+\cst_5h_t^{-2}\big)}}{\sum_{t = 1}^T\eta_t}\\
        &=
        \underbrace{\frac{4\delta_1}{\sum_{t=1}^{T}\eta_t}}_{=: \tT_1} + \underbrace{\frac{2\cst_3\sum_{t=1}^{T}\eta_t h_t^{2(\beta-1)}}{\sum_{t=1}^{T}\eta_t}}_{=: \tT_2} + \underbrace{\frac{2d^2\sum_{t=1}^{T}\eta_t^2\big(\cst_4d^{-1}h_t^2+\cst_5h_t^{-2}\big)}{\sum_{t=1}^{T}\eta_t}}_{=: \tT_3}\enspace.
    \end{aligned}
    \end{equation}

We will bound the above three terms separately.    
\paragraph{Bounding each term.}
But first, let us introduce the following shorthand notation: $a_T \triangleq d^{-\frac{2(\beta-1)}{2\beta-1}}T^{-\frac{\beta}{2\beta}}$. In this notation, we have $\eta_t = \min\left(\frac{1}{8\kappa \bL d},a_T\right)$. Note that the for the inverse denominator appearing in all three terms of Eq.~\eqref{noncal2} we can write the following bound
% \evg[inline]{Arya, we need a lower bound on the denominator, not upper bound. So you need an extra factor of $1/2$. Or if you wish, we can just get rid of one of the terms, involving $a_T$, which is simpler to handle.}
    \begin{align*}
        \left(\sum_{t=1}^{T}\eta_t\right)^{-1} = \frac{1}{\min\left(\frac{T}{8\kappa \bar{L}d},Ta_T\right)}
        =
        \max\left(\frac{8\kappa \bar{L}d}{T},\frac{1}{Ta_T}\right) \leq
        \frac{8\kappa \bar{L}d}{T}+\frac{1}{Ta_T}\enspace.
    \end{align*}
Furthermore, using the above inequality, and the fact that $\eta_t \leq a_T$, each term in Eq.~\eqref{noncal2} can be bounded as follows:
\begin{align*}
% [\parindent]
% \begin{equation*}
% \begin{split}\label{noncal3}
    &\tT_1
    % = \frac{4\delta_1}{\sum_{t=1}^{T}\eta_t}
    \leq \left(\frac{32\kappa\bL d}{T} + \frac{4}{a_T T}\right)\delta_1\enspace,\\
% \end{split}
% \end{equation*}
% \end{fleqn}
% \begin{fleqn}[\parindent]
% \begin{equation*}
% \begin{split}\label{noncal4}
    &\tT_2
    % = \frac{2\cst_3\sum_{t=1}^{T}\eta_t h_t^{2(\beta-1)}}{\sum_{t=1}^{T}\eta_t}
    \leq
    2\cst_3 a_T\left(\frac{8\kappa \bL d }{T} + \frac{1}{Ta_T}\right)\sum_{t=1}^{T}h_{t}^{2(\beta-1)}
    \leq
    \cst_6 a_T\left(\frac{d}{T}+\frac{1}{Ta_T}\right)\sum_{t=1}^{T}h_{t}^{2(\beta-1)}\enspace,\\
% \end{split}
% \end{equation*}
% \end{fleqn}
% % and
% \begin{fleqn}[\parindent]
% \begin{equation*}
% \begin{split}
   &\tT_3
%   = \frac{2d^2\sum_{t=1}^{T}\eta_t^2\big(\cst_4d^{-1}h_t^2+\cst_5h_t^{-2}\big)}{\sum_{t=1}^{T}\eta_t}
   \leq 2d^2a_T^2\Big(\frac{8\kappa \bL d }{T} + \frac{1}{Ta_T}\Big)\sum_{t=1}^{T}\left(\cst_4d^{-1}h_t^2+\cst_5h_t^{-2}\right)
   \leq \frac{\cst_7d^2a_T^2}{T}\left(d + a_T^{-1}\right)\sum_{t=1}^{T}\big(d^{-1}h_t^2+h_t^{-2}\big) \enspace,
% \end{split}
% \end{equation*}
\end{align*}
where we introduced $\cst_6 = 2\cst_3\big(8\kappa \bL+1\big)$ and $\cst_7 = 2\big(8\kappa \bL+1\big)\big(\cst_4 + \cst_5\big)$.
\paragraph{Substitution.}
Substituting the above inequalities into Eq.~\eqref{noncal2} and rearranging we deduce that
\begin{align*}
    \Exp\left[\norm{\nabla f(\bx_S)}^2\right] \leq \left(\frac{32\kappa\bL d}{T}+\frac{4}{a_T T}\right)\delta_1 + \frac{(da_T+1)}{T}\sum_{t=1}^{T}\Big(\cst_6h_t^{2(\beta-1)}+\cst_7d^2a_T\big(d^{-1}h_t^2+h_t^{-2}\big)\Big).
\end{align*}
It remain to bound the second term in the above bound.
Since $h_t = h_T$ for $t = 1,\dots,T$, then we can write 
\begin{align}\label{noncal10}
    \Exp\norm{\nabla f(\bx_S)}^2 \leq \left({32\kappa\bL d}{+}\frac{4}{a_T }\right)\frac{\delta_1}{T} + (da_T{+}1)\Big(\cst_6h_T^{2(\beta-1)}+\cst_7d^2a_T\big(d^{-1}h_T^2+h_T^{-2}\big)\Big).
\end{align}
% Let us clarify the choice of the parameters for this result. We would like to minimize the second term on right hand side of the above inequality simultaneously over $a_T$ and $h_T$, which (up to absolute multiplicative constant) gives us exactly the choice of the parameters announced in the statement of this result.
% Therefore $h_T = \Big(\frac{d^2}{T}\Big)^{\frac{1}{2(2\beta-1)}}$ and 
% $a_T = d^{-\frac{2(\beta-1)}{2\beta-1}}T^{-\frac{\beta}{2\beta-1}}$, which justifies the choice of $\eta_t$ and $h_t$ for this problem, with $t = 1,\dots,T$.
Finally, substituting the expressions for $a_T$ and $h_T$ into the above bound, the right hand side of Eq.~\eqref{noncal10} reduces to
\begin{align*}
    % \Exp\norm{\nabla f(\bx_S)}^2
    % &\leq \left(\frac{64\kappa\bL d}{T}+\frac{4}{a_T T}\right)\delta_1 + (da_T+1)\left(\cst_6h_T^{2(\beta-1)}+\cst_7d^2a_T\left(d^{-1}h_T^2+h_T^{-2}\right)\right)
    % \\
    % &\leq
    \frac{32\kappa\bar{L}d}{T}\delta_1 +\left(4\delta_1 + \left(\left(\frac{d}{T^{\beta}}\right)^{\frac{1}{2\beta-1}}{+}1\right)\left(\cst_6+\cst_7\left(1+d^{\frac{5-2\beta}{2\beta-1}}T^{-\frac{2}{2\beta-1}}\right)\right)\right)\left(\frac{d^2}{T}\right)^{\frac{\beta-1}{2\beta-1}}.
\end{align*}
To conclude, we note that the assumption $T \geq d^{\frac{1}{\beta}}$, implies that for all $\beta \geq 2$ we have  $d^{\tfrac{5-2\beta}{2\beta-1}}T^{-\frac{2}{2\beta-1}} \leq 1$ and $\left(\tfrac{d}{T^{\beta}}\right)^{\frac{1}{2\beta-1}}\leq 1$. Therefore, we have
\begin{align*}
    \Exp\left[\norm{\nabla f(\bx_S)}^2\right]
    &\leq
    \frac{32\kappa\bar{L}d}{T}\delta_1 +\Big(4\delta_1 + 2\Big(\cst_6+2\cst_7\Big)\Big)\Big(\frac{d^2}{T}\Big)^{\frac{\beta-1}{2\beta-1}}
    \leq
    \Big(\cst_1\delta_1 + \cst_2\Big)\Big(\frac{d^2}{T}\Big)^{\frac{\beta-1}{2\beta-1}},
\end{align*}
where we introduced $\cst_1 = 32\kappa\bL+4$ and $\cst_2 = 2\big(\cst_6+2\cst_7\big)$.
\end{proof}
}
\begin{comment}
\begin{proof}[Proof of Theorem~\ref{nonc:simp} ($\ell_1$-randomization)]
 By Lemma \ref{HighSF}, we have
\begin{align}\label{gre1}
    \Exp\norm{\nabla f(\bx_S)}^2\leq \frac{2\delta_1 + \sum_{t=1}^{T}\eta_t\left(b_t^2+\bL\eta_tv_t\right)}{\sum_{t=1}^{T}\eta_t\left(1-\bL\eta_t m\right)},
\end{align}
where $\delta_1 = \Exp[f(\bx_1)]-f^{\star}$. For Algorithm \ref{algo:simplex}, by Lemma \ref{lem:bias_simplex} we get $b_t^2\leq (\kappa_\beta \ell L)^2h_t^{2(\beta-1)}d^{1-\beta}$, with $\ell = \floor{\beta}$. Also, by Lemma \ref{lem:var_simplex} we have $v_t = 3\bar{L}^2 \kappa h_t^2d + \frac{2\sigma^2\kappa d^2}{h_t^2}$, and $m \leq 8\kappa d$. By substituting these terms in \eqref{gre1}, we obtain
\begin{align*}
    \Exp \norm{\nabla f(\bx_S)}^2 \leq\frac{2\delta_1+\sum_{t=1}^{T}\eta_t\left(\cst_3h_t^{2(\beta-1)}d^{1-\beta}+\eta_td\left(\cst_4h_t^2 + \cst_5d^2h_{t}^{-2}\right)\right)}{\sum_{t=1}^{T}\eta_t(1-8\bL\kappa d\eta_t)},
\end{align*}
where $\cst_3 = (\kappa_\beta \ell L)^2$, $\cst_4 = 3\bL^3\kappa$, and $\cst_5 = \bL\sigma^2\kappa$. Since $\eta_t \leq \frac{1}{16\bL\kappa d}$, we have $1-8\bL\kappa d\eta_t \leq \frac{1}{2}$. Therefore,
\begin{align}\label{gre2}
    \Exp \norm{\nabla f(\bx_S)}^2 \leq\frac{4\delta_1}{\sum_{t=1}^{T}\eta_t}+\frac{\sum_{t=1}^{T}2\eta_t\left(\cst_3h_t^{2(\beta-1)}d^{1-\beta}+\eta_td\left(\cst_4h_t^2 + \cst_5d^2h_{t}^{-2}\right)\right)}{\sum_{t=1}^{T}\eta_t}.
\end{align}
Denote $\gamma = d^{-\frac{2(\beta-1)}{2\beta-1}}T^{-\frac{\beta}{2\beta-1}}$ and note that $\eta_t = \min\left(\frac{1}{16\bL\kappa d}, \gamma\right)$. Then, for the term in the denominators we have 
    \begin{align*}
        \Big(\sum_{t=1}^{T}\eta_t\Big)^{-1} = \frac{1}{\min\big(\frac{T}{16\kappa \bar{L}d},T\gamma\big)} = \max\Big(\frac{18\kappa \bar{L}d}{T},\frac{1}{T\gamma}\Big) \leq \frac{16\kappa \bar{L}d}{T}+\frac{1}{T\gamma}.
    \end{align*}
Now, for the terms appear in \eqref{gre2} we can see
\begin{fleqn}[\parindent]
\begin{equation*}
\begin{split}\label{noncal3}
    \frac{4\delta_1}{\sum_{t=1}^{T}\eta_t} \leq \Big(\frac{64\kappa\bL d}{T} + \frac{4}{\gamma T}\Big)\delta_1,
\end{split}
\end{equation*}
\end{fleqn}
\begin{fleqn}[\parindent]
\begin{equation*}
\begin{split}\label{noncal4}
    \frac{2\cst_3d^{1-\beta}\sum_{t=1}^{T}\eta_t h_t^{2(\beta-1)}}{\sum_{t=1}^{T}\eta_t} &\leq 2\cst_3 d^{1-\beta}\gamma\Big(\frac{18\kappa \bL d }{T} + \frac{1}{T\gamma}\Big)\sum_{t=1}^{T}h_{t}^{2(\beta-1)}
    \\&\leq \cst_6 d^{1-\beta}\gamma \Big(\frac{d}{T}+\frac{1}{T\gamma}\Big)\sum_{t=1}^{T}h_{t}^{2(\beta-1)},
\end{split}
\end{equation*}
\end{fleqn}
\begin{fleqn}[\parindent]
\begin{equation*}
\begin{split}
   \frac{2\cst_4d\sum_{t=1}^{T} \eta_t^2h_t^2}{\sum_{t=1}^{T}\eta_t} 
   &\leq 2\cst_4d\gamma^2\Big(\frac{18\kappa \bL d }{T} + \frac{1}{T\gamma}\Big)\sum_{t=1}^{T}h_t^2
   \leq
   \cst_7d\gamma^2\big(\frac{d}{T}+\frac{1}{T\gamma}\big)\sum_{t=1}^{T}h_t^2,
\end{split}
\end{equation*}
\end{fleqn}
and
\begin{fleqn}[\parindent]
\begin{equation*}
\begin{split}
   \frac{2\cst_5d^3\sum_{t=1}^{T} \eta_t^2h_t^{-2}}{\sum_{t=1}^{T}\eta_t} &\leq 2\cst_5d^3\gamma^2\Big(\frac{18\kappa \bL d }{T} + \frac{1}{T\gamma}\Big)\sum_{t=1}^{T}h_t^{-2}
   \leq
   \cst_8d^3\gamma^2\Big(\frac{d}{T} + \frac{1}{T\gamma}\Big)\sum_{t=1}^{T}h_t^{-2},
\end{split}
\end{equation*}
\end{fleqn}
where $\cst_6 = 2\cst_3\big(18\kappa \bL+1\big)$, $\cst_7 = 2\cst_4\big(18\kappa \bL+1\big)$, and $\cst_8 = 2\cst_5\big(18\kappa \bL+1\big)$. Now by substituting the bounds in the above in \eqref{gre2}, we get 
\begin{align}\label{gre3}
    \Exp\norm{\nabla f(\bx_S)}^2\leq (\frac{64\kappa\bL d}{T}+\frac{4}{\gamma T})\delta_1+(\frac{d\gamma+1}{T})\sum_{t=1}^{T}\left(\cst_6d^{1-\beta}h_t^{2(\beta-1)}+d\gamma\left(\cst_7h_t^2+\cst_8d^2h_t^{-2}\right)\right).
\end{align}
Now note that to minimze the term 
\begin{align*}
    \frac{1}{\gamma T} + d^{1-\beta}h_T^{2(\beta-1)} + d^3\gamma h_T^{-2},
\end{align*}
we should have
$$\gamma = \frac{h_T}{\sqrt{d^3T}},\quad\quad\gamma= d^{-\beta-2}h_T^{2\beta},$$
which yields $h_T = d^{\frac{2\beta+1}{2(2\beta-1)}}T^{-\frac{1}{2(2\beta-1)}}$, and $\gamma = d^{\frac{-2\beta+2}{2\beta-1}}T^{-\frac{\beta}{2\beta-1}}.$ This justifies the assignments for $\eta_t$ and $h_t$, in this theorem. Now, by substituting $\eta_t$ and $h_t$ in \eqref{gre3}, we get
\begin{align*}
    \Exp\norm{\nabla f(\bx_S)}^2\leq \frac{64\kappa\bL d}{T}\delta_1+\left(4\delta_1+(\left(\frac{d}{T^{\beta}}\right)^{\frac{1}{2\beta-1}} +1)\left(\cst_6+\cst_8+\cst_7\left(\frac{d^2}{T}\right)^{\frac{2}{2\beta-1}}\right)\left(\frac{d^2}{T}\right)\right)^{\frac{\beta-1}{2\beta-1}}
\end{align*}
Since $T\geq d^2$, we have $\frac{d}{T^{\beta}},\frac{d^{2}}{T}\leq 1$. Therefore, we can write
\begin{align*}
    \Exp\norm{\nabla f(\bx_S)}^2\leq \left(\cst_1\delta_1+\cst_2\right)\left(\frac{d^2}{T}\right)^{\frac{\beta-1}{2\beta-1}},
\end{align*}
where $\cst_1 = 64\kappa\bL+4$, and $\cst_2=2\left(\cst_6+\cst_7+\cst_8\right)$.
\end{proof}
\end{comment}
\begin{proof}[Proof of Theorem~\ref{nonc:simp} ($\ell_1$-randomization)]
We start identically to the proof of the previous result (Theorem~\ref{nonc}). 
%  By Lemma \ref{HighSF}, we have
% \begin{align}\label{gre1}
%     \Exp\norm{\nabla f(\bx_S)}^2\leq \frac{2\delta_1 + \sum_{t=1}^{T}\eta_t\left(b_t^2+\bL\eta_tv_t\right)}{\sum_{t=1}^{T}\eta_t\left(1-\bL\eta_t m\right)},
% \end{align}
% where $\delta_1 = \Exp[f(\bx_1)]-f^{\star}$.
Lemma \ref{lem:bias_simplex} (for the the bias) and Lemma~\ref{lem:var_l1_v2} (more precisely, Eq.~\eqref{eq:var_l1_for_proofs} for the variance) imply that
\begin{align*}
    b_t^2\leq (\kappa_\beta \ell L)^2h_t^{2(\beta-1)}d^{1-\beta}\qquad\text{and}\qquad{\color{black}v_t = 856\bL^{2}\kappa h_t^2+\frac{d^3\kappa\sigma^2}{2h_t^2}}\qquad\text{and}\qquad{\color{black}m = 87d\kappa}\enspace,
\end{align*}
with $\ell = \floor{\beta}$.
Substituting the above quantities into Lemma~\ref{HighSF}, we deduce that
\begin{align*}
    \Exp \norm{\nabla f(\bx_S)}^2 \leq\frac{2\delta_1+\sum_{t=1}^{T}\eta_t\left(\cst_3h_t^{2(\beta-1)}d^{1-\beta}+\eta_t\left(\cst_4h_t^2 + \cst_5d^3h_{t}^{-2}\right)\right)}{\sum_{t=1}^{T}\eta_t(1-{\color{black}87\bL\kappa d\eta_t})}\enspace,
\end{align*}
where $\cst_3 = (\kappa_\beta \ell L)^2$, ${\color{black}\cst_4 = 856\bL^{3}\kappa}$, and $\cst_5 = \frac{\bL\sigma^2\kappa}{2}$. Since, by definition of $\eta_t$, we have ${\color{black}\eta_t \leq \tfrac{1}{174\bL\kappa d}}$, we also have ${\color{black}1-87\bL\kappa d\eta_t \leq \tfrac{1}{2}}$. Therefore, the above bound reduces to
\begin{align}\label{gre2}
    \Exp \norm{\nabla f(\bx_S)}^2 \leq\frac{4\delta_1}{\sum_{t=1}^{T}\eta_t}+\frac{\sum_{t=1}^{T}2\eta_t\left(\cst_3h_t^{2(\beta-1)}d^{1-\beta}+\eta_t\left(\cst_4h_t^2 + \cst_5d^3h_{t}^{-2}\right)\right)}{\sum_{t=1}^{T}\eta_t}\enspace.
\end{align}
As for the proof of Theorem~\ref{nonc}, introduce the short-hand notation $a_T = d^{-\frac{2(\beta-1)}{2\beta-1}}T^{-\frac{\beta}{2\beta-1}}$ and note that using this notation ${\color{black}\eta_t = \min\left(\frac{1}{174\bL\kappa d}, a_T\right)}$. Then, the inverse of denominators in Eq.~\eqref{gre2} can be bounded 
    \begin{align*}
        \left(\sum_{t=1}^{T}\eta_t\right)^{-1} ={\color{black} \frac{1}{\min\big(\frac{T}{174\bL\kappa d},Ta_T\big)} = \max\Big(\frac{174\bL\kappa d}{T},\frac{1}{Ta_T}\Big) \leq \frac{174\bL\kappa d}{T}+\frac{1}{Ta_T}}\enspace.
    \end{align*}
\paragraph{Bounding each term in Eq.~\eqref{gre2}. } Thanks to the above derive bound we deduce that
\begin{fleqn}[\parindent]
\begin{equation*}
\begin{split}\label{noncal3}
    \frac{4\delta_1}{\sum_{t=1}^{T}\eta_t} \leq \Big({\color{black}\frac{696\kappa\bL d}{T}} + \frac{4}{a_T T}\Big)\delta_1,
\end{split}
\end{equation*}
\end{fleqn}
\begin{fleqn}[\parindent]
\begin{equation*}
\begin{split}\label{noncal4}
    \frac{2\cst_3d^{1-\beta}\sum_{t=1}^{T}\eta_t h_t^{2(\beta-1)}}{\sum_{t=1}^{T}\eta_t} &\leq 2\cst_3 d^{1-\beta}a_T\Big(\frac{174\kappa \bL d }{T} + \frac{1}{Ta_T}\Big)\sum_{t=1}^{T}h_{t}^{2(\beta-1)}
    \\&\leq \cst_6 d^{1-\beta}a_T \Big(\frac{d}{T}+\frac{1}{Ta_T}\Big)\sum_{t=1}^{T}h_{t}^{2(\beta-1)}\enspace,
\end{split}
\end{equation*}
\end{fleqn}
\begin{fleqn}[\parindent]
\begin{equation*}
\begin{split}
   \frac{2\cst_4\sum_{t=1}^{T} \eta_t^2h_t^2}{\sum_{t=1}^{T}\eta_t} 
   &\leq 2\cst_4a_T^2\Big({\color{black}\frac{174\kappa \bL d }{T}} + \frac{1}{Ta_T}\Big)\sum_{t=1}^{T}h_t^2
   \leq
   \cst_7a_T^2\left(\frac{d}{T}+\frac{1}{Ta_T}\right)\sum_{t=1}^{T}h_t^2\enspace,
\end{split}
\end{equation*}
\end{fleqn}
and
\begin{fleqn}[\parindent]
\begin{equation*}
\begin{split}
   \frac{2\cst_5d^3\sum_{t=1}^{T} \eta_t^2h_t^{-2}}{\sum_{t=1}^{T}\eta_t} &\leq 2\cst_5d^3a_T^2\Big({\color{black}\frac{174\kappa \bL d }{T}} + \frac{1}{Ta_T}\Big)\sum_{t=1}^{T}h_t^{-2}
   \leq
   \cst_8d^3a_T^2\Big(\frac{d}{T} + \frac{1}{Ta_T}\Big)\sum_{t=1}^{T}h_t^{-2}\enspace,
\end{split}
\end{equation*}
\end{fleqn}
where ${\color{black}\cst_6 = 2\cst_3\big(174\kappa \bL+1\big)}$, ${\color{black}\cst_7 = 2\cst_4\big(174\kappa \bL+1\big)}$, and ${\color{black}\cst_8 = 2\cst_5\big(174\kappa \bL+1\big)}$.

\paragraph{Substitution.} Substituting the bounds above into Eq.~\eqref{gre2}, we get 
\begin{align}\label{gre3}
    \Exp\norm{\nabla f(\bx_S)}^2\leq \left({\color{black}\frac{696\kappa\bL d}{T}}+\frac{4}{a_T T}\right)\delta_1+\left(\frac{da_T+1}{T}\right)\sum_{t=1}^{T}\left(\cst_6d^{1-\beta}h_t^{2(\beta-1)}+a_T\left(\cst_7h_t^2+\cst_8d^3h_t^{-2}\right)\right)\enspace.
\end{align}
% Now note that to minimize the term 
% \begin{align*}
%     \frac{1}{a_T T} + d^{1-\beta}h_T^{2(\beta-1)} + d^3a_T h_T^{-2}\enspace,
% \end{align*}
% we should have
% $$a_T = \frac{h_T}{\sqrt{d^3T}},\quad\quada_T= d^{-\beta-2}h_T^{2\beta},$$
% which yields $h_T = d^{\frac{2\beta+1}{2(2\beta-1)}}T^{-\frac{1}{2(2\beta-1)}}$, and $\gamma = d^{\frac{-2\beta+2}{2\beta-1}}T^{-\frac{\beta}{2\beta-1}}.$ This justifies the assignments for $\eta_t$ and $h_t$, in this theorem. Now, by
Substituting $\eta_t$ and $h_t$ into Eq.~\eqref{gre3}, we deduce that
\begin{align*}
    \Exp\norm{\nabla f(\bx_S)}^2\leq {\color{black}\frac{696\kappa\bL d}{T}}\delta_1+\left(4\delta_1+\left(\left(\frac{d}{T^{\beta}}\right)^{\frac{1}{2\beta-1}} +1\right)\left(\cst_6+\cst_8+\cst_7{\color{black}\left(\frac{d^{5-2\beta}}{T^2}\right)^{\frac{1}{2\beta-1}}}\right)\right)\left(\frac{d^2}{T}\right)^{\frac{\beta-1}{2\beta-1}}\enspace.
\end{align*}
Since, by assumption, ${\color{black}T\geq d^{\frac{1}{\beta}}}$, we have $\frac{d}{T^{\beta}}$ and $\frac{d^{5-2\beta}}{T^2}\leq 1$. Thus, 
\begin{align*}
    \Exp\norm{\nabla f(\bx_S)}^2\leq \left(\cst_1\delta_1+\cst_2\right)\left(\frac{d^2}{T}\right)^{\frac{\beta-1}{2\beta-1}}\enspace,
\end{align*}
where $\cst_1 = {\color{black}696\kappa\bL}+4$, and $\cst_2=2\left(\cst_6+\cst_7+\cst_8\right)$.
\end{proof}
\newpage
\section{Upper bounds: gradient dominant functions}
\begin{comment}

\begin{proof}[Proof of Theorem~\ref{evgoo}]
Since the gradient of $f$ is $\bar{L}$-Lipschitz continuous, then
\begin{align*}
    f(\bx_{t+1}) &\leq f(\bx_t) - \eta_t \langle \nabla f(\bx_t),\bg_t \rangle +\frac{\bar{L}\eta_t^2}{2}\norm{\bg_t}^2\\&\leq f(\bx_t)
    -\eta_t\norm{\nabla f(\bx_t)}^2 + \eta_t\langle\nabla f(\bx_t), \nabla f(\bx_t) - \bg_t \rangle +\frac{\bar{L}\eta_t^2}{2}\norm{\bg_t}^2.
\end{align*}
Taking conditional expectation from both sides, we deduce that
\begin{align*}
    \Exp[f(\bx_{t+1}) \mid \bx_t]
    &\leq
    f(\bx_{t}) -\eta_{t}\norm{\nabla f(\bx_t)}^2 + \eta_t \langle\nabla f(\bx_t), \nabla f(\bx_t) - \Exp[\bg_t \mid \bx_t]\rangle +\frac{\bar{L}\eta_t^2}{2}\Exp[\norm{\bg_t}^2 \mid \bx_t]
    \\
    &\leq f(\bx_t) -\frac{\eta_t}{2}\norm{\nabla f(\bx_t)}^2 +\frac{\eta_t}{2} \norm{\nabla f(\bx_t) - \Exp[\bg_t \mid \bx_t]}^2 +\frac{\bar{L}\eta_t^2}{2}\Exp[\norm{\bx_t}^2 \mid \bx_t]\enspace,
\end{align*}
where the second line is obtained by Cauchy-Swartz inequality combined with $2ab \leq a^2 + b^2$.
Let us introduce the following short-hand notation $\delta(t) \triangleq \Exp[f(\bx_t)] - f(\bx^*)$. We substract $f(\bx^*)$ from both sides of the last inequality and take the total expectation. Furthermore, applying Lemma~\ref{tru} to control the bias term and Lemma 2.4 in \cite{akhavan2020} which gives the control on the variance term, we obtain
% taking total expectation  and subtracting $f(x^*)$ from both sides, implies
\begin{align*}
    \delta(t+1) \leq \delta(t)+ \parent{-\frac{\eta_t}{2}+\frac{L\eta_t^{2}}{2}9d\kappa }\norm{\nabla f(x_t)}^2+\frac{(\kappa_{\beta}L)^2}{2}\eta_th_{t}^{2(\beta-1)} + \frac{3L\kappa\eta_{t}^2}{4}\parent{\frac{\sigma^2}{h_t^2}+\frac{3\bar{L}^2}{2}h_{t}^2}d^2\enspace.
\end{align*}
Since $\eta_t = \min\left(\tfrac{1}{18L^2d\kappa}, \tfrac{4}{\alpha t}\right)$, and $f$ is $\alpha$-gradient dominant, we can write
\begin{align*}
    \delta(t+1) \leq \parent{1 - \frac{\eta_{t}\alpha}{2}}\delta(t)+ \frac{2(\kappa_{\beta}L)^2}{\alpha t}h_{t}^{2(\beta-1)} + \frac{12L\kappa}{\alpha^2 t^2}\parent{\frac{\sigma^2}{h_t^2}+\frac{3\bar{L}^2}{2}h_{t}^2}d^2
\end{align*}
Substituting $h_{t} = t^{-\frac{1}{2\beta}}d^{\frac{1}{\beta}}$ in the above inequality and simplifying yields
\begin{align}\label{rut}
    \delta(t+1) \leq \parent{1 - \frac{\eta_{t}\alpha}{2}}\delta(t)+ \cst_1\frac{d^{2-\frac{2}{\beta}}}{\min\{\alpha, \alpha^2\}}t^{-\frac{2\beta-1}{\beta}}+\cst_2\frac{d^{2+\frac{2}{\beta}}}{\alpha^2}t^{-\frac{2\beta+1}{\beta}}\enspace,
\end{align}\evg{I did not check this derivation yet}
where $\cst_1=2(\kappa_{\beta}L)^2 + 12\bar{L}\kappa\sigma^2$, and $\cst_2 = 36L\bar{L}^2\kappa$. 
To analyze the above recursion, we proceed in two steps.
Let $T_1 = \floor{\frac{36L^2d\kappa}{\alpha}}$. \emph{First}, we analyze it for any $t =T_{1}+1,\dots,T$. In this regime of $t$, the step-size $\eta_t = \tfrac{4}{\alpha t}$, hence

\begin{align*}
    \delta(t+1) &\leq \parent{1-\frac{2}{t}}\delta(t)+ \cst_1\frac{d^{2-\frac{2}{\beta}}}{\min\{\alpha, \alpha^2\}}t^{-\frac{2\beta-1}{\beta}}+\cst_2\frac{d^{2+\frac{2}{\beta}}}{\alpha^2}t^{-\frac{2\beta+1}{\beta}}.
\end{align*}
Lemma~\ref{lemma:bisev} in appendix applied to the above recursion leads to
\begin{align*}
    \delta(T+1) &\leq \frac{2T_1}{T}\delta(T_1+1)+ \cst_3\frac{d^{2-\frac{2}{\beta}}}{\min\{\alpha, \alpha^2\}}T^{-\frac{\beta-1}{\beta}}+\cst_4\frac{d^{2+\frac{2}{\beta}}}{\alpha^2}T^{-\frac{\beta+1}{\beta}}
\end{align*}
where $\cst_3 = \frac{\beta}{\beta+1}\cst_1$, and $\cst_4 = \frac{\beta}{\beta-1}\cst_2$. On the other hand, since $T \geq d^2$, we get
\begin{align*}
    \delta(T+1) &\leq \frac{2T_1}{T}\delta(T_1+1)+ \cst_3\frac{d^{2-\frac{2}{\beta}}}{\min\{\alpha, \alpha^2\}}T^{-\frac{\beta-1}{\beta}}+\cst_4\frac{d^{2-\frac{2}{\beta}}}{\alpha^2}T^{-\frac{\beta-1}{\beta}}d^{\frac{4}{\beta}}T^{-\frac{2}{\beta}}\\&\leq
    \frac{2T_1}{T}\delta(T_1+1)+ \cst_5\frac{d^{2-\frac{2}{\beta}}}{\min\{\alpha, \alpha^2\}}T^{-\frac{\beta-1}{\beta}},
\end{align*}
where $\cst_5 = \cst_3+\cst_4$. 
To conclude the proof it is enough to bound the term $\delta(T_1 + 1)$, which we perform below. For any $t = 1, \dots, T_1$ we have $\eta_t \geq \frac{1}{T_1 + 1}$, thus, thanks to Eq.~\eqref{rut} we obtain
\begin{align*}
    \delta(t+1) \leq \left(1- \frac{1}{T_1+1}\right)\delta(t) + U(t)\enspace,
\end{align*}
where $U(t) \triangleq \cst_1\frac{d^{2-\frac{2}{\beta}}}{\min\{\alpha, \alpha^2\}}t^{-\frac{2\beta-1}{\beta}}+\cst_2\frac{d^{2+\frac{2}{\beta}}}{\alpha^2}t^{-\frac{2\beta+1}{\beta}}$ is the remainder term. The proof is concluded following the same arguments as that of Theorem~\ref{plgoo}.
\end{proof}
\end{comment}
{
% \color{black}
\begin{proof}[Proof of Theorem~\ref{plgoo} ($\ell_2$-randomization)]
By Lemma \ref{lem:general}, we have
\begin{align*}
    \delta_{t+1} \leq \delta_{t}-\frac{\eta_t}{2}(1-\bar{L}\eta_{t}m)\Exp{[\norm{\nabla f(\bx_t)}^2]}+\frac{\eta_t}{2}(b_t^2+\bar{L}\eta_tv_t),
\end{align*}
where $\delta_t = \Exp[f(\bx_t)-f^{\star}]$. Recall that $\ell =\floor{\beta}$. Applying Lemmas \ref{lem:bias_sphere} (bound on the bias) and \ref{lem:var_sphere_v2} (bound on the variance), we deduce
\begin{align*}
    \delta_{t+1}&\leq \delta_t-\frac{\eta_t}{2}(1-{\color{black}4}\bar{L}\eta_td\kappa)\Exp{[\norm{\nabla f(\bx_t)^2}]} + \eta_t\cst_3h_{t}^{2(\beta-1)} +\eta_t^2d^2\Big(\cst_4{\color{black}d^{-1}}h_t^2+\cst_5h_{t}^{-2}\Big),
\end{align*}
where $\cst_3 = \frac{1}{2}\big(\kappa_{\beta} \frac{L}{(\ell-1)!}\big)^2$, ${\color{black}\cst_4=2\kappa \bL^3}$, and ${\color{black}\cst_5 = {\color{black}\frac{\kappa\sigma^2}{4}}}$. Since, by definition of thereof, $\eta_t \leq {\color{black}\frac{1}{8\kappa\bar{L}d}}$ for $1 \leq t \leq T$, we note that ${\color{black}1 - \eta_{t}(4\kappa \bar{L}d) \geq \frac{1}{2}}$. Together with $\alpha$-gradient dominancy of $f$, we get
\begin{align}\label{sa1}
    \delta_{t+1}&\leq \delta_t\parent{1-\frac{\eta_t \alpha}{2}} + \eta_t\cst_3h_{t}^{2(\beta-1)} +\eta_t^2d^2\Big(\cst_4{\color{black}d^{-1}}h_t^2+\cst_5h_{t}^{-2}\Big).
\end{align}

Recall that $T_0 = \floor{\frac{{\color{black}32} \kappa \bar{L}d}{\alpha}}$. 
First we suppose that $T > T_0$ and divide the proof in two cases: $t \in (T_0, T]$ and $t \in [1, T_0]$. After, we treat the case $T \leq T_0$.
\paragraph{Case 1: $t \in (T_0, T]$} For any $t = T_0+1,\dots,T$, we have $\eta_t = \frac{4}{\alpha t}$ and we can write
\begin{align}\label{sa2}
    \delta_{t+1}&\leq \delta_t\left(1-\frac{2}{t}\right) + 4\cst_3\frac{h_{t}^{2(\beta-1)}}{{\alpha t}} +16\frac{d^2}{\alpha^2t^2}\Big(\cst_4{\color{black}d^{-1}}h_t^2+\cst_5h_{t}^{-2}\Big).
\end{align}
Additionally in this regime of $t$, we have $h_t = \big(\frac{d^2}{t}\big)^\frac{1}{2\beta}$. Thus, substituting this expression for $h_t$ into Eq.~\eqref{sa2}, we deduce that
\begin{align}
    \delta_{t+1}\leq \delta_t\left(1-\frac{2}{t}\right) + 4\left(\cst_3+4\cst_5\right)\frac{d^{2-\frac{2}{\beta}}}{\min\{\alpha, \alpha^2\}}t^{-\frac{2\beta-1}{\beta}} + 16\cst_4 \frac{{\color{black}d^{1+\frac{2}{\beta}}}}{\alpha^2}t^{-\frac{2\beta+1}{\beta}},
\end{align}
Applying Lemma \ref{lemma:bisev}, which allows us to take care of the above recursion, we get
\begin{align*}
    \delta_{T}\leq \frac{2T_0}{T}\delta_{T_{0}+1} + \frac{4\left(\cst_3+6\cst_5\right)}{\min\{\alpha, \alpha^2\}}\left(\frac{d^2}{T}\right)^{\frac{\beta-1}{\beta}} + \frac{32\cst_4}{\alpha^2}{\color{black}d^{-1+\frac{4}{\beta}}T^{-\frac{2}{\beta}}}\left(\frac{d^2}{T}\right)^{-\frac{\beta-1}{\beta}}\enspace.
\end{align*}
Recall that in the statement of the present result we assumed that ${\color{black}T \geq d^{2-\frac{\beta}{2}}}$, which allows us to get
\begin{align*}
    \delta_{T}\leq \frac{2T_0}{T}\delta_{T_{0}+1} + \frac{4\left(\cst_3+4\left(2\cst_4+\cst_5\right)\right)}{\min\{\alpha, \alpha^2\}}\left(\frac{d^2}{T}\right)^{\frac{\beta-1}{\beta}}\enspace.
\end{align*}
To conclude the proof, it is enough to provide an upper bound for $\delta_{T_{0}+1}.$ If $T_0 = 0$, the proof is concluded.

\paragraph{Case 2: $t \in [1, T_0]$.} For $t = 1,\dots, T_0$ we have $\eta_t = \frac{1}{8\kappa\bar{L}d}$ and $\frac{4}{(T_0+1)\alpha} \leq \eta_t \leq \frac{4}{T_0\alpha}$. Together with Eq~\eqref{sa1}, for any $t = 1, \dots, T_0$ we get
\begin{align}\label{oddca}
    \delta_{t+1} \leq \delta_t\left(1 - \frac{2}{T_0+1}\right) + \frac{4\cst_3}{T_0\alpha}h_t^{2(\beta-1)} +\frac{16d^2}{T_0^2\alpha^2}\Big(\cst_4h_t^2+\cst_5h_t^{-2}\Big)\enspace.
\end{align}
Substituting $h_t = \big(\frac{d^2}{T}\big)^{\frac{1}{2\beta}}$ and roughly bounding $(1 - \tfrac{2}{T_0 + 1})$ by $1$ implies for $t = 1, \ldots, T_0$ that
\begin{align*}
    \delta_{t+1} \leq \delta_t + \frac{4\cst_3}{T_0\alpha}\left(\frac{d^2}{T}\right)^{\frac{\beta-1}{\beta}} +\frac{16d^2}{T_0^2\alpha^2}\Big(\cst_4{\color{black}d^{-1}}\left(\frac{d^2}{T}\right)^\frac{1}{\beta}+\cst_5\left(\frac{d^2}{T}\right)^{-\frac{1}{\beta}}\Big)\enspace.
\end{align*}
Unfolding the above recursion leads to
\begin{align*}
    \delta_{T_0+1} \leq \delta_1+ \frac{4\cst_3}{\alpha}\left(\frac{d^2}{T}\right)^{\frac{\beta-1}{\beta}} +\frac{16d^2}{T_0\alpha^2}\left(\cst_4\left(\frac{d^2}{T}\right)^\frac{1}{\beta}+\cst_5\left(\frac{d^2}{T}\right)^{-\frac{1}{\beta}}\right)\enspace.
\end{align*}
Thus, after re-arranging we deduce that
\begin{equation}
    \label{sa3}
\begin{aligned}
    \frac{2T_0}{T}\delta_{T_0+1} &\leq \color{black}64\kappa\bL \frac{d}{T\alpha}\delta_1 + \frac{8\left(\cst_3+4\left(\cst_5+\cst_4{\color{black}d^{-1+\frac{4}{\beta}}T^{-\frac{2}{\beta}}}\right)\right)}{\min\{\alpha,\alpha^2\}}\left(\frac{d^2}{T}\right)^{\frac{\beta-1}{\beta}}.
\end{aligned}
\end{equation}
Again, since, by assumption, ${\color{black}T \geq d^{2-\frac{\beta}{2}}}$, it holds that ${\color{black}d^{-1+\frac{4}{\beta}}T^{-\frac{2}{\beta}}\leq 1}$ and by the combination of Eqs.~\eqref{sa2} and~\eqref{sa3} delivers
\begin{align*}
    \delta_T \leq \cst_7\frac{d}{T\alpha}\delta_3 + \frac{\cst_{2}}{\min\{\alpha, \alpha^2\}}\left(\frac{d^2}{T}\right)^{\frac{\beta-1}{\beta}},
\end{align*}
where ${\color{black}\cst_1 =\color{black}64\kappa\bL }$, and $\cst_2 = 12\left(\cst_3+4\left(2\cst_4+\cst_5\right)\right)$.



% \evg[inline]{Here I am lost}
\paragraph{Handling the case $T \leq T_0$.} The above analysis was performed under the assumption that $T > T_0$, to conclude, we need to complete the above derived bound for the case when $T \leq T_0.$ Eq~\eqref{oddca} and the fact that in this regime $h_t = \big(\frac{d^2}{T}\big)^{\frac{1}{2\beta}}$ imply
\begin{align*}
    \delta_{T+1}
    &\leq
    \delta_1 \left(1- \frac{2}{T_0+1}\right)^{T}+(4\cst_3+16\cst_4)\frac{d^{2-\frac{2}{\beta}}}{\min\{\alpha, \alpha^{2}\}}\sum_{t=1}^{T}\Big(\frac{1}{T}\Big)^{\frac{2\beta-1}{\beta}} +16\cst_5 \frac{{\color{black}d^{1+\frac{2}{\beta}}}}{\alpha^{2}}\sum_{t=1}^{T}\Big(\frac{1}{T}\Big)^{\frac{2\beta+1}{\beta}}\\
    &\leq
    \delta_1 \left(1- \frac{2}{T_0+1}\right)^{T}+ \frac{4\Big(\cst_3 + 4\big(\cst_4+\cst_5\big)\Big)}{\min(\alpha,\,\alpha^2)}\left(\frac{d^2}{T}\right)^{\frac{\beta-1}{\beta}},
\end{align*}
where the last inequality is obtained from the assumption ${\color{black}T \geq d^{2-\frac{\beta}{2}}}$.

Recall that for any $\rho, T> 0$, we have $(1 - \rho)^{T-2} \leq \exp(-\rho T) \leq \tfrac{1}{\rho T}$ and hence for $\rho = \tfrac{2}{T_0 + 1}$ we can write

\begin{align*}
    \delta_{T+1} &\leq \frac{T_0+1}{2T}\delta_3 +\frac{4\Big(\cst_3 + 4\big(\cst_4+\cst_5\big)\Big)}{\min(\alpha,\, \alpha^2)}\left(\frac{d^2}{T}\right)^{\frac{\beta-1}{\beta}}
    \leq
    2\cst_7\frac{d}{(T+1)\alpha}\delta_1 + \frac{\cst_2}{\min\{\alpha,\alpha^2\}}\left(\frac{d^2}{T+1}\right)^{\frac{\beta-1}{\beta}}\enspace,
\end{align*}

with the last inequality following from the definition of $T_0$, $T+1\leq 2T$, for any $T\geq 1.$

\end{proof}
\begin{comment}
\begin{proof}
[Proof of Theorem~\ref{plgoo:simplex} ($\ell_1$-randomization)] By Lemma \ref{lem:general}, we have
\begin{align*}
    \delta_{t+1} \leq \delta_{t}-\frac{\eta_t}{2}(1-\bar{L}\eta_{t}m)\Exp{[\norm{\nabla f(\bx_t)}^2]}+\frac{\eta_t}{2}(b_t^2+\bar{L}\eta_tv_t),
\end{align*}
where $\delta_t = \Exp[f(\bx_t)-f^{\star}]$ for all $t \geq 1$. For Algorithm \ref{algo:simplex}, by applying Lemmas \ref{lem:bias_simplex} and \ref{lem:var_simplex} we get
\begin{align*}
    \delta_{t+1} \leq \delta_t - \frac{\eta_t}{2}\left(1-8\bL\kappa d\eta_t\right)\Exp[\norm{\nabla f(\bx_t)}^2]+\cst_3h_t^{2(\beta-1)}d^{1-\beta}+\eta_t^2d\left(\cst_4h_t^2+\cst_5d^2h_t^{-2}\right),
\end{align*}
where $\cst_3 = \frac{(\kappa_\beta \ell L)^2}{2}$, $\cst_4 = 12\bL^3\kappa$, and $\cst_5 = \sigma^3\kappa$. Since $\eta_t \leq \frac{1}{16\bL\kappa d}$, we have $1-8\bL\kappa d\eta_t\leq \frac{1}{2}$. The latter with the fact that $f$ is an $\alpha$-gradient dominant function, yield 
\begin{align}\label{yur1}
    \delta_{t+1} \leq \delta_t\left(1-\frac{\eta_t\alpha}{2}\right)+\cst_3\eta_th_t^{2(\beta-1)}d^{1-\beta}+\eta_t^2d\left(\cst_4h_t^2+\cst_5d^2h_t^{-2}\right).
\end{align}
Recall that $T_0 = \floor{\frac{64\bL\kappa d}{\alpha}}$. From now on, we divide the proof into two cases. The first case is when $T \geq T_0$. Then for any $T_0+1\leq t \leq T$, we have $\eta_t = \frac{4}{\alpha t}$ and $h_t = d^{\frac{2+\beta}{2\beta}}t^{-\frac{1}{2\beta}}$. Substituting these terms in \eqref{yur1}, implies 
\begin{align*}
    \delta_{t+1} \leq \delta_t\left(1-\frac{2}{\alpha t}\right) + \left(4\cst_3+16\cst_5\right)\frac{d^{2-\frac{2}{\beta}}}{\min\{\alpha, \alpha^2\}}t^{-\frac{2\beta-1}{\beta}}+16\cst_4\frac{d^{2+\frac{2}{\beta}}}{\alpha^2}t^{-\frac{2\beta+1}{\beta}}.
\end{align*}
Now, by applying Lemma \ref{lemma:bisev} we have
\begin{align*}
    \delta_{T} \leq \frac{2T_0}{T}\delta_{T_0+1} + \frac{4\cst_3+16\cst_5+16\cst_4\left(\frac{d^2}{T}\right)^{\frac{2}{\beta}}}{\min\{\alpha, \alpha^2\}}\left(\frac{d^2}{T}\right)^{\frac{\beta-1}{\beta}}.
\end{align*}
Since $T\geq d^2$, we have $\left(\frac{d^2}{T}\right)^{\frac{2}{\beta}}\leq 1$, which implies
\begin{align}\label{yur2}
    \delta_{T} \leq \frac{2T_0}{T}\delta_{T_0+1} + \frac{4\left(\cst_3+4\cst_4+4\cst_5\right)}{\min\{\alpha, \alpha^2\}}\left(\frac{d^2}{T}\right)^{\frac{\beta-1}{\beta}},
\end{align}
Now, it is enough to bound the term $\delta_{T_0+1}$. If $T_0 = 0$, the proof is concluded. Otherwise, note that for $1\leq t\leq T_0$ we have $h_t = d^{\frac{2+\beta}{2\beta}}T^{-\frac{1}{2\beta}}$, $\eta_t = \frac{1}{16\bL\kappa d}$, and $\frac{4}{(T_0+1)\alpha}\leq \eta_t \leq \frac{4}{T_0\alpha}$. By substituting $h_t$ and $\eta_t$ in \eqref{yur1}, for $1\leq t\leq T_0$ we have
\begin{align}\label{yur3}
    \delta_{t+1} \leq \delta_t\left(1 - \frac{2}{T_0+1}\right)+\frac{4\cst_3}{T_0\alpha}\left(\frac{d^2}{T}\right)^{\frac{\beta-1}{\beta}} + \frac{16\cst_5}{T_0^2\alpha^2}d^{2-\frac{2}{\beta}}T^{\frac{1}{\beta}} + \frac{16\cst_4}{T_0^2\alpha^2}\left(\frac{d^2}{T}\right)^{\frac{1}{\beta}}d^{2-\frac{2}{\beta}}T^{\frac{1}{\beta}}.
\end{align}
Again since $T\geq d^2$, we have $\left(\frac{d^2}{T}\right)^{\frac{1}{\beta}}\leq 1$ and by \eqref{yur3} we can write
\begin{align*}
    \delta_{T_0+1} \leq \delta_1+\frac{4\cst_3}{\alpha}\left(\frac{d^2}{T}\right)^{\frac{\beta-1}{\beta}} +  \frac{16\left(\cst_4+\cst_5\right)}{T_0\alpha^2}d^{2-\frac{2}{\beta}}T^{\frac{1}{\beta}}.
\end{align*}
Therefore, for the term in r.h.s of \eqref{yur2} we get
\begin{align}\label{yur4}
    \frac{2T_0}{T}\delta_{T_0+1}\leq \frac{128\bL\kappa d}{\alpha T}\delta_1 + \frac{8\left(\cst_3+4\cst_4+4\cst_5\right)}{\min\{\alpha,\alpha^2\}}\left(\frac{d^2}{T}\right)^{\frac{\beta-1}{\beta}}.
\end{align}
By combining \eqref{yur2} and \eqref{yur4} we get
\begin{align*}
    \delta_T \leq \cst_1\frac{d}{\alpha T}\delta_1 + \frac{\cst_2}{\min\{\alpha,\alpha^2\}}\left(\frac{d^2}{T}\right)^{\frac{\beta-1}{\beta}},
\end{align*}
where $\cst_1 = 128\bL\kappa d$ and $\cst_2 = 12\left(\cst_3+4\cst_4+4\cst_5\right)$. Now, suppose that $T \leq T_0$. Then by \eqref{yur3}, we get
\begin{align*}
    \delta_{T+1}&\leq \delta_1\left(1 - \frac{2}{T_0+1}\right)^{T} +\frac{4\cst_3}{\alpha}\left(\frac{d^2}{T}\right)^{\frac{\beta-1}{\beta}} + \frac{16\cst_5}{T_0\alpha^2}d^{2-\frac{2}{\beta}}T^{\frac{1}{\beta}} + \frac{16\cst_4}{T_0\alpha^2}\left(\frac{d^2}{T}\right)^{\frac{1}{\beta}}d^{2-\frac{2}{\beta}}T^{\frac{1}{\beta}}
    \\&\leq \delta_1\left(1 - \frac{2}{T_0+1}\right)^{T} + \frac{4\left(\cst_3 + 4\cst_4+4\cst_5\right)}{\min\{\alpha,\alpha^2\}}\left(\frac{d^2}{T}\right)^{\frac{\beta-1}{\beta}},
\end{align*}
where the last inequality is obtained from $T \leq T_0$ and $T\geq d^2$. Since for any $\rho > 0$ we have $0<\rho<1$, $\rho^T \leq \frac{1}{\log(\frac{1}{\rho})T}\leq \frac{1-\rho}{T}$, we can write 
\begin{align*}
    \delta_{T+1}&\leq \frac{T_0+1}{2T}\delta_1+\frac{4\left(\cst_3 + 4\cst_4+4\cst_5\right)}{\min\{\alpha,\alpha^2\}}\left(\frac{d^2}{T}\right)^{\frac{\beta-1}{\beta}}
    \\&\leq \frac{T_0}{T}\delta_1 +\frac{4\left(\cst_3 + 4\cst_4+4\cst_5\right)}{\min\{\alpha,\alpha^2\}}\left(\frac{d^2}{T}\right)^{\frac{\beta-1}{\beta}}.
\end{align*}
Therefore, we obtain
\begin{align*}
    \delta_{T}\leq \cst_1\frac{d}{\alpha T}\delta_1 +\frac{\cst_2}{\min\{\alpha,\alpha^2\}}\left(\frac{d^2}{T}\right)^{\frac{\beta-1}{\beta}}\enspace.
\end{align*}
\end{proof}
\end{comment}
\begin{proof}
[Proof of Theorem~\ref{plgoo:simplex} ($\ell_1$-randomization)] By Lemma \ref{lem:general}, we have
\begin{align*}
    \delta_{t+1} \leq \delta_{t}-\frac{\eta_t}{2}(1-\bar{L}\eta_{t}m)\Exp{[\norm{\nabla f(\bx_t)}^2]}+\frac{\eta_t}{2}(b_t^2+\bar{L}\eta_tv_t)\enspace,
\end{align*}
where $\delta_t = \Exp[f(\bx_t)-f^{\star}]$ for all $t \geq 1$. For Algorithm \ref{algo:simplex}, by applying Lemmas \ref{lem:bias_simplex} (bias) and \ref{lem:var_l1_v2} (variance) we get
\begin{align*}
    \delta_{t+1} \leq \delta_t - \frac{\eta_t}{2}\left(1-{\color{black}87\bL d\kappa\eta_t}\right)\Exp[\norm{\nabla f(\bx_t)}^2]+\cst_3h_t^{2(\beta-1)}d^{1-\beta}+\eta_t^2\left(\cst_4h_t^2+\cst_5d^3h_t^{-2}\right)\enspace,
\end{align*}
where $\cst_3 = \frac{(\kappa_\beta \ell L)^2}{2}$, ${\color{black}\cst_4 = 428\bL^3\kappa}$, and ${\color{black}\cst_5 = \frac{\kappa \bL \sigma^2}{4}}$. Since, by its definition, ${\color{black}\eta_t \leq \frac{1}{174\bL d\kappa}}$, we have ${\color{black}1-87\bL d\kappa\eta_t\leq \frac{1}{2}}$, then the latter inequality, combined with the fact that $f$ is an $\alpha$-gradient dominant function yields
\begin{align}\label{yur1}
    \delta_{t+1} \leq \delta_t\left(1-\frac{\eta_t\alpha}{2}\right)+\cst_3\eta_th_t^{2(\beta-1)}d^{1-\beta}+\eta_t^2\left(\cst_4h_t^2+\cst_5d^3h_t^{-2}\right)\enspace.
\end{align}
Recall that ${\color{black}T_0 = \floor{\frac{696\bL d\kappa}{\alpha}}}$.
As in the previous proof we first assume that $T > T_0$ and split our analysis into two parts: for $t \in [T_0 + 1, T]$ and for $t \in [1, T_0]$.

\paragraph{Case 1: $t \in [T_0 + 1, T]$.} For any $t$ in this regime, we have $\eta_t = \frac{4}{\alpha t}$ and $h_t = d^{\frac{2+\beta}{2\beta}}t^{-\frac{1}{2\beta}}$. Substituting these terms in \eqref{yur1}, implies 
\begin{align*}
    \delta_{t+1} \leq \delta_t\left(1-\frac{2}{\alpha t}\right) + \left(4\cst_3+16\cst_5\right)\frac{d^{2-\frac{2}{\beta}}}{\min\{\alpha, \alpha^2\}}t^{-\frac{2\beta-1}{\beta}}+16\cst_4\frac{{\color{black}d^{1+\frac{2}{\beta}}}}{\alpha^2}t^{-\frac{2\beta+1}{\beta}}.
\end{align*}
Applying Lemma \ref{lemma:bisev}, to control the above recursive relation, we deduce that
\begin{align*}
    \delta_{T} \leq \frac{T_0}{T}\delta_{T_0+1} + \frac{4\cst_3+16\cst_5+32\cst_4{\color{black}\left(\frac{d^{4-\beta}}{T^2}\right)}^{\frac{1}{\beta}}}{\min\{\alpha, \alpha^2\}}\left(\frac{d^2}{T}\right)^{\frac{\beta-1}{\beta}},
\end{align*}
Since, we assumed that ${\color{black}T\geq d^{2-\frac{\beta}{2}}}$, we have ${\color{black}\left(\frac{d^{4-\beta}}{T^2}\right)}^{\frac{1}{\beta}}\leq 1$, which allows to simplify the above derived bound as
\begin{align}\label{yur2}
    \delta_{T} \leq \frac{T_0}{T}\delta_{T_0+1} + \frac{4\left(\cst_3+8\cst_4+4\cst_5\right)}{\min\{\alpha, \alpha^2\}}\left(\frac{d^2}{T}\right)^{\frac{\beta-1}{\beta}},
\end{align}
As before, it is enough to bound the term $\delta_{T_0+1}$. If $T_0 = 0$, the proof is concluded. 
\paragraph{Case 2: $t \in [1, T_0]$.}
Note that for $t$ in this regime, we have $h_t = d^{\frac{2+\beta}{2\beta}}T^{-\frac{1}{2\beta}}$, ${\color{black}\eta_t = \frac{1}{174\bL\kappa d}}$, and $\frac{4}{(T_0+1)\alpha}\leq \eta_t \leq \frac{4}{T_0\alpha}$. Substituting $h_t$ and $\eta_t$ into Eq.~\eqref{yur1}, for $1\leq t\leq T_0$
\begin{align}\label{yur3}
    \delta_{t+1} \leq \delta_t\left(1 - \frac{2}{T_0+1}\right)+\frac{4\cst_3}{T_0\alpha}\left(\frac{d^2}{T}\right)^{\frac{\beta-1}{\beta}} + \frac{16}{T_0 \alpha^2}\left(\cst_5 + \cst_4{\color{black}\left(\frac{d^{4-\beta}}{T^2}\right)^{\frac{1}{\beta}}}\right)d^{2-\frac{2}{\beta}}T^{\frac{1}{\beta}}\enspace.
\end{align}
Again since ${\color{black}T\geq d^{2-\frac{\beta}{2}}}$, we have ${\color{black}\left(\frac{d^{4-\beta}}{T^{2}}\right)^{\frac{1}{\beta}}}\leq 1$ and the above inequality (here we roughly bound $(1 - \tfrac{2}{T_0+1})$ by $1$) yields
\begin{align*}
    \delta_{T_0+1} \leq \delta_4+\frac{4\cst_3}{\alpha}\left(\frac{d^2}{T}\right)^{\frac{\beta-1}{\beta}} +  \frac{16\left(\cst_4+\cst_5\right)}{T_0\alpha^2}d^{2-\frac{2}{\beta}}T^{\frac{1}{\beta}}.
\end{align*}
Taking into account the above derived inequality and the definition of $T_0$, the first term on the right hand side of Eq.~\eqref{yur2} can be bounded as
\begin{align}\label{yur4}
    \frac{2T_0}{T}\delta_{T_0+1}\leq {\color{black}1392\bL\kappa\frac{d}{\alpha T}}\delta_4 + \frac{8\left(\cst_3+4\cst_4+4\cst_5\right)}{\min\{\alpha,\alpha^2\}}\left(\frac{d^2}{T}\right)^{\frac{\beta-1}{\beta}}.
\end{align}
The combination of Eq.~\eqref{yur2} and Eq.~\eqref{yur4} implies
\begin{align*}
    \delta_T \leq \cst_1\frac{d}{\alpha T}\delta_1 + \frac{\cst_2}{\min\{\alpha,\alpha^2\}}\left(\frac{d^2}{T}\right)^{\frac{\beta-1}{\beta}},
\end{align*}
where $\cst_1=1392\bL\kappa$ and $\cst_2 = 12\left(\cst_3+8\cst_4+4\cst_5\right)$.

\paragraph{Handling the case of $T \leq T_0$.} To finish the proof, we study separately the case of $T \leq T_0$. Unfolding the recursion in Eq.~\eqref{yur3}, we get
\begin{align*}
    \delta_{T+1}&\leq \delta_1\left(1 - \frac{2}{T_0+1}\right)^{T} +\frac{4\cst_3}{\alpha}\left(\frac{d^2}{T}\right)^{\frac{\beta-1}{\beta}} + \frac{16\cst_5}{T_0\alpha^2}d^{2-\frac{2}{\beta}}T^{\frac{1}{\beta}} + \frac{16\cst_4}{T_0\alpha^2}{\color{black}\left(\frac{d^{4-\beta}}{T^2}\right)^{\frac{1}{\beta}}}d^{2-\frac{2}{\beta}}T^{\frac{1}{\beta}}
    \\&\leq \delta_1\left(1 - \frac{2}{T_0+1}\right)^{T} + \frac{4\left(\cst_3 + 4\cst_4+4\cst_5\right)}{\min\{\alpha,\alpha^2\}}\left(\frac{d^2}{T}\right)^{\frac{\beta-1}{\beta}},
\end{align*}
where the last inequality is obtained from $T \leq T_0$ and $T\geq d^{2 - \frac{\beta}{2}}$. 
From here we conclude identically to the proof of Theorem~\ref{plgoo}.
% \begin{align*}
%     \delta_{T+1}&\leq \frac{T_0+1}{2T}\delta_1+\frac{4\left(\cst_3 + 4\cst_4+4\cst_5\right)}{\min\{\alpha,\alpha^2\}}\left(\frac{d^2}{T}\right)^{\frac{\beta-1}{\beta}}
%     \\&\leq \frac{T_0}{T}\delta_1 +\frac{4\left(\cst_3 + 4\cst_4+4\cst_5\right)}{\min\{\alpha,\alpha^2\}}\left(\frac{d^2}{T}\right)^{\frac{\beta-1}{\beta}}.
% \end{align*}
% Therefore, we obtain
% \begin{align*}
%     \delta_{T}\leq \cst_1\frac{d}{\alpha T}\delta_1 +\frac{\cst_2}{\min\{\alpha,\alpha^2\}}\left(\frac{d^2}{T}\right)^{\frac{\beta-1}{\beta}}.
% \end{align*}
\end{proof}
{
% \color{black}
\newpage
\section{Upper bounds: strongly convex functions}

\begin{proof}[Proof of Lemma~\ref{scuntunc}]
Recall that we denote by $\Exp_t[\cdot] = \Exp[\cdot \mid \bx_t]$.
For any $\bx \in \com$, by the definition of Algorithm \ref{algose}, we have 
\begin{align}\label{nl1}
    \norm{\bx_{t+1}-\bx}^2 = \norm{\proj_{\com}\big(\bx_{t} - \eta_t\bg_t\big) - \bx}^2 \leq \norm{\bx_t - \eta_t\bg_{t} - \bx}^2\enspace,
\end{align}
where the above inequality is obtained from the definition of Euclidean projection on the set $\com$ and the fact that $\bx \in \com$. It is clear that (\ref{nl1}) is equivalent to 
\begin{align}\label{nl2}
    \langle \bg_t, \bx_t - \bx \rangle \leq \frac{\norm{\bx_t - \bx}^2-\norm{\bx_{t+1}-\bx}^2}{2\eta_t}+\frac{\eta_t}{2}\norm{\bg_t}^2\enspace.
\end{align}
On the other hand, since $f$ is a strongly function on $\com$, we have
\begin{align}\label{nl3}
    f(\bx_t) - f(\bx) \leq \langle \nabla f(\bx_t), \bx_t -\bx \rangle -\frac{\alpha}{2}\norm{\bx_t -\bx}^2\enspace.
\end{align}
Combining Eq.~(\ref{nl2}) with Eq.~(\ref{nl3}) and denoting $a_t = \norm{\bx_t - \bx}^2$, we deduce that
\begin{align}\nonumber
    \Exp_t[f(\bx_t) - f(\bx)] &\leq \norm{\Exp_t[\bg_t] - \nabla f(\bx_t)}\norm{\bx_t-\bx} + \frac{1}{2\eta_t}\Exp_t[a_t-a_{t+1}]+\frac{\eta_t}{2}\Exp_t\norm{\bg_t}^{2}-\frac{\alpha}{2}\Exp_t[a_t]\\\label{nl4}&\leq b_t\norm{\bx_t-\bx}+\frac{1}{2\eta_t}\Exp_t[a_{t} - a_{t+1}] + \frac{\eta_t}{2}\Big(v_t+m\|\nabla f(\bx_t)\|^2\Big) - \frac{\alpha}{2}\Exp_t[a_t]\enspace,
\end{align}
Since $2ab\leq a^2+b^2$, we can write
\begin{align}\label{nl5}
    b_t\norm{\bx_t - \bx} \leq \frac{b_t^2}{\alpha}+\frac{\alpha}{4}\norm{\bx_t-\bx}^2\enspace.
\end{align}
Replacing (\ref{nl5}) in (\ref{nl4}), setting $r_t = \Exp[a_t]$ and taking total expectation from both sides of (\ref{nl4}), yield
\begin{align*}
    \Exp[f(\bx_t)-f(\bx)]\leq \frac{r_t-r_{t+1}}{2\eta_t}-\frac{\alpha}{4}r_t+\frac{b_{t}^2}{\alpha}+\frac{\eta_t}{2}\big(v_t+m\Exp\|\nabla f (\bx_t)\|^2\big)\enspace.
\end{align*}


% With the similar steps as in the proof of Lemma \ref{scunt}, we get
% \begin{align*}
%     \Exp[f(\bx_t)-f^{\star}] &\leq \frac{r_t - r_{t+1}}{2\eta_t}-r_t\left(\frac{\alpha}{4}-\frac{\eta_t}{2}m\right)+\frac{b_t^2}{\alpha}+\frac{\eta_t}{2}v_t,
% \end{align*}
% where $r_t = \Exp\norm{x_t -x^*}^2$ for $t= 1, \dots, T$. Since $\eta_t = \min\big(\frac{\alpha}{4m},\frac{4}{\alpha t}\big)$, we have $\frac{\eta_{t}}{2}m\leq \frac{\alpha}{8}$ and we can write
% \begin{align}\label{ma1}
%     \Exp[f(\bx_t)-f^{\star}] &\leq \frac{r_t - r_{t+1}}{2\eta_t} - \frac{\alpha}{8}r_t + \frac{b_t^2}{\alpha} + \frac{\eta_t}{2}v_t\enspace.
% \end{align}
% Let us introduce $T_0 = \floor{\tfrac{16m}{\alpha^2}}$---the moment when $\eta_t$ switches from $\tfrac{\alpha}{4 m}$ to $\tfrac{4}{\alpha t}$.
% Summing the above inequality over $t = 1, \ldots, T$ we obtain
% \begin{align*}
%     \sum_{t = 1}^t\Exp[f(\bx_t)-f^{\star}]
%     &\leq
%     \parent{\underbrace{\sum_{t = 1}^{T_0}}_{=: \texttt{T}_2} + \underbrace{\sum_{t = T_0 + 1}^T}_{:=\texttt{T}_1}}\parent{\frac{r_t - r_{t+1}}{2\eta_t} - \frac{\alpha}{8}r_t + \frac{b_t^2}{\alpha} + \frac{\eta_t}{2}v_t}\enspace.
% \end{align*}
% In what follows we provide an upper bound on the term appearing on the right hand side of the above inequality. To do so, we partition the summation $\sum_{t = 1}^T$ into two parts: $\texttt{T}_1 = \sum_{t = T_0 + 1}^{T} (\ldots)$ and $\texttt{T}_2 = \sum_{t = 1}^{T_0}(\ldots)$.
% Note that in this part of the proof we explicitly assume that $T > T_0$ and we deal with the complement situation later in the proof.

% \paragraph{Bound on $\texttt{T}_1$.}
% In this regime of $t$ we have $\eta_t = \frac{4}{\alpha t}$.
% Substituting this value into the definition of $\texttt{T}_1$ we obtain
% \begin{equation}
% \label{ma2}
% \begin{aligned}
%     \texttt{T}_1
%     &=
%     \frac{\alpha}{8}\sum_{t=T_{0}+1}^{T}\Big((r_t - r_{t+1})t -r_t\Big) + \frac{1}{\alpha}\sum_{t= T_{0}+1}^{T}\Big(b_t^2 + \frac{2}{t}v_t\Big)
%     \\
%     &\leq
%     \frac{\alpha}{8}T_{0}r_{T_{0}+1} + \frac{1}{\alpha}\sum_{t= T_{0}+1}^{T}\Big(b_t^2 + \frac{2}{t}v_t\Big).
% \end{aligned}
% \end{equation}
% It remains to provide an upper bound for the term $r_{T_{0}+1}$. If $T_0 =0$, the proof can be concluded by convexity of $f$. Otherwise, from Eq.~\eqref{ma1} and using the fact that $f(\bx_t) - f^{\star} \geq 0$, we deduce that
% \begin{align*}
%     r_{t+1} \leq r_{t} +2\eta_t\frac{b_{t}^2}{\alpha}+\eta_t^2v_t\enspace,
% \end{align*}
% for $t = 1, \dots, T$. Substituting $\eta_{t} = \min\big(\frac{\alpha}{4m},\frac{4}{\alpha t}\big)$ and using $\eta_{t}^2 \leq \frac{1}{m t}$, we get
% \begin{align*}
%     r_{t+1} &\leq r_{t} + \frac{1}{2m}\Big(b_t^2+ \frac{2}{t}v_t\Big).
% \end{align*}
% Therefore, unfolding the above recursion, we deduce that
% \begin{align}\label{ma3}
%     r_{T_{0}+1} &\leq r_{1} + \frac{1}{2m}\sum_{t=1}^{T_{0}}\Big(b_t^2+ \frac{2}{t}v_t\Big).
% \end{align}
% Substituting the bound derived in Eq.~\eqref{ma3} into Eq.~\eqref{ma2} we get
% \begin{align}\nonumber
%     \sum_{t= T_{0}+1}^{T}\Exp[f(\bx_t)-f^{\star}] &\leq \frac{2m}{\alpha}r_1 + \frac{1}{\alpha}\sum_{t=1}^{T}\Big(b_t^2 + \frac{2}{t}v_t\Big).
% \end{align}
% Since $\alpha \geq 4\bar{L}\sqrt{\frac{2m}{T}}$, we have $T_{0}\leq \frac{T}{2}$. Together with convexity of $f$, implies
% \begin{align}\nonumber
%     \Exp[f(\bar{\bx}_{T_{0},T})-f^{\star}] &\leq \frac{4m}{\alpha T}r_1 + \frac{2}{\alpha T}\sum_{t=1}^{T}\Big(b_t^2 + \frac{2}{t}v_t\Big).
% \end{align}
\end{proof}



\section{Unconstrained optimization}
\begin{proof}[Proof of Theorem~\ref{thm:sconvex_l2_uncons} ($\ell_2$-randomization)] 
Note that since $f \in \class{F}_2(\bL)$ and $\com = \bbR^d$, then $\norm{\nabla f (\bx_t)} \leq \bL \norm{\bx_t - x^*}$.
Hence, by using Lemma \ref{scuntunc}, for all $t \geq 1$ we have

\begin{align*}
    \Exp[f(\bx_t) - f^{\star}] \leq \frac{r_t - r_{t+1}}{2\eta_t} - r_t\left(\frac{\alpha}{4} - \frac{\eta_t}{2}\bL^2 m\right) + \frac{b_t^2}{\alpha} + \frac{\eta_t}{2}v_t\enspace.
\end{align*}
Using Lemma~\ref{lem:bias_sphere} (bound on the bias) and Lemma~\ref{lem:var_sphere_v2} (bound on the variance), we deduce that 
% \evg[inline]{Here should be $\bL^2$ in $4\eta_t d \kappa c\bL$! Right?}
\begin{align*}
    \Exp[f(\bx_t) - f^{\star}] \leq \frac{r_t - r_{t+1}}{2\eta_t} - r_t\left(\frac{\alpha}{4}-{\color{black}2\eta_td\kappa \bL^2} \right)+\cst_3\frac{h_t^{2(\beta-1)}}{\alpha} + \eta_td^2\left(\cst_4{\color{black}d^{-1}}h_t^2+\cst_5h_t^{-2}\right)\enspace,
\end{align*}
where $\cst_3=\left(\kappa_\beta \frac{L}{\left(\ell-1\right)!}\right)^2$, ${\color{black}\cst_4 = 2\kappa\bL^2}$, and ${\color{black}\cst_5 = \frac{\kappa\sigma^2}{4}}$. Since, by definition, ${\color{black}\eta_t \leq \frac{\alpha}{16 d\kappa \bL^2}}$, then we have $\frac{\alpha}{4} - {\color{black}2\eta_td\kappa\bL^2}\geq\frac{\alpha}{8}$ and the above inequality is simplified as
\begin{align}\label{generalscuns}
    \Exp[f(\bx_t) - f^{\star}] \leq \frac{r_t - r_{t+1}}{2\eta_t} -\frac{\alpha}{8}r_t+\cst_3\frac{h_t^{2(\beta-1)}}{\alpha} + \eta_td^2\left(\cst_4{\color{black}d^{-1}}h_t^2+\cst_5h_t^{-2}\right)\enspace.
\end{align}
Recall that ${\color{black}T_0 = \floor{\frac{64d\kappa\bL^2}{\alpha^2}}}$---the moment when $\eta_t$ changes its behaviour. Let us first assume that $T_0<T$ and provide the proof for this case. The case of $T \leq T_0$ will be treated separately, in the end of the present proof.
As for all other cases, we partition the proof into two parts, analysing the regimes: $t \in [T_0 +1 , T]$ and $T \in [1, T_0]$.
The case distinguishing is slightly different for this proof compared to the previous proofs.
By convexity of $f$, we have
\begin{align}
\label{eq:strongly_convex_l2_1}
    f(\bar{\bx}_T) - f^{\star} \leq \frac{1}{T}\sum_{t = 1}^T(f(\bx_t) - f^\star) = \frac{1}{T}\underbrace{\sum_{t = T_0 + 1}^{T}(f(\bx_t) - f^\star)}_{\text{case 1}} + \frac{1}{T}\underbrace{\sum_{t = 1}^{T_0}(f(\bx_t) - f^\star)}_{\text{case 2}} \enspace.
\end{align}


\paragraph{Case 1: $t \in [T_0 +1 , T]$.}
For any $T_0 +1\leq t \leq T$, we have $\eta_t = \frac{4}{\alpha t}$ and $h_t = \left(\frac{d^2}{t}\right)^{\frac{1}{2\beta}}$. Summing both side of \eqref{generalscuns} from $T_0+1$ to $T$, and substituting $\eta_t$ and $h_t$, we deduce that

\begin{align*}
    \sum_{t=T_0+1}^{T}\Exp[f(\bx_t) - f^{\star}] \leq
    \underbrace{\frac{\alpha}{8}\sum_{t=T_0+1}^{T}\left( \left(r_t -r_{t+1}\right)t -r_t\right)}_{=:\tT_1}
    &+
    \underbrace{\frac{\cst_3+4\cst_5}{\alpha}\sum_{t=T_0+1}^{T}\left(\frac{d^2}{t}\right)^{\frac{\beta-1}{\beta}}}_{=:\tT_2}\\
    &+
    \underbrace{ \frac{4\cst_4}{\alpha }{\color{black}d^{1+\frac{2}{\beta}}}\sum_{t=T_0+1}^{T}t^{-\frac{1}{\beta}-1}}_{=:\tT_3}\enspace,
\end{align*}
where we defined $\tT_1, \tT_2,$ and $\tT_3$.

It is straightforward to see that $\tT_1 \leq \tfrac{\alpha}{8} T_0 r_{T_0+1}$ (the summation, involved in $\tT_1$, is telescoping). For $\tT_2$ we can write
\begin{align*}
    \tT_2 
    \leq \frac{\cst_3 + 4\cst_5}{\alpha}d^{2-\frac{2}{\beta}}\sum_{t=1}^{T}t^{-\frac{\beta-1}{\beta}}
    \leq \frac{\beta\left(\cst_3 + 4\cst_5\right)}{\alpha}d^{2-\frac{2}{\beta}}T^{\frac{1}{\beta}}\enspace.
\end{align*}
{\color{black}
Furthermore, for the term $\tT_3$ we have
\begin{align*}
    \tT_3
    \leq \frac{4\cst_4}{\alpha }d^{1+\frac{2}{\beta}}\sum_{t=T_0+1}^{T}t^{-\frac{1}{\beta}-1}
    &\leq \frac{4\cst_4}{\alpha }d^{1+\frac{2}{\beta}}\left(\parent{T_0 + 1}^{-\frac{1}{\beta}-1} + \int_{T_0}^{T} t^{-\frac{1}{\beta}-1} \d t\right)\\
    &\leq \frac{4\cst_4}{\alpha }d^{1+\frac{2}{\beta}}\left(\parent{T_0 + 1}^{-\frac{1}{\beta}-1} + \beta {T_0}^{-\frac{1}{\beta}}\right)\\
    &\leq \frac{4(\beta+1)\cst_4}{\alpha }d^{1+\frac{2}{\beta}} {T_0}^{-\frac{1}{\beta}}\\
    &\leq \frac{4(\beta+1)\cst_4}{\alpha }d^{1+\frac{1}{\beta}} \frac{\alpha^{\frac{2}{\beta}}}{(64\kappa\bL^2)^{\frac{1}{\beta}}}\\
    &\leq \frac{\cst_{6}}{\alpha}d^{1+\frac{1}{\beta}}
    \leq \frac{\cst_{6}}{\alpha}d^{2-\frac{2}{\beta}}T^{\frac{1}{\beta}},
\end{align*}
where $\cst_6 = \frac{4(\beta+1)\cst_4}{(64\kappa)^{\frac{1}{\beta}}}$, and the two last inequalities are obtained from the fact that $\alpha \leq \bL$, $\beta \geq 2$ and $d^{2-\frac{\beta}{2}}\leq T$.}
Combining the bounds on $\tT_1, \tT_2$, and $\tT_3$ we obtain
\begin{align}\label{sfar1}
    \sum_{t=T_0+1}^{T}\Exp[f(\bx_t)-f^{\star}] \leq \frac{\alpha}{8}T_0r_{T_0+1} + \frac{\cst_7}{\alpha}d^{2-\frac{2}{\beta}}T^{\frac{1}{\beta}}\enspace, 
\end{align}
where $\cst_7 = \beta(\cst_3+4\cst_4) +\cst_6$. If $T_0=0$ then the proof is concluded by convexity of $f$ and the imposed assumption that $T_0<T$. Otherwise, for the term $r_{T_0+1}$, Eq.~\eqref{generalscuns} implies that for $1 \leq t \leq T_0$ 
\begin{align*}
    r_{t+1} \leq r_t + 2\cst_3 \eta_t \frac{h_t^{2(\beta-1)}}{\alpha} + 2\eta_t^2d^2\left(\cst_4{\color{black}d^{-1}}h_t^2+\cst_5h_t^{-2}\right)\enspace.
\end{align*}
In addition, for $1\leq t\leq T_0$ we have ${\color{black}\eta_t = \frac{\alpha}{16d\kappa \bL}}$ and $\eta_t\leq \frac{4}{\alpha T_0}$. Therefore, unfolding the above recursion we get
\begin{align*}
    r_{T_0+1}\leq r_1 + \sum_{t=1}^{T_0}\left(\frac{8\cst_3}{ T_0}\frac{h_t^{2(\beta-1)}}{\alpha^2} + \frac{32}{\alpha^2 T_0^2}d^{2}\left(\cst_4{\color{black}d^{-1}}h_t^2+\cst_5h_t^{-2}\right)\right)\enspace.
\end{align*}
Plugging in $h_t = \left(\frac{d^2}{T}\right)^{\frac{1}{2\beta}}$, yields
\begin{align*}
    r_{T_0+1} \leq r_1 + \frac{8\cst_3}{\alpha^{2}}\left(\frac{d^2}{T}\right)^{\frac{\beta-1}{\beta}}+\frac{32\cst_4}{\alpha^2T_0}\left({\color{black}\frac{d^{4 - \beta}}{T^{2}}}\right)^{\frac{1}{\beta}}d^{2-\frac{2}{\beta}}T^{\frac{1}{\beta}} + \frac{32\cst_5}{\alpha^{2}T_0}d^{2-\frac{2}{\beta}}T^{\frac{1}{\beta}}\enspace.
\end{align*}
Again, since we assumed that ${\color{black}T \geq d^{2-\frac{\beta}{2}}}$, then we have $\left({\color{black}\frac{d^{4 - \beta}}{T^{2}}}\right)^{\frac{1}{\beta}}\leq 1$ and the first term on the right hand side of Eq.~\eqref{sfar1} can be bounded as
\begin{align}\label{sfar2}
    \frac{\alpha}{8} T_0 r_{T_0+1}\leq {\color{black}8}\kappa\bL^2\frac{d}{\alpha}r_1 + \frac{\cst_3T_0}{\alpha }\left(\frac{d^2}{T}\right)^{\frac{\beta-1}{\beta}} + \frac{4\left(\cst_4+\cst_5\right)}{\alpha}d^{2-\frac{2}{\beta}}T^{\frac{1}{\beta}}\enspace.
\end{align}
Substituting the bound in Eq.~\eqref{sfar2} into Eq.~\eqref{sfar2}, we deduce that
\begin{align}\label{sfar3}
    \sum_{t=T_0+1}^{T}\Exp[f(\bx_t)-f^{\star}] \leq {\color{black}8}\kappa \bL^2\frac{d}{\alpha}r_1 +\frac{\cst_3T_0}{\alpha }\left(\frac{d^2}{T}\right)^{\frac{\beta-1}{\beta}}+\frac{\cst_8}{\alpha}d^{2-\frac{2}{\beta}}T^{\frac{1}{\beta}}\enspace, 
\end{align}
where $\cst_8 = 4\left(\cst_4+\cst_5\right)+\cst_7.$


\paragraph{Case 2: $t \in [1 , T_0]$.} Note that $\frac{4}{\alpha(T_0+1)}\leq \eta_t$. Then, summing \eqref{generalscuns} from $1$ to $T_0$ we have
% \begin{equation}
\begin{align}
    \sum_{t=1}^{T_0} \Exp[f(\bx_t) -f^{\star}] 
    &\leq \frac{\alpha (T_0+1)}{8}r_1 + \frac{\cst_3T_0}{\alpha}d^{2-\frac{2}{\beta}}T^{-\frac{\beta-1}{\beta}} +\sum_{t=1}^{T_0} \frac{4}{T_0\alpha}\left(\cst_4\left({\color{black}\frac{d^{4 - \beta}}{T^{2}}}\right)^{\frac{1}{\beta}}+\cst_5\right)d^{2-\frac{2}{\beta}}T^{\frac{1}{\beta}}\nonumber
    \\&\leq \frac{\alpha T_0}{4}r_1 + \frac{\cst_3T_0}{\alpha}d^{2-\frac{2}{\beta}}T^{-\frac{\beta-1}{\beta}} + \frac{4\left(\cst_4+\cst_5\right)}{\alpha}d^{2-\frac{2}{\beta}}T^{\frac{1}{\beta}}\enspace,\label{sfar4}
\end{align}
where in the last inequality we used the assumption $T \geq d^{2 - \frac{\beta}{2}}$.
% \end{equation}

As indicated in Eq.~\eqref{eq:strongly_convex_l2_1} at the beginning of the proof, we sum up the two studied cases---Eq.~\eqref{sfar3} and Eq.~\eqref{sfar4}---to deduce that
% \begin{align*}
%     \sum_{t=1}^{T}\Exp[f(\bx_t)-f^{\star}]\leq \cst_1\frac{d}{\alpha}r_1 + \frac{3\cst_3T_0}{2\alpha}d^{2-\frac{2}{\beta}}T^{-\frac{\beta-1}{\beta}} + \frac{\cst_9}{\alpha}d^{2-\frac{2}{\beta}}T^{\frac{1}{\beta}},
% \end{align*}
\begin{align*}
    \Exp[f(\bar{\bx}_T)-f^{\star}] \leq \cst_1\frac{d}{\alpha T}r_1+\frac{1}{\alpha}\left(\frac{3\cst_3}{2}\left(\frac{T_0}{T}\right)+\cst_9\right)\left(\frac{d^2}{T}\right)^{\frac{\beta-1}{\beta}}\enspace,
\end{align*}
where $\cst_1 = 54\kappa\bL$ and $\cst_9 = 20\left(\cst_4+\cst_5\right) + \cst_7$.


Since in thi part of the proof we assume that $T_0<T$, then we have $\frac{T_0}{T}<1$ and the proof is concluded by letting $\cst_2 = \frac{3\cst_3}{2}+\cst_9$.


\paragraph{Handling the case $T \leq T_0$.} Finally, we establish the result for $T \leq T_0$. Eq.~\eqref{generalscuns} yields
\begin{align*}
    \sum_{t=1}^{T}\Exp[f(\bx_t) - f^{\star}] 
    &\leq \frac{r_1}{2\eta_1} + \frac{\cst_3T}{\alpha}\left(\frac{d^2}{T}\right)^{\frac{\beta-1}{\beta}} + \eta_1T\left(\cst_4\left({\color{black}\frac{d^{4 - \beta}}{T^{2}}}\right)^{\frac{1}{\beta}}+\cst_5\right)d^{2-\frac{2}{\beta}}T^{\frac{1}{\beta}}
    \\&\leq \frac{T_0+1}{8}r_1 + \frac{\cst_3T}{\alpha}\left(\frac{d^2}{T}\right)^{\frac{\beta-1}{\beta}}+\frac{4T\left(\cst_4+\cst_5\right)}{T_0\alpha}d^{2-\frac{2}{\beta}}T^{\frac{1}{\beta}}
    \\&\leq \frac{T_0}{4}r_1 + \frac{\cst_3T}{\alpha}\left(\frac{d^2}{T}\right)^{\frac{\beta-1}{\beta}}+\frac{4\left(\cst_4+\cst_5\right)}{\alpha}d^{2-\frac{2}{\beta}}T^{\frac{1}{\beta}}
    \\&\leq {\color{black}32}\kappa\bL\frac{d}{\alpha}r_1 + \frac{T}{\alpha}\left(\cst_3+4\left(\cst_4 +\cst_5\right)\right)\left(\frac{d^2}{T}\right)^{\frac{\beta-1}{\beta}}\enspace,
\end{align*}
where we again utilized the assumption that $T \geq d^{2 - \frac{\beta}{2}}$.
The proof is concluded by convexity of $f$, with ${\color{black}\cst_1 = 32\kappa\bL}$ and $\cst_2 = \cst_3+4\left(\cst_4+\cst_5\right)$.
\end{proof}
\begin{proof}[Proof of Theorem~\ref{thm:sconvex_l1_uncons} ($\ell_1$-randomization)] By applying Lemma \ref{scuntunc}, for all $t \geq 1$ we have
\begin{align*}
    \Exp\left[f(\bx_t) - f^{\star}\right] \leq \frac{r_t-r_{t+1}}{2\eta_t} -r_t\left(\frac{\alpha}{4} - \frac{\eta_t}{2}\bL^2 m\right) + \frac{b_t^2}{\alpha}+\frac{\eta_t}{2}v_t.
\end{align*}
Using Lemma \ref{lem:bias_simplex} (bias) and Lemma \ref{lem:var_l1_v2} (variance), implies
\begin{align*}
    \Exp\left[f(\bx_t) - f^\star\right] \leq \frac{r_t-r_{t+1}}{2\eta_t} -r_t\left(\frac{\alpha}{4} - 43.5\eta_td\kappa\bL^2 \right) +\cst_3\frac{h_t^{2(\beta-1)}}{\alpha}d^{1-\beta}+\cst_4\eta_th_t^2+\cst_5\eta_td^3h_{t}^{-2},
\end{align*}
where $\cst_3 = \kappa_\beta \ell \bL$, $\cst_4 = 428\kappa\bL$, and $\cst_5 = \frac{\sigma^2\kappa}{4}$. Since $\eta_t \leq \frac{\alpha}{348 d\kappa \bL^2}$, we have $\frac{\alpha}{4} - 43.5\eta_t d\kappa \bL^2 \geq \frac{\alpha}{8}$ and the above inequality can be written as 
\begin{align}\label{generalscuns_l1}
    \Exp\left[f(\bx_t) - f^\star\right] \leq \frac{r_t-r_{t+1}}{2\eta_t} -\frac{\alpha}{8}r_t +\cst_3\frac{h_t^{2(\beta-1)}}{\alpha}d^{1-\beta}+\cst_4\eta_th_t^2+\cst_5\eta_td^3h_{t}^{-2}.
\end{align}
Recall that ${\color{black}T_0 = \floor{\frac{1392d\kappa\bL^2}{\alpha^2}}}$---the moment when $\eta_t$ and $h_t$ change their behaviour. First we assume that $T_0 < T$. for this regime, since $f$ is a convex function, we have 
\begin{align}
\label{eq:strongly_convex_l1_1}
    f(\bar{\bx}_T) - f^{\star} \leq \frac{1}{T}\sum_{t = 1}^T(f(\bx_t) - f^\star) = \frac{1}{T}\underbrace{\sum_{t = T_0 + 1}^{T}(f(\bx_t) - f^\star)}_{\text{case 1}} + \frac{1}{T}\underbrace{\sum_{t = 1}^{T_0}(f(\bx_t) - f^\star)}_{\text{case 2}} \enspace.
\end{align}
\paragraph{Case 1: $t \in [T_0 +1 , T]$.} For any $t \in [T_0, T]$, we have $\eta_t = \frac{4}{\alpha t}$ and $h_t = d^{\frac{2+\beta}{2\beta}}t^{-\frac{1}{2\beta}}$. By summing up both sides of Eq.~\eqref{generalscuns_l1} from $T_0$ to $T$, we get 
\begin{align*}
    \sum_{t=T_0+1}^{T}\Exp[f(\bx_t) - f^{\star}] \leq
    \underbrace{\frac{\alpha}{8}\sum_{t=T_0+1}^{T}\left( \left(r_t -r_{t+1}\right)t -r_t\right)}_{=:\tT_1}
    &+
    \underbrace{\frac{\cst_3+4\cst_5}{\alpha}\sum_{t=T_0+1}^{T}\left(\frac{d^2}{t}\right)^{\frac{\beta-1}{\beta}}}_{=:\tT_2}\\
    &+
    \underbrace{ \frac{4\cst_4}{\alpha }{\color{black}d^{1+\frac{2}{\beta}}}\sum_{t=T_0+1}^{T}t^{-\frac{1}{\beta}-1}}_{=:\tT_3}\enspace,
\end{align*}
where we introduced $\tT_1, \tT_2,$ and $\tT_3$.

It is straightforward to check that $\tT_1 \leq \tfrac{\alpha}{8} T_0 r_{T_0+1}$. For $\tT_2$ we can write
\begin{align*}
    \tT_2 
    \leq \frac{\cst_3 + 4\cst_5}{\alpha}d^{2-\frac{2}{\beta}}\sum_{t=1}^{T}t^{-\frac{\beta-1}{\beta}}
    \leq \frac{\beta\left(\cst_3 + 4\cst_5\right)}{\alpha}d^{2-\frac{2}{\beta}}T^{\frac{1}{\beta}}\enspace.
\end{align*}
{\color{black}
Furthermore, for the term $\tT_3$ we have
\begin{align*}
    \tT_3
    \leq \frac{4\cst_4}{\alpha }d^{1+\frac{2}{\beta}}\sum_{t=T_0+1}^{T}t^{-\frac{1}{\beta}-1}
    &\leq \frac{4\cst_4}{\alpha }d^{1+\frac{2}{\beta}}\left(\parent{T_0 + 1}^{-\frac{1}{\beta}-1} + \int_{T_0}^{T} t^{-\frac{1}{\beta}-1} \d t\right)\\
    &\leq \frac{4\cst_4}{\alpha }d^{1+\frac{2}{\beta}}\left(\parent{T_0 + 1}^{-\frac{1}{\beta}-1} + \beta {T_0}^{-\frac{1}{\beta}}\right)\\
    &\leq \frac{4(\beta+1)\cst_4}{\alpha }d^{1+\frac{2}{\beta}} {T_0}^{-\frac{1}{\beta}}\\
    &\leq \frac{4(\beta+1)\cst_4}{\alpha }d^{1+\frac{1}{\beta}} \frac{\alpha^{\frac{2}{\beta}}}{(1392\kappa\bL^2)^{\frac{1}{\beta}}}\\
    &\leq \frac{\cst_{6}}{\alpha}d^{1+\frac{1}{\beta}}
    \leq \frac{\cst_{6}}{\alpha}d^{2-\frac{2}{\beta}}T^{\frac{1}{\beta}},
\end{align*}
where $\cst_6 = \frac{4(\beta+1)\cst_4}{(1392\kappa)^{\frac{1}{\beta}}}$, and the two last inequalities are obtained from the fact that $\alpha \leq \bL$, $\beta \geq 2$ and $d^{2-\frac{\beta}{2}}\leq T$.} 
By combining the bounds on $\tT_1, \tT_2$, and $\tT_3$ we deduce that 
\begin{align}\label{sfar1_l1}
    \sum_{t=T_0+1}^{T}\Exp[f(\bx_t)-f^{\star}] \leq \frac{\alpha}{8}T_0r_{T_0+1} + \frac{\cst_7}{\alpha}d^{2-\frac{2}{\beta}}T^{\frac{1}{\beta}}\enspace, 
\end{align}
where $\cst_7 = \beta(\cst_3+4\cst_4) +\cst_6$. If $T_0=0$ then the proof is concluded by Eq.~\eqref{eq:strongly_convex_l1_1}. Otherwise, we need to provide an upper bound for the term $r_{T_0+1}$ appeared in Eq.~\eqref{sfar1_l1}. By Eq.~\eqref{generalscuns_l1}, for any $t \in [1, T_0]$, we can write
\begin{align*}
    r_{t+1} \leq r_t + 2\cst_3\eta_t\frac{h_t^{2(\beta-1)}}{\alpha}d^{1-\beta}+2\eta_t^2\left(\cst_4h_t^2+\cst_5d^3h_{t}^{-2}\right)\enspace.
\end{align*}
Therefore,
\begin{align*}
    r_{T_0+1} \leq r_1 + \sum_{t=1}^{T_0}\left(2\cst_3\eta_t\frac{h_t^{2(\beta-1)}}{\alpha}d^{1-\beta}+2\eta_t^2\left(\cst_4h_t^2+\cst_5d^3h_{t}^{-2}\right)\right)\enspace.
\end{align*}
Furthermore, plugging in $\eta_t \leq \frac{4}{\alpha T_0}$ and $h_t = d^{\frac{2+\beta}{2\beta}}T^{-\frac{1}{2\beta}}$ for $t \in [1, T_0]$, implies
\begin{align}
    r_{T_0+1} \leq r_1 + \frac{8\cst_3}{\alpha^2}\left(\frac{d^2}{T}\right)^{\frac{\beta-1}{\beta}}+\frac{32\cst_4}{\alpha^2T_0}\left({\color{black}\frac{d^{4 - \beta}}{T^{2}}}\right)^{\frac{1}{\beta}}d^{2-\frac{2}{\beta}}T^{\frac{1}{\beta}} +  \frac{32\cst_5}{\alpha^{2}T_0}d^{2-\frac{2}{\beta}}T^{\frac{1}{\beta}}\enspace.
\end{align}
Since $T \geq d^{2-\frac{\beta}{2}}$, we have $\left(\frac{d^{4-\beta}}{T^2}\right)^{\frac{1}{\beta}} \leq 1$, and for the term on the right hand side of Eq.~\eqref{sfar1_l1} we can deduce that
\begin{align*}
    \frac{\alpha}{8}T_0r_{T_0+1}\leq 174\kappa\bL^2 \frac{d}{\alpha}r_1+\frac{\cst_3T_0}{\alpha}\left(\frac{d^2}{T}\right)^{\frac{\beta-1}{\beta}}+\frac{4\left(\cst_4+\cst_5\right)}{\alpha}d^{2-\frac{2}{\beta}}T^{\frac{1}{\beta}}.
\end{align*}
Substituting the above bound in Eq.~\eqref{sfar1_l1}, yields
\begin{align}\label{sfar4_l1}
    \sum_{t=T_0+1}^{T}\Exp\left[f(\bx_t)-f^{\star}\right]\leq 174\kappa\bL^2\frac{d}{\alpha}r_1 +\frac{\cst_3T_0}{\alpha}\left(\frac{d^2}{T}\right)^{\frac{\beta-1}{\beta}}+\frac{\cst_8}{\alpha}d^{2-\frac{2}{\beta}}T^{\frac{1}{\beta}},
\end{align}
where $\cst_8 = 4\left(\cst_4+\cst_5\right)+\cst_7$.  
\paragraph{Case 2: $t \in [1 , T_0]$.} Note that $\frac{4}{\alpha(T_0+1)}\leq \eta_t$, and by summing Eq.~\eqref{generalscuns_l1} from $1$ to $T_0$ we get
\begin{align}
    \sum_{t=1}^{T_0} \Exp[f(\bx_t) -f^{\star}] 
    &\leq \frac{\alpha (T_0+1)}{8}r_1 + \frac{\cst_3T_0}{\alpha}\left(\frac{d^2}{T}\right)^{\frac{\beta-1}{\beta}} +\sum_{t=1}^{T_0} \frac{4}{T_0\alpha}\left(\cst_4\left({\color{black}\frac{d^{4 - \beta}}{T^{2}}}\right)^{\frac{1}{\beta}}+\cst_5\right)d^{2-\frac{2}{\beta}}T^{\frac{1}{\beta}}\nonumber
    \\&\leq 348\kappa\bL^2\frac{d}{\alpha}r_1 + \frac{\cst_3T_0}{\alpha}\left(\frac{d^2}{T}\right)^{\frac{\beta-1}{\beta}} + \frac{4\left(\cst_4+\cst_5\right)}{\alpha}d^{2-\frac{2}{\beta}}T^{\frac{1}{\beta}}\enspace,\label{sfar5_l1}
\end{align}
where again the last inequality can be obtained by the fact that $T \geq d^{2-\frac{\beta}{2}}$. By taking expectation from both side of Eq.~\eqref{generalscuns_l1} and substituting the provided bounds in Eq.~\eqref{sfar4_l1} and Eq.~\eqref{sfar4_l1} we get
\begin{align*}
    \Exp\left[f(\bar{\bx}_T) - f^{\star}\right] \leq \cst_1\frac{d}{\alpha T}r_1 + \cst_2\frac{d}{\alpha}\left(\frac{d^2}{T}\right)^{\frac{\beta-1}{\beta}},
\end{align*}
where we introduced $\cst_1 = 522 \kappa\bL^2$, and $\cst_2 = 2\left(\cst_3+ 2\left(\cst_4+\cst_5\right)\right)+\cst_8.$
\paragraph{Handling the case $T \leq T_0$.} At the end, we state the proof for the case $T \leq T_0$. By Eq.~\eqref{generalscuns_l1}, we can write
\begin{align*}
    \sum_{t=1}^{T}\Exp[f(\bx_t) - f^{\star}] 
    &\leq \frac{r_1}{2\eta_1} + \frac{\cst_3T}{\alpha}\left(\frac{d^2}{T}\right)^{\frac{\beta-1}{\beta}} + \eta_1T\left(\cst_4+\cst_5\right)d^{2-\frac{2}{\beta}}T^{\frac{1}{\beta}}
    \\&\leq \frac{T_0}{4}r_1 + \frac{\cst_3T}{\alpha}\left(\frac{d^2}{T}\right)^{\frac{\beta-1}{\beta}}+\frac{4T\left(\cst_4+\cst_5\right)}{T_0\alpha}d^{2-\frac{2}{\beta}}T^{\frac{1}{\beta}}.
\end{align*}
Therefore, by convexity of $f$ we can see
\begin{align*}
    \Exp[f(\bar{\bx}_T) - f^{\star}] \leq  \cst_1\frac{d}{\alpha T}r_1 + \frac{\cst_2}{\alpha}\left(\frac{d^2}{T}\right)^{\frac{\beta-1}{\beta}}.
\end{align*}
where $\cst_1 = 348\kappa\bL^2$, and $\cst_2= \cst_3 + 4\left(\cst_4+\cst_5\right).$
\end{proof}



\subsection{Constrained optimization}


\begin{proof}[Proof of Lemma~\ref{scunt}]
% Let $\bx^*_T$ be any minimizer of $\sum_{t = 1}^T f(\bx)$ over $\com$.
Recalling that $\sup_{\bx \in \com}\norm{\nabla f(\bx)} \leq G$, by Lemma~\ref{scuntunc} we have for any $t = 1, \ldots, T$
\begin{align}
    \label{eq:lemma43_0}
    0 \leq \Exp[f(\bx_t)- f^{\star}]\leq \frac{r_t-r_{t+1}}{2\eta_t}-\frac{\alpha}{4}r_t+\frac{b_{t}^2}{\alpha}+\frac{\eta_t}{2}\big(v_t+mG^2\big)\enspace.
\end{align}
Summing up the above inequalities over $t = 1, \ldots, T$, we get
\begin{align}\label{eq:lemgeneta}
    \sum_{t=1}^{T}(f_t(\bx_t)- f^{\star})
    % &\leq
    % \sum_{t=1}^{T}f_t(\bx_t)- \sum_{t=1}^{T} \min_{\bx \in \com}f_t(\bx)\\
    &\leq
    \frac{1}{2}\sum_{t=1}^{T}\Big(\frac{r_t - r_{t+1}}{\eta_t} - \frac{\alpha}{2}r_t\Big) + \sum_{t=1}^{T}\Big(\frac{\eta_t}{2}(v_t+mG^2) +\frac{b_t^2}{\alpha}\Big)\enspace.
\end{align}
\paragraph{Bounding the first term on r.h.s. of Eq.~\eqref{eq:lemgeneta}.}
Recall that $\eta_t = \tfrac{2}{\alpha t}$, hence
\begin{align*}
\sum_{t=1}^{T}\Big(\frac{r_t - r_{t+1}}{\eta_t} - \frac{\alpha}{2}r_t\Big)
=
\frac{\alpha}{2}\sum_{t=1}^{T}\Big(r_t(t - 1) - r_{t+1}t\Big) \leq 0 \enspace.
\end{align*}
% The first term in the right hand side of Eq.~\eqref{eq:lemgeneta} is less than zero. In fact,
% \begin{align*}
%     \sum_{t=1}^{T}\Big(\frac{r_t - r_{t+1}}{\eta_t} - \frac{\alpha}{2}r_t\Big)\leq r_1\left(\frac{1}{\eta_1}-\frac{\alpha}{2}\right)+\sum_{t=2}^{T}r_t\left(\frac{1}{\eta_t}-\frac{1}{\eta_{t-1}}-\frac{\alpha}{2}\right) \leq 0.
% \end{align*}
\paragraph{Bounding the second term on r.h.s. of Eq.~\eqref{eq:lemgeneta}.}
Substitution of $\eta_t = \frac{2}{\alpha t}$ in Eq.~\eqref{eq:lemgeneta}, implies
\begin{align*}
    \sum_{t=1}^{T}\Exp[f(\bx_t)-f^\star]\leq \frac{1}{\alpha}\sum_{t=1}^{T}\Big(\frac{1}{t}(v_t+mG^2)+b_t^2\Big)\enspace.
\end{align*}
The proof is concluded using the standard bound on the partial sum of the harmonic series and the convexity of $f$.
\end{proof}


% \subsection{Unconstrained case}


}
{\color{black}\begin{proof}[Proof of Theorem~\ref{thm:sconvex_l2_cons} ($\ell_2$-randomization)] 
By Lemma \ref{scunt}, we have
\begin{align*}
    \Exp[f(\bar\bx_t)-f(\bx)] \leq \frac{mG^2 \left(\log(T)+1\right)}{\alpha T}+ \frac{1}{\alpha T}\sum_{t =1}^{T}\Big(\frac{v_t}{t}+b_t^2\Big)\enspace.
\end{align*}
Applying Lemma \ref{lem:bias_sphere} (bound on the bias) and Lemma \ref{lem:var_sphere_v2} (bound on the variance), implies
\begin{align*}
    \Exp[f(\bar\bx_t)-f(\bx)] \leq 8\kappa G^2\left(\log(T)+1\right)\frac{d}{\alpha T}+\frac{1}{\alpha T}\sum_{t =1}^{T}\Big(\cst_4h_t^{2(\beta-1)}+\frac{1}{t}d\left(\cst_5h_{t}^2+\cst_6dh_t^{-2}\right)\Big)\enspace,
\end{align*}
where $\cst_4 = (\kappa L)^2$, $\cst_5 = 4\kappa\bL^2$, and $\cst_6 = \frac{\sigma^2\kappa}{2}$. By substituting $h_t = \left(\frac{d^2}{t}\right)^{\frac{1}{2\beta}},$ we can write
\begin{align}\label{eq:const1}
    \Exp[f(\bar\bx_t)-f(\bx)] &\leq 4\kappa G^2\left(\log(T)+1\right)\frac{d}{\alpha T} + \frac{1}{\alpha T}\sum_{t=1}^{T}\left(\left(\cst_4+\cst_6\right)\left(\frac{d^2}{t}\right)^{\frac{\beta-1}{\beta}}+\cst_5d^{1+\frac{2}{\beta}}t^{-\frac{\beta+1}{\beta}}\right)\enspace,
\end{align}
Moreover, we have 
\begin{align*}
    \sum_{t=1}^{T}t^{-\frac{\beta-1}{\beta}}
    % \leq 1+\sum_{t=2}^{T}\int_{t-1}^{t}u^{-\frac{\beta-1}{\beta}}\d u
    =1+\int_{1}^{T}u^{-\frac{\beta-1}{\beta}}\d u
    % = 1+\beta u^{\frac{1}{\beta}}\Big|_{1}^{T}
    = \beta T^{\frac{1}{\beta}}+1 -\beta  \leq \beta T^{\frac{1}{\beta}}\enspace,
\end{align*}
and 
\begin{align*}
    \sum_{t=1}^{T}t^{-\frac{1}{\beta}-1}\leq
    % 1+\sum_{t=2}^{T}\int_{t-1}^{t}u^{-\frac{1}{\beta}-1}\d u
    1+\int_{1}^{T}u^{-\frac{1}{\beta}-1}\d u=1-\beta u^{-\frac{1}{\beta}}\Big|_{1}^{T}
    =
    1+\beta - \beta T^{-\frac{1}{\beta}}\leq 1+\beta\enspace.
    \end{align*}
Therefore, Eq.~\eqref{eq:const1} can be simplified as 
\begin{align*}
    \Exp[f(\bar\bx_t)-f(\bx)] \leq\cst_1\left(\log(T)+1\right)\frac{d}{\alpha T  }+\frac{\cst_2}{\alpha T}d^{\frac{2(\beta-1)}{\beta}}T^{\frac{1}{\beta}}+\frac{\cst_3}{\alpha T}d^{1+\frac{2}{\beta}}\enspace,
\end{align*}
where $\cst_1 = 4\kappa G^2$, $\cst_2 = \beta\left(\cst_3+\cst_5\right)$, and $\cst_3 = (\beta+1)\cst_5$. Furthermore, by the fact that $f$ is a convex function, we get 
\begin{align*}
    \Exp[f(\bar{\bx}_T)-f(\bx)] &\leq \cst_1\frac{d\left(\log(T)+1\right)}{\alpha T} +\frac{\cst_2}{\alpha}\left(\frac{d^2}{T}\right)^{\frac{\beta-1}{\beta}}+\frac{\cst_3}{\alpha}\frac{d^{1+\frac{2}{\beta}}}{T}\enspace.
\end{align*}
\end{proof}
\begin{proof}[Proof of Theorem~\ref{thm:sconvex_l1_cons} ($\ell_1$-randomization)] Applying Lemma \ref{scunt}, yields
\begin{align*}
   \Exp[f(\bar\bx_t)-f^\star] \leq \frac{mG^2\left(\log(T)+1\right)}{\alpha T}+ \frac{1}{\alpha T}\sum_{t = 1}^{T}\Big(\frac{v_t}{t}+b_t^2\Big)\enspace.
\end{align*}
By utilizing Lemma \ref{lem:bias_simplex} (bound on the bias) and Lemma \ref{lem:var_l1_v2} (bound on the variance), we get 
\begin{align*}
    \Exp[f(\bar\bx_t)-f^\star] \leq 87\kappa G^2\left(\log(T)+1\right)\frac{d}{\alpha T}+\frac{1}{\alpha T}\sum_{t = 1}^{T}\Big(\cst_4h_{t}^{2(\beta-1)}d^{1-\beta}+\frac{1}{t}\left(\cst_5h_t^2+\cst_6d^3h_t^{-2}\right)\Big)\enspace,
\end{align*}
where $\cst_4 = \left(\kappa_\beta \ell L\right)^2$, $\cst_5 = 856\kappa\bL^2$, and $\cst_6 = \frac{\sigma^2\kappa}{2}$. Plugging in $h_t = d^{\frac{2+\beta}{2\beta}}t^{-\frac{1}{2\beta}}$, implies
\begin{align*}
    \Exp[f(\bar\bx_t)-f^\star] \leq 87\kappa G^2\left(\log(T)+1\right)\frac{d}{\alpha T}+\frac{1}{\alpha T}\sum_{t=1}^{T}\left(\left(\cst_4+\cst_6\right)\left(\frac{d^2}{t}\right)^{\frac{\beta-1}{\beta}}+\cst_5d^{1+\frac{2}{\beta}}t^{-\frac{\beta+1}{\beta}}\right)
    \enspace.
\end{align*}
We a similar argument as in the previous Theorem, we have
\begin{align*}
    \Exp[f(\bar\bx_t)-f(\bx)] \leq \cst_1\left(\log(T)+1\right)\frac{d}{\alpha T}+\frac{\cst_2}{\alpha T}d^{\frac{2(\beta-1)}{\beta}}T^{\frac{1}{\beta}}+ \frac{\cst_3}{\alpha T}d^{1+\frac{2}{\beta}}
    \enspace.
\end{align*}
where we assigned $\cst_1 = 87\kappa G^2$, $\cst_2 =\beta\left(\cst_4+\cst_6\right)$, and $\cst_3=\left(\beta+1\right)\cst_5$.
% Using convexity of $f$, finishes the proof.
\end{proof}
}



\newpage
\section{Upper bound for quadratic functions}
% \evg[inline]{Todo: harmonize with $\circ$, $\diamond$; write general statement for unbiased gradient estimators.}

\begin{lemma}
\label{lem:general_quadratics}
Assume that $f \in \mathcal{F}_{\quadr}$. Consider the iterative algorithm defined in Eq.~\eqref{eq:algo_general} with $\com = \bbR^d$.
Assume that
\begin{align*}
    \Exp[\bg_t \mid \bx_t] = \nabla f(\bx_t)\enspace,
\end{align*}
then for all $t \geq 1$ we have
\begin{align}\label{ri1}
    \Exp[f(\bx_{t+1})\mid \bx_t] = f(\bx_{t}) - \eta_t\norm{\nabla f(\bx_t)}^2 + \frac{\eta_t^2}{2} \bg^\top_t A \bg_t\enspace.
\end{align}
\end{lemma}
\begin{proof}
Recall that
\begin{align*}
    f(\bx) = \frac{1}{2} \bx^\top A \bx + \bb^\top \bx + c\enspace.
\end{align*}
Hence, for any $\bx, \bu \in \bbR^d$ we have Taylor's theorem which states that
\begin{align*}
    &f(\bx - \bu) = f(\bx) - \scalar{\nabla f(\bx)}{\bu} + \frac{1}{2} \bu^\top A\bu\enspace.
\end{align*}
% The above combined with the fact that $\Exp[\bzeta_t \bzeta_t^\top] = \tfrac{1}{d}I$ and $\int_{-1}^1 r K(r) \d r = \int_{-1}^1 |r| \d r = 1$ implies
% \begin{align*}
%     \Exp[\bg_t]
%     &=
%     \frac{d}{2h_t}\Exp\Big[\left(f(\bx_t + h_tr_t \bzeta_t) - f(\bx_t - h_tr_t \bzeta_t) + \xi_t - \xi_t'\right)\bzeta_tK(r_t) \mid \bx_t\Big] = \nabla f(\bx_t)\enspace.
% \end{align*}
Furthermore, since $\bx_{t+1} = \bx_t - \eta_t \bg_t$ and $\bg_t$ is an unbiased estimator of $\nabla f(\bx_t)$ we conclude that
\begin{align*}
% \label{ri1}
    \Exp[f(\bx_{t+1})\mid \bx_t] = f(\bx_{t}) - \eta_t\norm{\nabla f(\bx_t)}^2 + \frac{\eta_t^2}{2} \bg^\top_t A \bg_t\enspace.
\end{align*}
\end{proof}


\subsection{$\ell_2$-randomization}
The next result is a particular case of \cite[Theorem 3.3][]{fang2018symmetric}, where the expressions for moments of vector uniformly distributed on the unit sphere are provided.
\begin{lemma}\label{lemmoment}
Let $\bzeta = (\zeta_1, \ldots, \zeta_d)^\top \in \bbR^d$ be distributed uniformly on $\sphere_{d}^2$, then
\begin{itemize}
    \item $\Exp[\zeta^{2k+1}_j \zeta^{k'}_{j'}] = 0$ for all $j \neq j'$, $k', k \in \bbN$.
    \item $\Exp[\zeta_j^2\zeta_{j'}^2] = \tfrac{1}{d(d+2)}$ for all $j \neq j'$;
    \item $\Exp[\zeta_j^4] = \tfrac{3}{d(d+2)}$ for all $j \in \bbN$.
\end{itemize}
\end{lemma}
% \begin{proof}
% Let us show the first claim. Fix some $j \neq j'$ and $k, k' \in \bbN$.
% Due to the spherical symmetry, the distribution of $\bzeta$ is the same as that of
% \begin{align*}
%     \bzeta^{-j} = (\zeta_1, \ldots, \zeta_{j - 1}, -\zeta_j, \zeta_{j + 1}, \ldots, \zeta_d)^\top\enspace.
% \end{align*}
% % Thus, for any measurable $F : \mathbb{S}_{d - 1} \to \bbR$ we have
% % \begin{align*}
% %     \Exp[F(\bzeta)] = \Exp[F(\bzeta^{-j})]\enspace.
% % \end{align*}
% In particular, it holds that
% \begin{align*}
%     \Exp[\zeta^{2k+1}_j \zeta^{k'}_{j'}] = \Exp[(-\zeta_j)^{2k+1} \zeta^{k'}_{j'}] = -\Exp[\zeta^{2k+1}_j \zeta^{k'}_{j'}]\enspace,
% \end{align*}
% which yields the first claim. 
% For the second and the third claim, without loss of generality (again due to the spherical symmetry) assume that $j = 1, j' = 2$.
% We have
% \begin{align}
%     \Exp[\zeta_1^2\zeta_{2}^2]
%     =
%     \frac{1}{2\binom{d}{2}} \sum_{j \neq j'}\Exp[\zeta_j^2\zeta_{j'}^2]
%     &=
%     \frac{1}{2\binom{d}{2}} \Exp\parent{\norm{\zeta}^2\norm{\zeta}^2 - \sum_{j = 1}^d \zeta_j^4}\nonumber\\
%     &=
%     \frac{1}{d(d-1)} \parent{1 - d \Exp[\zeta_1^4]}\enspace.\label{eq:4_sphere}
% \end{align}

% % {
% % \color{black} I computed and it seems that
% % \begin{align*}
% %     \Exp[\zeta_1^4] = \frac{3}{d(d+2)}\enspace.
% % \end{align*}
% % Thus,
% % \begin{align*}
% %     \Exp[\zeta_1^2\zeta_{2}^2] = \frac{1}{d(d-1)} \parent{1 - \frac{3}{d + 2}} = \frac{1}{d(d+2)}\enspace.
% % \end{align*}
% % Yes, I've exactly got the same thing. I'm writing the proof here.
% % }

% Let $\bZ = (Z_1, \ldots, Z_d) \sim \mathcal{N}(0, I)$ and recall that $\left(\tfrac{Z_1}{\norm{\bZ}}, \ldots , \tfrac{Z_d}{\norm{\bZ}}\right)$ and $\bzeta$ have the same distribution. 
% Furthermore, it is known \cite[see \eg Theorem 2.3][]{fang2018symmetric} that
%  $\left(\tfrac{Z_1}{\norm{\bZ}}, \dots , \tfrac{Z_d}{\norm{\bZ}}\right)$ and $\norm{\bZ}$ are independent. Thus, we get
% \begin{align*}
%     \Exp[\zeta_1^4]
%     =
%     \Exp\left[\frac{Z_1^4}{\norm{\bZ}^4}\right]
%     &=
%     \Exp\left[\frac{Z_1^4}{\norm{\bZ}^4}\right] \frac{\Exp[\norm{\bZ}^4]}{\Exp[\norm{\bZ}^4]}
%     =
%     \Exp\left[\frac{Z_1^4}{\norm{\bZ}^4}\norm{\bZ}^4\right] \frac{1}{\Exp[\norm{\bZ}^4]}\\
%     &=
%     \Exp[Z_{1}^4]\frac{1}{\Exp[\norm{\bZ}^4]}
%     = 
%     \frac{3}{d(d+2)}\enspace,
% \end{align*}
% where the last equality follows from the expression for the fourth moment of standard Gaussian and second moment of the Chi-squared distribution with $d$ degrees of freedom. Substituting the above into Eq.~\eqref{eq:4_sphere} asserts the second and the third claim.

% % Note that $\norm{\bZ}^2$ follows Chi-squared distribution with $d$ degrees of freedoms Therefore,
% % \begin{align*}
% %     \Exp[\zeta_1^2\zeta_{2}^2]
% %     =\frac{1}{\Exp[\norm{\bold{z}}^4]} = \frac{1}{d(d+2)},
% % \end{align*}
% % and $\Exp[\zeta_1^4] = \frac{3}{d(d+2)}$
% \end{proof}


\begin{proof}[Proof of Theorem~\ref{thm:upper_quadratic} ($\ell_2$-randomization)]
First we show that $\bg_t^{\circ}$ is an unbiased estimator of $\nabla f(\bx_t)$, then applying Lemma~\ref{lem:general_quadratics}, we will bound the variance term which appears in Eq.~\eqref{ri1}.
For any $\bx, \bu \in \bbR^d$ we have Taylor's theorem which states that
\begin{align*}
    &f(\bx + \bu) = f(\bx) + \scalar{\nabla f(\bx)}{\bu} + \frac{1}{2} \bu^\top \bfA \bu\enspace,\\
    &f(\bx - \bu) = f(\bx) - \scalar{\nabla f(\bx)}{\bu} + \frac{1}{2} \bu^\top \bfA\bu\enspace.
\end{align*}
The above combined with the fact that $\Exp[\bzeta_t^{\circ} (\bzeta_t^{\circ})^\top] = \tfrac{1}{d}\bfI$ and $\int_{-1}^1 r K(r) \d r = \int_{-1}^1 |r| \d r = 1$ implies
\begin{align*}
    \Exp_t[\bg_t^{\circ}]
    &=
    \frac{d}{2h_t}\Exp_t\Big[\left(f(\bx_t + h_tr_t \bzeta_t^{\circ}) - f(\bx_t - h_tr_t \bzeta_t^{\circ}) + \xi_t - \xi'_t\right)\bzeta_t^{\circ}K(r_t)\Big] = \nabla f(\bx_t)\enspace.
\end{align*}
Thus, we can apply the result of Lemma~\ref{lem:general_quadratics}.
% Furthermore, since $\bx_{t+1} = \bx_t - \eta_t \bg_t$ we have
% \begin{align}\label{ri1}
%     \Exp[f(\bx_{t+1})\mid x_t] = f(x_{t}) - \eta_t\norm{\nabla f(\bx_t)}^2 + \frac{\eta_t^2}{2} \bg^\top_t A \bg_t\enspace.
% \end{align}
Now our goal is to bound the variance term $\bg^\top_t \bfA \bg_t$. Observe that by definition of $\bg_t$ we have
{
% \color{black}
\begin{align*}
    \scalar{\bg^{\circ}_t}{\bfA \bg_t^{\circ}}
    &=
    \frac{d^2}{4h_t^2}\left(f(\bx_t + h_tr_t \bzeta_t^{\circ}) - f(\bx_t + h_tr_t \bzeta_t^{\circ}) + \xi_t - \xi_t'\right)^2K^2(r_t) \scalar{\bzeta_t^{\circ}}{\bfA \bzeta_t^{\circ}}\\
    &=
    \frac{d^2}{4h_t^2}\left(h_tr_t\scalar{\nabla f(\bx_t)}{\bzeta_t^{\circ}} + \xi_t - \xi_t'\right)^2K^2(r_t) \scalar{\bzeta_t^{\circ}}{\bfA \bzeta_t^{\circ}}\\
    &\leq
    \frac{d^2}{2h_t^2}\left(h_t^2r^2_t\scalar{\nabla f(\bx_t)}{\bzeta_t^{\circ}}^2 + (\xi_t - \xi_t')^2\right)K^2(r_t) \scalar{\bzeta_t^{\circ}}{\bfA \bzeta_t^{\circ}}\enspace.
\end{align*}
Taking expectation and using the independence Assumption~\ref{ass1}, the above implies that
\begin{equation}
\label{eq:quadratic_2}
\begin{aligned}
    \Exp_t[\scalar{\bg^{\circ}_t}{\bfA \bg_t^{\circ}}]
    \leq
    \frac{d^2}{2}&\underbrace{{\Exp[ r^2 K^2(r)]}}_{\triangleq \kappa_1 = 2 / 3}\Exp_t\left[\scalar{\nabla f(\bx_t)}{\bzeta_t}^2\scalar{\bzeta_t^{\circ}}{\bfA\bzeta_t^{\circ}}\right]
    +
    \frac{d\sigma^2}{h_t^2}\underbrace{{\Exp[K^2(r)]}}_{\triangleq \kappa_2 = 2} \tr(\bfA)\enspace.
%     \\
%     &\leq \frac{d^2}{2}
%     \underbrace{\parent{\int_{-1}^1 r^2 K^2(r) \d r}}_{\triangleq \kappa_1}\Big(\Exp_t[\langle \nabla f(\bx_t),\bzeta \rangle^4]\Big)^{\frac{1}{2}}\Big(\Exp_t[(\bzeta_t^\top A \bzeta_t)^2]\Big)^{\frac{1}{2}}+ \frac{d\sigma^2}{h_t^2}\underbrace{\parent{\int_{-1}^1 K^2(r) \d r}}_{\triangleq \kappa_2} \tr(A)\enspace\\&\leq
%     \frac{d\kappa_{1}\tr(A)}{2}\Big(\sum_{1\leq i,j \leq d}\Exp_t[\bzeta_{i}^{2}\bzeta_{j}^{2}]\big(\nabla f(\bx_t)\big)_i^2\big(\nabla f(\bx_t)\big)_j^2\Big)^\frac{1}{2}+ \frac{d\sigma^2}{h_t^2} \kappa_2 \tr(A)\enspace\\&\leq
%     \kappa_{1}\tr(A)\norm{\nabla f(\bx_t)}^2+ \frac{d\sigma^2}{h_t^2} \kappa_2 \tr(A)\enspace,
\end{aligned}
\end{equation}
Applying Cauchy-Schwarz inequality and Lemma~\ref{lemmoment} we deduce that
% \evg[inline]{Need to come back here, there seem to be a mistake (a constant $\sqrt{3}$ is missing)}
% \evg[inline]{Fixed the issue, to doublecheck}
\begin{align*}
    \Exp_t\bigg[\scalar{\nabla f(\bx_t)}{\bzeta_t^{\circ}}^2&\scalar{\bzeta_t^{\circ}}{\bfA\bzeta_t^{\circ}}\bigg]
    \leq
    \left(\Exp_t[\langle \nabla f(\bx_t),\bzeta_t^{\circ} \rangle^4]\right)^{\frac{1}{2}}\left(\Exp_t[\scalar{\bzeta_t^{\circ}}{\bfA\bzeta_t^{\circ}}^2]\right)^{\frac{1}{2}}\\
    &\leq
    \left(\frac{3}{d(d+2)}\sum_{1\leq i,j \leq d}\big(\nabla f(\bx_t)\big)_i^2\big(\nabla f(\bx_t)\big)_j^2\right)^\frac{1}{2}\parent{\frac{3}{d(d+2)}\sum_{j = 1}^d A_{jj}^2}^{\frac{1}{2}}\\
    &=\frac{3}{d(d+2)}\|\nabla f(\bx_t)\|^2\parent{\sum_{j = 1}^d A_{jj}^2}^{\frac{1}{2}}
    \leq
    \frac{3}{d(d+2)} \tr(A)\|\nabla f(\bx_t)\|^2\enspace.
\end{align*}
Substituting the above bound into Eq.~\eqref{eq:quadratic_2} we obtain
\begin{align*}
    \Exp_t[\scalar{\bg^{\circ}_t}{A \bg_t^{\circ}}]
    % &\leq
    % \frac{3d^2}{2d(d+2)}\kappa_1\tr(\bfA)\|\nabla f(\bx_t)\|^2  + \frac{d\sigma^2}{h_t^2}\kappa_2 \tr(A)
    \leq
    {\tr(\bfA)}\|\nabla f(\bx_t)\|^2  + \frac{2d\sigma^2}{h_t^2} \tr(\bfA)\enspace.
\end{align*}
% where in the last inequality we used the fact that $\tfrac{3d^2}{2d(d+2)} \leq 3/2$ for all $d \geq 1$.
% \evg[inline]{need to come back here to fix}
}
% Hi! I am here!

% So in the above, I bound 
% \begin{align*}
%     \Exp\left[\scalar{\nabla f(\bx_t)}{\bzeta_t}^2\bzeta_t^\top A \bzeta\right] \leq \frac{\upsilon}{d}\|\nabla f(\bx_t)\|^2
% \end{align*}
% like that

% But it is actually very rough

% I would expect that
% \begin{align*}
%     \Exp\left[\scalar{\nabla f(\bx_t)}{\bzeta_t}^2\bzeta_t^\top A \bzeta\right] \leq \frac{\tr(A)}{d^2}\|\nabla f(\bx_t)\|^2
% \end{align*}
% which would be nice for us! you see the point? (p.s. the above inequality might involve some constant, so it is not exact :) )



Substituting the above bound on the variance term into Eq.~\eqref{ri1} and taking total expectation from both sides, we get
\begin{align*}
    \Exp[f(\bx_{t+1})] = \Exp[f(\bx_{t})] - \eta_t\parent{1 - \eta_t\frac{ \tr(\bfA)}{2}}\Exp\big[\norm{\nabla f(\bx_t)}^2 \big]
    +{d \tr(\bfA)\sigma^2 }\parent{\frac{\eta_t}{h_t}}^2\enspace.
\end{align*}
% As long as $4 \geq \eta_t{ d\upsilon\kappa_1}$ 
Set $\eta_t = \min \parent{\tfrac{1}{\tr(\bfA)}, \tfrac{2}{\lambda_{\min}^{\nz}(\bfA) t}}$, hence for such a choice of the step-size we have $1 - \eta_t\frac{ \tr(\bfA)}{2} \geq \tfrac{1}{2}$ and
we can use the fact that $f$ is $\lambda_{\min}^{\nz}(\bfA)$-gradient dominant, leading to
\begin{align}
    \label{eq:quad_l2_0}
    \delta_{t + 1} \leq \left(1 - \lambda_{\min}^{\nz}(\bfA)\eta_t \right)\delta_{t}
    +{d \tr(\bfA)\sigma^2 }\parent{\frac{\eta_t}{h_t}}^2\enspace,
\end{align}
where $\delta_t \triangleq \Exp[f(\bx_t) - f^\star]$.

% \evg{To finish from here, I need to go... Everything below is from the old version}

% where $\delta(t) = \Exp[f(x_{t}) - f(x^*)]$, for $t =1 \dots T-1$. 
Let $T_{0} \triangleq \floor{\frac{2\tr(\bfA)}{\lambda_{\min}^{\nz}(\bfA)}}$---the moment when $\eta_t$ changes its behaviour.

\paragraph{Case 1: $t \in [T_0 + 1, T]$.} For any $t \in [T_{0}+1, T]$ we have ${\color{black}}\eta_{t} = \frac{2}{\lambda_{\min}^{\nz}(\bfA) t}$ and 
% \arya{I think it's better to assign different $h_{t}$s for different blocks}
${h_{t} = \sqrt{\frac{d}{\lambda_{\min}^{\nz}(\bfA)}}}$ and, thus, in this range of $t$ we have
\begin{align}
    \label{eq:quad_l2_1}
    \delta_{t+1} \leq \left(1 - \frac{2}{t} \right)\delta_{t}
    +4\sigma^2\frac{\tr(\bfA)}{ \lambda_{\min}^{\nz}(\bfA) t^2}\enspace.
    % \,\qquad \forall t \in\{T_{1}+1, \dots, T\} \enspace.
\end{align}
Applying Lemma \ref{lemma:bisev} we deduce that 
\begin{align}\label{ricco1}
    \delta_{T} \leq \frac{4\tr(\bfA) }{\lambda_{\min}^{\nz}(\bfA) T}\delta_{T_0+1} +4\sigma^2\frac{\tr(\bfA)}{ \lambda_{\min}^{\nz}(\bfA) T}\enspace.
\end{align}
% \evg{Stopped here}
\paragraph{Case 2: $t \in [1, T_0]$.}
To conclude the proof, it remains to bound $\delta_{T_0 + 1}$. For any $t \in \{1, \dots, T_{0}\}$, using the fact that $\eta_t^2 \leq \big(\frac{1}{\tr(\bfA)}\big)^2$ and the definition of $h_t$ we deduce from Eq.~\eqref{eq:quad_l2_0} that
\begin{align*}
    \delta_{t+1} \leq
    \left(1 - \frac{\lambda_{\min}^{\nz}(\bfA)}{\tr(\bfA)} \right)\delta_{t}
    +{d \tr(\bfA)\sigma^2 }\parent{\frac{\eta_t}{h_t}}^2
    \leq
    \delta_{t}
    +\sigma^2\frac{\lambda_{\min}^{\nz}(\bfA) }{ \tr(\bfA) }\enspace,
\end{align*}
Therefore, unfolding the above recursion and using the definiton of $T_0$, we get
\begin{align}
\label{ricco2}
    \delta_{T_0+1}&\leq \delta_1 + \sigma^2\frac{T_0\lambda_{\min}^{\nz}(\bfA) }{ \tr(\bfA) } \leq \delta_1 + 2\sigma^2\enspace.
\end{align}
{\color{black}
Substituting the bound derived in Eq.~\eqref{ricco2} into Eq.~\eqref{ricco1} we obtain

\begin{align*}
    \delta_{T}
    \leq
    \frac{4\tr(\bfA) }{\lambda_{\min}^{\nz}(\bfA) T}(\delta_1 + 2\sigma^2) +4\sigma^2\frac{\tr(\bfA)}{ \lambda_{\min}^{\nz}(\bfA)}
    =
    \frac{4\tr(\bfA) }{\lambda_{\min}^{\nz}(\bfA) T}\parent{\delta_1 + 3\sigma^2}\enspace.
\end{align*}
}
{\color{black}
\paragraph{Handling the case $T \leq T_0$.} In this case, note that $\frac{2}{\lambda_{\min}^{\nz}(\bfA)(T_0+1)}\leq\eta_t$, and $\eta_t^2 \leq \frac{4}{\left(\lambda_{\min}^{\nz}(\bfA)\right)^2T^2}$. By Eq.~\eqref{eq:quad_l2_0}, we get 
\begin{align*}
    \delta_{T+1}&\leq \delta_1\left(1 - \frac{2}{T_0+1}\right)^T +16\sigma^2\frac{\tr\left(\bA\right)}{\lambda_{\min}^{\nz}(\bfA)T}.
\end{align*}
Again, since for any $\rho, T > 0$ we have $(1 - \rho)^{T} \leq \exp(-\rho T) \leq \tfrac{1}{\rho T}$, we observe that for $\rho = \tfrac{2}{T_0 + 1}$ it can be written as
\begin{align*}
    \delta_{T} &\leq \frac{T_0+1}{2(T-1)}\delta_1 +16\sigma^2\frac{\tr\left(\bA\right)}{\lambda_{\min}^{\nz}(\bfA)(T-1)}
    \leq
    \frac{4\tr(\bfA) }{\lambda_{\min}^{\nz}(\bfA) T}\parent{\delta_1 + 8\sigma^2}\enspace.
\end{align*}
The proof is concluded by $T_0+1\leq 2T_0$ and $T-1\geq\frac{T}{2},$ for $2\leq T\leq T_0.$
}
\end{proof}




\begin{proof}[Proof of Theorem~\ref{thm:upper_quadraticl1} ($\ell_1$-randomization)]
We start identically as in the proof of Theorem~\ref{thm:upper_quadratic} and show that
\begin{align*}
    \Exp [\bg^{\diamond}_t] = \frac{d}{2h_t}\Exp\left[(f(\bx_t + h_t r_t \bzeta^{\diamond}_t) - f(\bx_t - h_t r_t \bzeta^{\diamond}_t) + \xi_t - \xi_t')\sign(\bzeta^{\diamond}_t)K(r_t)\right] = \nabla f(\bx_t)\enspace,
\end{align*}
where the equality follows from the fact that $\Exp[\bzeta_t^{\diamond} \sign(\bzeta_t^{\diamond})^\top] = \frac{1}{d}\bfI$ and the properties of the kernel $K(\cdot)$.
Again, we continue similarly and provide a bound on the variance term
\begin{align*}
    \scalar{\bg^{\diamond}_t}{\bfA \bg^{\diamond}_t}
    &=
    \frac{d^2}{4h_t^2}\parent{f(\bx_t + h_t r_t \bzeta^{\diamond}_t) - f(\bx_t - h_t r_t \bzeta^{\diamond}_t) + \xi_t - \xi_t'}^2 K^2(r_t)\scalar{\sign(\bzeta_t^{\diamond})}{\bfA \sign(\bzeta_t^{\diamond})}\\
    &=
    \frac{d^2}{4h_t^2}\parent{h_tr_t\scalar{\nabla f(\bx_t)}{\bzeta_t^{\diamond}} + \xi_t - \xi_t'} K^2(r_t)\scalar{\sign(\bzeta_t^{\diamond})}{\bfA \sign(\bzeta_t^{\diamond})}\\
    &\leq
    \frac{d^2}{2h_t^2}\parent{h_t^2r_t^2\scalar{\nabla f(\bx_t)}{\bzeta_t^{\diamond}}^2 + (\xi_t - \xi_t')^2} K^2(r_t)\scalar{\sign(\bzeta_t^{\diamond})}{\bfA \sign(\bzeta_t^{\diamond})}\enspace.
\end{align*}
Taking the expectation from both sides of the above inequality and utilizing Assumption~\ref{ass1}, we obtain similarly to the previous proof
\begin{align}
    \label{eq:quadratic_l1_0}
    \Exp[ \scalar{\bg^{\diamond}_t}{\bfA \bg^{\diamond}_t}]
    \leq
    \frac{d^2}{3}&\Exp[\scalar{\nabla f(\bx_t)}{\bzeta_t^{\diamond}}^2\scalar{\sign(\bzeta_t^{\diamond})}{\bfA \sign(\bzeta_t^{\diamond})}]
    +
    \frac{2d^2\sigma^2}{h_t^2}\tr(\bfA)\enspace.
\end{align}
% \arya[inline]{Here I need to specify the constants $\kappa_1$ and $\kappa_2$}
It remains to bound the first expectation on the right hand side of the above inequality. By Cauchy-Schwarz inequality, it is sufficient to bound
\begin{align}
    \label{eq:quadratic_l1_1}
    \Exp[\scalar{\nabla f(\bx_t)}{\bzeta_t^{\diamond}}^4]\qquad\text{and}\qquad\Exp[\scalar{\sign(\bzeta_t^{\diamond})}{\bfA \sign(\bzeta_t^{\diamond})}^2]\enspace.
\end{align}
For the second expectation in Eq.~\eqref{eq:quadratic_l1_1} we can write
\begin{align*}
    \Exp[\scalar{\sign(\bzeta_t^{\diamond})}{\bfA \sign(\bzeta_t^{\diamond})}^2] = \Exp\parent{\sum_{i,j = 1}^dA_{ij}\epsilon_i\epsilon_j}^2\enspace,
\end{align*}
where $\epsilon_1, \ldots, \epsilon_d$ are \iid Rademacher random variables. Thus, we have
\begin{align}
    \label{eq:quadratic_l1_2}
    \Exp[\scalar{\sign(\bzeta_t^{\diamond})}{\bfA \sign(\bzeta_t^{\diamond})}^2] = \sum_{i = 1}^d A_{ii}^2 \leq \tr(\bfA)^2\enspace.
\end{align}
Meanwhile, for the first expectation in Eq.~\eqref{eq:quadratic_l1_1} we have
\begin{align*}
    \Exp[\scalar{\nabla f(\bx_t)}{\bzeta_t^{\diamond}}^4] = \Exp[\scalar{\nabla f(\bx_t)}{\bepsilon \odot \bZ}^4]\enspace,
\end{align*}
where $\bepsilon \in \bbR^d$ is an \iid Rademacher vector and $\bZ$ is distributed uniformly on $\Delta_{d-1}$ being independent from $\bepsilon$. We again recall the following property of $\bZ = (Z_1, \ldots, Z_d)^\top$:
\begin{align*}
    \Exp[Z_j^4] = \frac{24(d-1)!}{(d+3)!}\qquad\text{and}\qquad \Exp[Z_j^2Z_i^2] = \frac{4(d-1)!}{(d+3)!}\qquad i\neq j\enspace.
\end{align*}
Hence, due to the above and since $\bepsilon$ is an \iid Rademacher vector we have
\begin{align}
    \label{eq:quadratic_l1_3}
    \Exp[\scalar{\nabla f(\bx_t)}{\bepsilon \odot \bZ}^4] = \sum_{i, j = 1}^d \parent{\nabla f(\bx_t)}_i^2\parent{\nabla f(\bx_t)}_j^2 \Exp[Z_i^2 Z_j^2] \leq \frac{25}{d^4} \norm{\nabla f(\bx_t)}^4\enspace.
\end{align}
Substituting Eqs.~\eqref{eq:quadratic_l1_2}--\eqref{eq:quadratic_l1_3} into Eq.~\eqref{eq:quadratic_l1_0} we deduce that
\begin{align*}
    \Exp[ \scalar{\bg^{\diamond}_t}{\bfA \bg^{\diamond}_t}] \leq 2{\tr(\bfA)}\norm{\nabla f(\bx_t)}^2 + \frac{2d^2\sigma^2\tr(\bfA)}{h_t^2}\enspace.
\end{align*}
% \evg[inline]{to finish}
{\color{black}Combining the last display with Lemma \ref{lem:general_quadratics}, implies
\begin{align*}
    \delta_{t+1} \leq \delta_t - \eta_t\left(1- \eta_t \tr(\bfA)\right)\norm{\nabla f(\bx_t)}^2+ 2d^2\sigma^2\tr(\bfA)\left(\frac{\eta_t}{h_t}\right)^2,
\end{align*}
where $\delta_t = \Exp [f(\bx_t)]-f^{\star}$, for all $t \geq 1$.
{\color{black}Similar to the proof of Theorem \ref{thm:upper_quadratic}, first we assume that $T_0< T$, where $T_0 = \floor{\frac{4\tr(\bA)}{\lambda_{\min}^{\nz}(\bfA)}}$.} Since $\eta_t \leq \frac{1}{2\tr(\bfA)}$, we have and $1 - \eta_t\tr(\bfA) \geq \frac{1}{2}$. Hence, since $f$ is $\lambda_{\min}^{\nz}(\bfA)$-gradient dominant we deduce \begin{align}\label{genl1quad1}
    \delta_{t+1} \leq \left(1 - \lambda_{\min}^{\nz}(\bfA) \eta_t \right)\delta_t  + 2d^2\sigma^2\tr(\bfA)\left(\frac{\eta_t}{h_t}\right)^2\enspace.
\end{align}
Note how the above inequality is similar to Eq.~\eqref{eq:quad_l2_0} appearing in the previous proof. The only difference is that $d$ in Eq.~\eqref{eq:quad_l2_0} is replaced by $2d^2$ in the above case. The term $2d^2$ is taken care by the step-size $h_t = d\sqrt{\tfrac{2}{\lambda_{\min}^{\nz}(\bfA)}}$.
Performing analogous arguments, we deduce that
\begin{align*}
    \delta_{T}
    \leq
    \frac{8\tr(\bfA) }{\lambda_{\min}^{\nz}(\bfA) T}(\delta_1 + 4\sigma^2) +4\sigma^2\frac{\tr(\bfA)}{ \lambda_{\min}^{\nz}(\bfA) T}
    =
    \frac{4\tr(\bfA) }{\lambda_{\min}^{\nz}(\bfA) T}\parent{2\delta_1 + 9\sigma^2}\enspace.
\end{align*}
{\color{black}
\paragraph{Handling the case $T \leq T_0$.} Again note that $\frac{2}{\lambda_{\min}^{\nz}(\bfA)\left(T_0+1 \right)}\leq\eta_{t}$, and $\eta_t^2\leq\frac{4}{\left(\lambda_{\min}^{\nz}(\bfA)\right)^2T^2}$. Then by Eq.~\eqref{genl1quad1} we can write
\begin{align*}
    \delta_{T+1}&\leq \delta_1\left(1 - \frac{2}{T_0+1}\right)^T +16\sigma^2\frac{\tr\left(\bA\right)}{\lambda_{\min}^{\nz}(\bfA)T},
\end{align*}
and 
\begin{align*}
    \delta_{T} &\leq \frac{T_0+1}{2(T-1)}\delta_1 +16\sigma^2\frac{\tr\left(\bA\right)}{\lambda_{\min}^{\nz}(\bfA)(T-1)}
    \leq
    \frac{8\tr(\bfA) }{\lambda_{\min}^{\nz}(\bfA) T}\parent{\delta_1 + 4\sigma^2}\enspace,
\end{align*}
where the last inequality is obtained by $T_0+1\leq 2T_0$ and $T-1\geq\frac{T}{2},$ for $2\leq T\leq T_0.$
}
% where we use the fact that $f$ is a $\gamma$-gradient dominant function. Recall that $T_1 =\floor{ \frac{2\sqrt{24}\tr(A)\kappa_1}{3\gamma}}$. First we assume that $T_1 \leq T$. Then for any $t = T_1+1,\dots,T$ we have $\eta_t = \frac{2}{\gamma}$, $h_t =\frac{d}{\sqrt{\gamma}}$, and we get
% \begin{align*}
%     \delta_{t+1} \leq \left(1-\frac{2}{t}\right)\delta_t + \frac{4\sigma^2\tr(A)\kappa_2}{\gamma t^2}.
% \end{align*}
% By applying Lemma \ref{lemma:bisev}, we have
% \begin{align}\label{genl1quad2}
%     \delta_T \leq \frac{4\sqrt{24}\tr(A)\kappa_1}{3\gamma T}\delta_{T_1+1} + \frac{4\sigma^2\tr(A)\kappa_2}{\gamma T}.
% \end{align}
% If $T_1 = 1$, the proof can be concluded. Otherwise, it is enough to provide an upper bound for $\delta_{T_1+1}.$ By substituting $\eta_t = \frac{3}{\sqrt{24}\tr(A)\kappa_1}$, $h_t = \frac{d}{\sqrt{\gamma}}$, for $t = 1,\dots,T_1$ in \eqref{genl1quad1}, we get
% \begin{align*}
%     \delta_{t+1} \leq (1-\frac{1}{T_1+1})\delta_{t} + \frac{3\gamma \sigma^2 \kappa_2}{8\tr(A)\kappa_1}.
% \end{align*}
% Therefore, 
% \begin{align*}
%     \delta_{T_1+1} \leq \delta_1 +\frac{3\gamma \sigma^2 \kappa_2}{8\tr(A)\kappa_1}T_1\leq \delta_1 + \frac{\sqrt{24}\sigma^2\kappa_2}{4}.
% \end{align*}
% By replacing the last display in \eqref{genl1quad2}, we deduce that
% \begin{align*}
%     \delta_T \leq \frac{4\sqrt{24}\tr(A)\kappa_1}{3\gamma T}\left(\delta_1+\frac{\sqrt{24}\sigma^2\kappa_2}{4}\right)+\frac{4\sigma^2\tr(A)\kappa_2}{\gamma T} \leq \cst_1\frac{\tr(A)}{\gamma T}\left(\delta_1 + \cst_2\right),
% \end{align*}
% where $\cst_1 = \frac{4\sqrt{24}\kappa_1}{3}$ and $\cst_2 = 4\sigma^2 \kappa_2\left(\kappa_1+1\right)$.
% \arya[inline]{I should finish the proof by considering the case $T \leq T_1$.}
}
\end{proof}




% \newpage

% \section{So far the rest}
\begin{comment}
\begin{restatable}{lemma}{jkj}
\label{ma} Let Assumptions \ref{nat}(ii) and \ref{ass1} hold. Let $x_t$ and $\hat{g}_t$ be defined by Algorithm \ref{algo:grad} on $\com =\mathbb{R}^{d}$, then
\begin{align}\nonumber
    \Exp[f({x}_{t+1}) \mid x_t]
    \leq
    &\,f(x_{t}) -
    \parent{\frac{\eta_{t}}{2} - \frac{9L\kappa\eta_{t}^{2}}{2}}\norm{\nabla f(x_{t})}^{2}\\
    &
    +
    \frac{\eta_{t}}{2}(L\kappa_{\beta})^{2}dh_{t}^{2(\beta-1)}+\frac{3L\kappa \eta_{t}^{2}}{4} \parent{ \frac{\sigma^2}{h_{t}^2}+ \frac{3 {\bar L}^2}{2} h_{t}^2}d \enspace.
\end{align}
\end{restatable}


\jkj*
\begin{proof}
Since by the definition of Algorithm \ref{algo:grad}, $x_{t+1}=x_t-\eta_{t}\hat{g}_t$, by Assumption \ref{nat}(ii), we get
\begin{align}\label{golden}
    f(x_{t+1})\leq f(x_t)-\eta_{t}\langle \nabla f(x_t),\hat{g}_t\rangle + \eta_{t}^2\frac{L}{2}\norm{\hat{g}_t}^2.
\end{align}
On the other hand, we have 
\begin{align}\nonumber
    -\eta_{t}\Exp[\langle \nabla f(x_t), \hat{g}_{t}|x_t]\rangle &\leq -\eta_{t}\norm{\nabla{f}(x_{t})}^{2}-\eta_{t}\langle \nabla f(x_t),\Exp[ \hat{g}_{t}|x_t] - \nabla f(x_{t})\rangle \\\label{golden1}&\leq -\frac{\eta_{t}}{2}\norm{\nabla{f}(x_{t})}^{2}+\frac{\eta_{t}}{2}\norm{\Exp[\hat{g}_{t}|x_t]-\nabla{f}(x_{t})}^{2}.
\end{align}
Now by taking conditional expectation from both sides of inequality (\ref{golden}), applying Lemmas \ref{lem1new} and \ref{lem2new}, and using the bound (\ref{golden1}), we get
\begin{align*}
    \Exp[f(x_{t+1})|x_{t}] &\leq f(x_{t}) -\frac{\eta_{t}}{2}\norm{\nabla f(x_{t})}^{2} +\frac{\eta_{t}}{2}(L\kappa_{\beta})^{2}dh_{t}^{2(\beta-1)}+\\&\quad\quad\quad+\eta_{t}^{2}\frac{L}{2}\Big(\frac{3}{2} \kappa \left( \frac{\sigma^2}{h_{t}^2}+ \frac{3 {\bar L}^2}{2} h_{t}^2 \right)d + 9  \norm{\nabla f(x_{t})}^{2} \kappa\Big)\\&\leq f(x_{t})+ (-\frac{\eta_{t}}{2}+\frac{9L\kappa\eta_{t}^{2}}{2})\norm{\nabla f(x_{t})}^{2} +\frac{\eta_{t}}{2}(L\kappa_{\beta})^{2}dh_{t}^{2(\beta-1)}+\frac{3L\kappa \eta_{t}^{2}}{4} \left( \frac{\sigma^2}{h_{t}^2}+ \frac{3 {\bar L}^2}{2} h_{t}^2 \right)d.
\end{align*}
\end{proof}
\nc*
\begin{proof}
Let $\delta(t) = \Exp[f(x_t) - f^{\star}$], for $t = 1, \dots, T$. From Lemma \ref{golden}, we obtain
\begin{align*}
    \delta(t+1) \le \delta(t)+\Big(-\frac{\eta_{t}}{2}+\frac{9L\kappa \eta_{t}^2}{2}\Big)\Exp[\norm{\nabla f(x_t)}^2]+\eta_{t}B_{t}^2+\eta_{t}^2V_{t},
\end{align*}
where $$B_{t}^2 = \frac{(L\kappa_{\beta})^2}{2}dh_{t}^{2(\beta-1)},$$
and
$$V_{t} = \frac{3L\kappa}{4}\Big(\frac{\sigma^2}{h_{t}^2}+\frac{3\bar{L}^2}{2}h_{t}^2\Big)d.$$
Let $\gamma = d^{-\frac{\beta}{2\beta-1}}T^{-\frac{\beta}{2\beta-1}}$. Since $\eta_{t} = \min\big(\frac{1}{18L\kappa}, \gamma\big)$, then $-1+9L\kappa \eta_t \leq -\frac{1}{2}$. So that
\begin{align*}
    \delta(t+1) \leq \delta(t) -\frac{\eta_t}{4}\Exp[\norm{\nabla f(x_{t})}^2]+\eta_{t}B_t^{2}+\eta_{t}^2V_t.
\end{align*}
By rearranging terms and summing both sides from $1$ to $T$, we get
\begin{align*}
    \sum_{t=1}^{T}\eta_t\Exp[\norm{\nabla f(x_t)}^2]&\leq 4\sum_{t=1}^{T}\Big(\delta(t) - \delta(t+1)\Big)+4\sum_{t=1}^{T}\eta_tB_{t}^{2}+4\sum_{t=1}^{T}\eta_{t}^2V_t\\&=4\delta(1)+4\sum_{t=1}^{T}\eta_tB_{t}^{2}+4\sum_{t=1}^{T}\eta_{t}^2V_t.
\end{align*}
Now, by the definition of random variable $S$, we have
\begin{align}\label{jhg4}
    \Exp[\norm{\nabla f(x_S)}^2]&\leq \frac{4\delta(1)}{\sum_{k=1}^{T}\eta_k}+4\sum_{t=1}^{T}\frac{\eta_tB_{t}^{2}+\eta_{t}^2V_t}{\sum_{k=1}^{T}\eta_k},
\end{align}
where the later expectation is taken with respect to the joint probability distribution of all the random variables. On the other hand, for the term $\Big(\sum_{k=1}^{T}\eta_{k}\Big)^{-1}$, we have
\begin{align}\label{jhg5}
    \Big(\sum_{k=1}^{T}\eta_{k}\Big)^{-1}=\frac{1}{\min\Big(\frac{T}{18L\kappa}, T\gamma\Big)} =\max\Big(\frac{18L\kappa}{T},\frac{1}{T\gamma}\Big)\leq \frac{18L\kappa}{T}+\frac{1}{T\gamma}.
\end{align}
For the terms appear in the right hand side of (\ref{jhg4}), by (\ref{jhg5}) we get
\begin{align}\label{yt1}
    &\frac{4\delta(1)}{\sum_{k=1}^{T}\eta_{k}}\leq \frac{72L\kappa}{T}\delta(1)+\frac{4\delta(1)}{T\gamma},\\\label{yt2}
    &4\sum_{t=1}^{T}\frac{\eta_{t}B_{t}^2}{\sum_{k=1}^{T}\eta_{k}}\leq \mathcal{C}_{3}\sum_{t=1}^{T}\gamma d h_{t}^{2(\beta-1)}\Big(\frac{1}{T}+\frac{1}{T\gamma}\Big),\\\label{yt3}
    &4\sum_{t=1}^{T}\frac{\eta_{t}^2V_t}{\sum_{k=1}^{T}\eta_{k}}\leq \mathcal{C}_{4}\sum_{t=1}^{T}\gamma^2d\Big(\frac{\sigma^2}{h_{t}^2}+h_{t}^2\Big)\Big(\frac{1}{T}+\frac{1}{T\gamma}\Big),
\end{align}
where $\mathcal{C}_{3} = 2(18L\kappa + 1)(L\kappa_{\beta})^2$, and $\mathcal{C}_{4} = 3L\kappa(18L\kappa + 1)(1+\frac{3\bar{L}^2}{2})$. By replacing (\ref{yt1}), (\ref{yt2}), and (\ref{yt3}) in (\ref{jhg4}), we have
\begin{align}
    \Exp[\norm{\nabla f(x_S)}^2]&\leq \frac{72L\kappa\delta(1)}{T}+\mathcal{C}_{5}\sum_{t=1}^{T}\Big[\gamma d h_{t}^{2(\beta-1)}+\gamma^2d\Big(\frac{\sigma^2}{h_{t}^2}+h_{t}^2\Big)\Big]\frac{1}{T}+\\\label{opi1}&\quad\quad+\frac{4\delta(1)}{T\gamma}+\mathcal{C}_{5}\sum_{t=1}^{T}\Big[dh_{t}^{2(\beta-1)}+\gamma d \Big(\frac{\sigma^2}{h_{t}^2}+h_{t}^2\Big)\Big]\frac{1}{T},
\end{align}
where $\mathcal{C}_{5} = \mathcal{C}_{3}+\mathcal{C}_{4}$. By omitting the term with $h_{t}^2$ in (\ref{opi1}), the choose $\gamma$, $h_{t}$ to minimize
$$\frac{1}{T\gamma} + d\Big(h_{t}^{2(\beta-1)}+\frac{\gamma}{h_{t}^2}\Big).$$
The minimizers $\gamma$, and $h_{t}$ should satisfy
\begin{align*}
    \gamma=h_{t}^{2\beta},\quad\quad\gamma=\frac{h_{t}}{\sqrt{T d}}.
\end{align*}
So that 
\begin{align*}
    \gamma = (dT)^{-\frac{\beta}{2\beta-1}}, \quad\quad h_{t} = (dT)^{-\frac{1}{2(2\beta-1)}}.
\end{align*}
Now, since $\gamma < 1$, we have
\begin{align}\label{hji}
    \Exp[\norm{\nabla f(x_{S})}^2]\leq \frac{(72L\kappa + 4)\delta(1)}{T\gamma}+2\mathcal{C}_{5}\sum_{t=1}^{T}\Big[dh_{t}^{2(\beta-1)}+\gamma d\Big(\frac{\sigma^2}{h_{t}^2}+h_{t}^2\Big)\Big]\frac{1}{T}.
\end{align}
By replacing $\gamma$, and $h_{t}$ in (\ref{hji}), we get
\begin{align}
    \Exp[\norm{\nabla f(x_{S})}^2]\leq (\mathcal{C}_{1}\delta(1)+\mathcal{C}_{2})d^{\frac{\beta}{2\beta-1}}T^{-\frac{\beta-1}{2\beta-1}},
\end{align}
where $\mathcal{C}_{1} = 72L\kappa + 4$, and $\mathcal{C}_{2} = 2\mathcal{C}_{5}(2+\sigma^2)$.
\end{proof}
\ploptgoo*
\begin{proof}
Let $\delta(t) = \Exp[f(x_t)-f^{\star}]$. By Lemma \ref{ma}, we have 
\begin{align}\label{trar}
    \delta(t+1)&\leq \delta(t)+ (-\frac{\eta_{t}}{2}+\frac{9L\kappa\eta_{t}^{2}}{2})\norm{\nabla f(x_{t})}^{2} +\frac{\eta_{t}}{2}(L\kappa_{\beta})^{2}dh_{t}^{2(\beta-1)}+\frac{3L\eta_{t}^{2}}{4}\kappa \left( \frac{\sigma^2}{h_{t}^2}+ \frac{3 {\bar L}^2}{2} h_{t}^2  \right)d.
\end{align}
Now, by replacing $\norm{\nabla f(x_{t})}^{2}$, using $\alpha$-gradient dominancy of $f$, we get
\begin{align}\nonumber
    \delta(t+1)&\leq \delta(t)-\frac{\eta_{t}}{2}\delta(t)\alpha +\frac{\eta_{t}}{2}(L\kappa_{\beta})^{2}dh_{t}^{2(\beta-1)}+\frac{3L\eta_{t}^{2}}{4} \kappa\left( \frac{\sigma^2}{h_{t}^2}+ \frac{3 {\bar L}^2}{2} h_{t}^2  \right)d,
\end{align}
where we used the fact the $\eta_t \leq \frac{1}{18L\kappa}$. Furthermore, by letting $T_1 = \max\{k: k\leq \frac{36L\kappa}{\alpha}\}$, as $\eta_{t}=\frac{2}{\alpha t}$, for $t\geq T_{1}+1$, we have
\begin{align}\nonumber
    \delta(t+1)&\leq (1-\frac{1}{t})\delta(t) +\cst_{1}\frac{d}{\min\{\alpha,\alpha^{2}\}}t^{-\frac{2\beta-1}{\beta}},
\end{align}
where $\cst_{1} = (L\kappa_{\beta})^{2}+3L\kappa\left(\sigma^2+ \frac{3 {\bar L}^2}{2}  \right).$ Applying Lemma \ref{lemma:bis}, implies
\begin{align}\label{hyt}
    \delta(T)&\leq \frac{72L\kappa}{\alpha T}\delta(T_{1}+1) +\beta\cst_{1}\frac{d}{\min\{\alpha,\alpha^2\}}T^{-\frac{\beta-1}{\beta}}.
\end{align}
It remains to evaluate $\delta(T_{1}+1)$. For $t \leq T_{1}$, we have $\eta_{t}=\frac{1}{18L\kappa}$, so that 
\begin{align*}
    \frac{\eta_{t}}{2}(-1+9L\kappa \eta_{t})2\alpha=-\frac{\alpha}{36L\kappa}\leq -\frac{1}{T_{1}+1}.
\end{align*}
Therefore, by (\ref{trar}) for $t \in \{1,\dots, T_{1}\}$, we have 
\begin{align*}
    \delta(t+1)\leq (1-\frac{1}{T_{1}+1})\delta(t)+ U(t),
\end{align*}
where $U(t) = \frac{\eta_{t}}{2}(L\kappa_{\beta})^{2}dh_{t}^{2(\beta-1)}+\frac{3L\eta_{t}^{2}}{4}\kappa \left( \frac{\sigma^2}{h_{t}^2}+ \frac{3 {\bar L}^2}{2} h_{t}^2  \right)d.$
For any $a \in (0,1)$, we get that if for $1 \leq t \leq T_{1}$
\begin{align*}
    \delta(t+1)\leq (1-a)\delta(t)+U(t),
\end{align*}
then 
\begin{align*}
    \delta(T_{1}+1)&\leq (1-a)^{T_1}\delta(1)+\sum_{s=0}^{T_1}U(T_1-s+1)\\&\leq \delta(1)+\cst_{1}\frac{d}{\min\{\alpha, \alpha^2\}}\sum_{s=0}^{T_{1}}(1-a)^s(T_{1}-s+1)^{-\frac{2\beta-1}{\beta}}.
\end{align*}
Set $\rho = 1-a$. Then we have the following lemma (see \cite{SMA})
\begin{lemma}
Let $0<\rho<1$. Then 
$$\sum_{s=1}^{t}s^{-\frac{2\beta-1}{\beta}}\rho^{t-s}\leq (24\frac{2\beta-1}{\beta}+3(2^{\frac{\beta-1}{\beta}}))\frac{t^{-\frac{2\beta-1}{\beta}}}{1-\rho}.$$
\end{lemma}
Using this lemma we get
\begin{align*}
    \sum_{s=0}^{T_1}(1-a)^{s}(T_1-s+1)^{-\frac{2\beta-1}{\beta}}&=\sum_{m=1}^{T_{1}}\rho^{T_{1}-m+1}m^{-\frac{2\beta-1}{\beta}}+(T_{1}+1)^{-\frac{2\beta-1}{\beta}}\\&\leq (24\frac{2\beta-1}{\beta}+3(2^{\frac{\beta-1}{\beta}}))\frac{T_{1}^{-\frac{2\beta-1}{\beta}}}{a}+(T_{1}+1)^{-\frac{2\beta-1}{\beta}}\\&\leq\cst_2T_{1}^{-\frac{2\beta-1}{\beta}}(1+\frac{1}{a}).
\end{align*}
where $\cst_2=24\frac{2\beta-1}{\beta}+3(2^{\frac{\beta-1}{\beta}})+1$. Recall that $a = \frac{1}{T_{1}+1}$. Thus
$$\sum_{s=0}^{T_1}(1-a)^{s}(T_1-s+1)^{-\frac{2\beta-1}{\beta}}\leq \cst_3T_{1}^{-\frac{2\beta-1}{\beta}},$$
where $\cst_3 =2\cst_2$. Finally
$$\delta(T_1+1)\leq \delta(1)+\cst_{4}\frac{d}{\min\{\alpha, \alpha^2\}}T_{1}^{-\frac{2\beta-1}{\beta}},$$
where $\cst_4=\cst_1\cst_3$. By plugging this in (\ref{hyt}), we get
\begin{align}\label{hyt}
    \delta(T)&\leq \frac{72L\kappa}{\alpha T}\delta(1)+\cst_{4}\frac{d}{\min\{\alpha, \alpha^2\}T}T_{1}^{-\frac{\beta-1}{\beta}} +\beta\cst_{1}\frac{d}{\alpha}T^{-\frac{\beta-1}{\beta}}.
\end{align}
\end{proof}
\rsintheorem*
\begin{proof}
Suppose $x_{p} \in \argmin_{x \in \mathbb{R}^{d}} f(x)$. By the definition of the algorithm, we have 
\begin{align}\nonumber
    \norm{x_{t+1}-x_{p}}^{2} &= \norm{x_{t}-\eta_{t}\hat{g}_{t}-x_{p}}^2\\\nonumber
    &= \norm{x_{t}-x_{p}}^2-2\eta_{t}\langle \hat{g}_{t}, x_{t} -x _{p}\rangle+\eta_{t}^2\norm{\hat{g}_{t}}^2\\\label{juh10} &\leq (1- 2\eta_{t}\alpha)\norm{x_{t}-x_{p}}^2-2\eta_{t}\langle \hat{g}_{t} - \nabla f(x_t), x_{t} -x _{p}\rangle+\eta_{t}^2\norm{\hat{g}_{t}}^2,
\end{align}
where the last inequality is obtained form the fact that 
$$\alpha\norm{x_{t} - x_{p}}^{2} \leq \langle \nabla f(x_{t}), x_{t}-x_{p}\rangle.$$
Now, by the taking conditional expectation from both sides of (\ref{juh10}), we have
\begin{align}
    \Exp[a_{t+1}|x_{t}] \leq (1-2\eta_{t}\alpha)a_{t} -2\eta_t \langle \Exp[\hat{g}_{t}|x_{t}]-\nabla f(x_{t}), x_{t}-x_{p}\rangle +\eta_{t}^{2}\Exp[\norm{\hat{g}_{t}}^2|x_{t}],
\end{align}
where $a_{t} = \norm{x_{t}-x_{p}}^2$, for $1 \leq t \leq T$. On the other hand, we have
\begin{align}\nonumber
   -2\eta_t \langle \Exp[\hat{g}_{t}|x_{t}]-\nabla f(x_{t}), x_{t}-x_{p}\rangle &\leq 2\eta_{t} \norm{\Exp[\hat{g}_t|x_{t}]-\nabla f(x_t)}\norm{x_{t}-x_{p}} \\\nonumber&\leq
   \frac{\eta_{t}}{\alpha}\norm{\Exp[\hat{g}_t|x_{t}]-\nabla f(x_t)}^2 + \eta_{t} \alpha a_t&\\\label{plh12}&\leq \frac{2\eta_t}{\alpha}(L \kappa_\beta)^2 {d} h_{t} ^{2(\beta-1)}+ \frac{\eta_{t}}{2} \alpha a_t,
\end{align}
where the last inequality is a result of Lemma \ref{lem1new}. Taking total expectation, applying Lemma \ref{lem2new}, and plugging in (\ref{plh12}) in (\ref{juh10}), implies
\begin{align*}
    r_{t+1} \leq (1-\frac{3\eta_{t}}{2\alpha})r_{t} +\frac{2\eta_{t}}{\alpha}(L\kappa_{\beta})^2dh_{t}^{2(\beta-1)}+\eta_{t}^2\Big(\frac{3}{2} \kappa\left( \frac{\sigma^2}{h_{t}^2}+ \frac{3 {\bar L}^2}{2} h_{t}^2  \right)d + 9\norm{\nabla f(x_t)}^2 \kappa\Big),
\end{align*}
where $r_{t} = \Exp[a_{t}]$. Since, $\eta_t\leq \frac{\alpha}{18\bar{L}^2\kappa}$, then $9\eta_t^2\norm{\nabla f(x_t)}^2\leq \frac{\eta_t}{2\alpha}r_t$ Substituting $\eta_{t} = \frac{1}{\alpha t}$, and $h_{t} = t^{-\frac{1}{2\beta}},$ yields
\begin{align*}
    r_{t+1} \leq (1-\frac{1}{t})r_{t} +\mathcal{C}_{1}\frac{d}{\alpha^2}t^{-\frac{2\beta-1}{\beta}}+\frac{\mathcal{C}_{2}}{\alpha^2t^2},
\end{align*}
where $\mathcal{C}_{1} = 2(L\kappa_{\beta})^2+\frac{3}{2}\kappa(\sigma^2+\frac{3\bar{L}^2}{2})$, and $\mathcal{C}_{2}=9G^2\kappa$. By applying Lemma \ref{lemma:bis}, we get
\begin{align*}
    r_{t+1} \leq \frac{2r_1}{t}+\beta\mathcal{C}_{1}\frac{d}{\alpha^2}t^{-\frac{\beta-1}{\beta}}+\frac{\mathcal{C}_{2}}{\alpha^2 t}.
\end{align*}
On the other hand, by Assumption \ref{nat}(ii), we have
\begin{align*}
   \Exp[f(x_{t}) - f(x^*)]&\leq\frac{\bar{L}}{2} r_{t}\\& \leq \frac{\bar{L}r_1}{2t}+\frac{\bar{L}\beta\mathcal{C}_{1}}{4}\frac{d}{\alpha^2}t^{-\frac{\beta-1}{\beta}}+\frac{\bar{L}\mathcal{C}_{2}}{4\alpha^2 t}\\&\leq \frac{\bar{L}r_1}{2t}+\mathcal{C}\frac{d}{\alpha^2}t^{-\frac{\beta-1}{\beta}},
\end{align*}
where $\mathcal{C} = \frac{\bar{L}\beta\mathcal{C}_1}{4}+\frac{\bar{L}\mathcal{C}_2}{4}$.
\end{proof}
\rsitheorem*
\begin{proof}
Suppose $x_{p} \in \argmin_{x \in \mathbb{R}^{d}} f(x) \cap \com$. By the definition of the algorithm, we have 
\begin{align}\nonumber
    \norm{x_{t+1}-x_{p}}^{2} &\leq \norm{x_{t}-\eta_{t}\hat{g}_{t}-x_{p}}^2\\\nonumber
    &= \norm{x_{t}-x_{p}}^2-2\eta_{t}\langle \hat{g}_{t}, x_{t} -x _{p}\rangle+\eta_{t}^2\norm{\hat{g}_{t}}^2\\\label{juh1} &\leq (1- 2\eta_{t}\alpha)\norm{x_{t}-x_{p}}^2-2\eta_{t}\langle \hat{g}_{t} - \nabla f(x_t), x_{t} -x _{p}\rangle+\eta_{t}^2\norm{\hat{g}_{t}}^2,
\end{align}
where the last inequality is obtained form the fact that 
$$\alpha\norm{x_{t} - x_{p}}^{2} \leq \langle \nabla f(x_{t}), x_{t}-x_{p}\rangle.$$
Now, by the taking conditional expectation from both sides of (\ref{juh1}), we have
\begin{align}
    \Exp[a_{t+1}|x_{t}] \leq (1-2\eta_{t}\alpha)a_{t} -2\eta_t \langle \Exp[\hat{g}_{t}|x_{t}]-\nabla f(x_{t}), x_{t}-x_{p}\rangle +\eta_{t}^{2}\Exp[\norm{\hat{g}_{t}}^2|x_{t}],
\end{align}
where $a_{t} = \norm{x_{t}-x_{p}}^2$, for $1 \leq t \leq T$. On the other hand, we have
\begin{align}\nonumber
   -2\eta_t \langle \Exp[\hat{g}_{t}|x_{t}]-\nabla f(x_{t}), x_{t}-x_{p}\rangle &\leq 2\eta_{t} \norm{\Exp[\hat{g}_t|x_{t}]-\nabla f(x_t)}\norm{x_{t}-x_{p}} \\\nonumber&\leq
   \frac{\eta_{t}}{\alpha}\norm{\Exp[\hat{g}_t|x_{t}]-\nabla f(x_t)}^2 + \eta_{t} \alpha a_t&\\\label{plh11}&\leq \frac{\eta_t}{\alpha}(L \kappa_\beta)^2 {d} h_{t} ^{2(\beta-1)}+ \eta_{t} \alpha a_t,
\end{align}
where the last inequality is a result of Lemma \ref{lem1new}. Taking total expectation, applying Lemma \ref{lem2new}, and plugging in (\ref{plh11}) in (\ref{juh1}), implies
\begin{align*}
    r_{t+1} \leq (1-\eta_{t}\alpha)r_{t} +\frac{\eta_{t}}{\alpha}(L\kappa_{\beta})^2dh_{t}^{2(\beta-1)}+\eta_{t}^2\Big(\frac{3}{2} \kappa\left( \frac{\sigma^2}{h_{t}^2}+ \frac{3 {\bar L}^2}{2} h_{t}^2  \right)d + 9G^2 \kappa\Big),
\end{align*}
where $r_{t} = \Exp[a_{t}]$. Substituting $\eta_{t} = \frac{1}{\alpha t}$, and $h_{t} = t^{-\frac{1}{2\beta}},$ yields
\begin{align*}
    r_{t+1} \leq (1-\frac{1}{t})r_{t} +\mathcal{C}_{1}\frac{d}{\alpha^2}t^{-\frac{2\beta-1}{\beta}}+\frac{\mathcal{C}_{2}}{\alpha^2t^2},
\end{align*}
where $\mathcal{C}_{1} = (L\kappa_{\beta})^2+\frac{3}{2}\kappa(\sigma^2+\frac{3\bar{L}^2}{2})$, and $\mathcal{C}_{2}=9G^2\kappa$. By applying Lemma \ref{lemma:bis}, we get
\begin{align*}
    r_{t+1} \leq \frac{2B}{t}+\beta\mathcal{C}_{1}\frac{d}{\alpha^2}t^{-\frac{\beta-1}{\beta}}+\frac{\mathcal{C}_{2}}{\alpha^2 t}.
\end{align*}
On the other hand, by Assumption \ref{nat}(ii), we have
\begin{align*}
   \Exp[f(x_{t}) - f(x^*)]&\leq\frac{\bar{L}}{2} r_{t}\\& \leq \frac{\bar{L}B}{2t}+\frac{\bar{L}\beta\mathcal{C}_{1}}{4}\frac{d}{\alpha^2}t^{-\frac{\beta-1}{\beta}}+\frac{\bar{L}\mathcal{C}_{2}}{4\alpha^2 t}\\&\leq \frac{\bar{L}B}{2t}+\mathcal{C}\frac{d}{\alpha^2}t^{-\frac{\beta-1}{\beta}},
\end{align*}
where $\mathcal{C} = \frac{\bar{L}\beta\mathcal{C}_1}{4}+\frac{\bar{L}\mathcal{C}_2}{4}$.
\end{proof}
\fiftheorem*
\begin{proof}
From the definition of Algorithm \ref{algo:grad}, we have
\begin{align*}
    \langle \hat{g}_{t}, x_t-x^* \rangle = \frac{\norm{x_t-x^*}^2-\norm{x_{t+1}-x^*}^{2}}{\eta_t}+\frac{\eta_t}{2}\norm{\hat{g}_t}^{2}.
\end{align*}
By the strong convexity assumption, we get
\begin{align*}
    \Exp[f(x_t)-f^{\star}|x_t]\leq \norm{\Exp[\hat{g}_t|x_t]-\nabla f(x_t)}\norm{x_t-x^*}+\frac{1}{2\eta_t}\Exp[a_t - a_{t+1}|x_t]+\frac{\eta_{t}}{2}\Exp[\norm{\hat{g}_{t}}^2|x_t]-\frac{\alpha}{2}a_t,
\end{align*}
where $a_t = \norm{x_t-x^*}^2$. Now, by letting $r_{t} = \Exp\norm{x_t-x^*}^2$, applying Lemmas \ref{lem1new}, \ref{lem2new} and taking total expectation from both sides, we get
\begin{align}\nonumber
    \Exp[f(x_t)-f^{\star}]&\leq \kappa_{\beta}L\sqrt{d}h_{t}^{\beta-1}\Exp\norm{x_t-x^*}+\frac{1}{2\eta_t}(r_t-r_{t+1})+\frac{3\eta_t}{4} \kappa\left( \frac{\sigma^2}{h_{t}^2}+ \frac{3 {\bar L}^2}{2} h_{t}^2  \right)d +\\\nonumber&\quad\quad+ \frac{9\eta_t}{2}\bar{L}^2\kappa r_{t} -\frac{\alpha}{2}r_t\\\nonumber&\leq 2(\kappa_{\beta}L)^2\frac{d}{\alpha}h_{t}^{2(\beta-1)}+\frac{\alpha}{8}r_{t}+\frac{1}{2\eta_t}(r_t-r_{t+1})+\frac{3\eta_t}{4} \kappa\left( \frac{\sigma^2}{h_{t}^2}+ \frac{3 {\bar L}^2}{2} h_{t}^2  \right)d +\\\nonumber&\quad\quad+ \frac{9\eta_t}{2}\bar{L}^2\kappa r_{t} -\frac{\alpha}{2}r_t\\\label{pool4}&\leq 2(\kappa_{\beta}L)^2\frac{d}{\alpha}h_{t}^{2(\beta-1)}+\frac{1}{2\eta_t}(r_t-r_{t+1})+\frac{3\eta_t}{4} \kappa\left( \frac{\sigma^2}{h_{t}^2}+ \frac{3 {\bar L}^2}{2} h_{t}^2  \right)d  -\frac{\alpha}{4}r_t ,
\end{align}
where the last inequality is due to $\eta_{t} \leq \frac{\alpha}{36\bar{L}^2\kappa}$, and thus $\frac{9\eta_t}{2}\bar{L}^2\kappa r_{t} \leq \frac{\alpha}{8}r_t$. 

Let $T_{1} = \floor{\frac{72\bar{L}^2\kappa}{\alpha^2}}$. First, suppose that $T_{1} \le T$. Summing both sides from $T_{1}+1$ to $T$, yields
\begin{align*}
    \sum_{t=T_{1}+1}^{T}\Exp[f(x_{t})-f^{\star}]\leq \sum_{t=T_{1}+1}^{T}\Big[\frac{r_{t}-r_{t+1}}{2\eta_t} - \frac{\alpha}{4}r_t\Big]+\sum_{t=T_{1}+1}^{T}\Big[2(\kappa_{\beta}L)^2\frac{d}{\alpha}h_{t}^{2(\beta-1)}+\frac{3\eta_t}{4} \kappa\left( \frac{\sigma^2}{h_{t}^2}+ \frac{3 {\bar L}^2}{2} h_{t}^2  \right)d \Big],
\end{align*}
Now, by replacing $h_{t} = t^{-\frac{1}{2\beta}}$, and $\eta_{t} = \frac{2}{\alpha t}$, for $t = T_{1}+1,\dots,T$, we have
\begin{align}\label{hyt}
    \sum_{t=T_{1}+1}^{T}\Exp[f(x_{t})-f^{\star}]\leq \frac{\mathcal{B}_{3}}{\alpha}r_{T_{1}+1}+\mathcal{B}_{4}\frac{d}{\alpha}T^{1/\beta},
\end{align}
where $\mathcal{B}_{3} = 18\bar{L}^2\kappa$, $\mathcal{B}_{4} = 2\beta(\kappa_{\beta}L)^2+\frac{3}{2}\beta\kappa(\sigma^2+\frac{3\bar{L}^2}{2})$, and we use the fact
\begin{align*}
    \frac{\alpha}{4}\sum_{t=T_{1}+1}^{T}[t(r_{t}-r_{t+1})-r_{t}] \leq \frac{T_1\alpha}{4}r_{T_{1}+1}\leq \frac{18\bar{L}^2\kappa}{\alpha}r_{T_{1}+1}.
\end{align*}
Now, it is only enough to provide the upper bound for the term $r_{T_{1}+1}$. From (\ref{pool4}), for $1 \leq t \leq T$ we have
\begin{align}\label{pool}
    \Exp[f(x_{t})-f^{\star}]\leq \frac{1}{2\eta_{t}}\Big(r_{t}-r_{t+1}\Big)-\frac{\alpha}{4}r_t + \frac{\mathcal{B}_{4}}{\beta}\frac{d}{\alpha}t^{-\frac{\beta-1}{\beta}},
\end{align}
where we substitute $h_{t} = t^{-\frac{1}{2\beta}}$, and $\eta_{t} = \Big(\frac{\alpha}{36\bar{L}^2\kappa}, \frac{2}{\alpha t}\Big)$. Now, for $t \leq T_{1}$, by substituting $\eta_{t} = \frac{\alpha}{36\bar{L}^2\kappa}$ an rearranging terms, we get
\begin{align*}
    r_{t+1}\leq r_{t} + \frac{\mathcal{B}_4}{18\bar{L}^2\kappa\beta}dt^{-\frac{\beta-1}{\beta}},
\end{align*}
which yields 
\begin{align}\label{hyt3}
    r_{t+1}\leq r_{1} + \frac{\mathcal{B}_4}{18\bar{L}^2\kappa}dT_{1}^{\frac{1}{\beta}},
\end{align}
Now, by plugging in (\ref{hyt3}) in (\ref{hyt}), we have
\begin{align}\label{fin1}
    \sum_{t=T_{1}+1}^{T}\Exp[f(x_{t})-f^{\star}]\leq \frac{\mathcal{B}_{3}}{\alpha}r_{1}+\frac{\mathcal{B}_{3}\mathcal{B}_{4}}{18\bar{L}^2\kappa}\beta\frac{d}{\alpha} T_{1}^{\frac{1}{\beta}}+\mathcal{B}_{4}\frac{d}{\alpha}T^{\frac{1}{\beta}}.
\end{align}
On the other hand, from (\ref{pool}), we get
\begin{align}\label{fin2}
    \sum_{t=1}^{T_1}\Exp[f(x_t)-f^{\star}]\leq \frac{72\bar{L}^2\kappa}{\alpha}r_{1}+\mathcal{B}_{4}\frac{d}{\alpha}T_{1}^{\frac{1}{\beta}}.
\end{align}
Combining (\ref{fin1}) and (\ref{fin2}), implies
\begin{align}
    \sum_{t=1}^{T}\Exp[f(x_{t})-f^{\star}]\leq \frac{\mathcal{B}_1}{\alpha}r_{1}+\mathcal{B}_{6}\frac{d}{\alpha}+\mathcal{B}_{4}\frac{d}{\alpha}T^{\frac{1}{\beta}},
\end{align}
where $\mathcal{B}_{1} = \mathcal{B}_{3}+72\bar{L}^2\kappa$, and $\mathcal{B}_{6}=\mathcal{B}_{4}(72\kappa)^{\frac{1}{\beta}}\beta\Big(\frac{\mathcal{B}_{3}}{18\bar{L}^2\kappa}+1\Big)$. Here we use the fact that $T_{1} \leq 72\kappa$, since $\alpha \leq \bar{L}$.

In the case $T \leq T_{1}$, with the same steps that we obtain (\ref{fin2}), we get
\begin{align}
    \sum_{t=1}^{T}\Exp[f(x_t)-f^{\star}]\leq \frac{72\bar{L}^2\kappa}{\alpha}r_{1}+\mathcal{B}_{4} \frac{d}{\alpha}T^{\frac{1}{\beta}}.
\end{align}
Now, the final result can be conclude from convexity of $f$
\begin{align*}
    \Exp[f(\bar{x}_{T})-f^{\star}]\leq \frac{\mathcal{B}_{1}}{\alpha T}r_{1}+\mathcal{B}_{2}\frac{d}{\alpha}T^{-\frac{\beta-1}{\beta}},
\end{align*}
where $\mathcal{B}_{2} = \mathcal{B}_{6}+\mathcal{B}_{4}$.
\end{proof}
\thdtheorem*
\rsitheorem*
\begin{proof}
Suppose $x_{p} \in \argmin_{x \in \mathbb{R}^{d}} f(x) \cap \com$. By the definition of the algorithm, we have 
\begin{align}\nonumber
    \norm{x_{t+1}-x_{p}}^{2} &\leq \norm{x_{t}-\eta_{t}\hat{g}_{t}-x_{p}}^2\\\nonumber
    &= \norm{x_{t}-x_{p}}^2-2\eta_{t}\langle \hat{g}_{t}, x_{t} -x _{p}\rangle+\eta_{t}^2\norm{\hat{g}_{t}}^2\\\label{juh} &\leq (1- 2\eta_{t}\alpha)\norm{x_{t}-x_{p}}^2-2\eta_{t}\langle \hat{g}_{t} - \nabla f(x_t), x_{t} -x _{p}\rangle+\eta_{t}^2\norm{\hat{g}_{t}}^2,
\end{align}
where the last inequality is obtained form the fact that 
$$\alpha\norm{x_{t} - x_{p}}^{2} \leq \langle \nabla f(x_{t}), x_{t}-x_{p}\rangle.$$
Now, by the taking conditional expectation from both sides of (\ref{juh}), we have
\begin{align}
    \Exp[a_{t+1}|x_{t}] \leq (1-2\eta_{t}\alpha)a_{t} -2\eta_t \langle \Exp[\hat{g}_{t}|x_{t}]-\nabla f(x_{t}), x_{t}-x_{p}\rangle +\eta_{t}^{2}\Exp[\norm{\hat{g}_{t}}^2|x_{t}],
\end{align}
where $a_{t} = \norm{x_{t}-x_{p}}^2$, for $1 \leq t \leq T$. On the other hand, we have
\begin{align}\nonumber
   -2\eta_t \langle \Exp[\hat{g}_{t}|x_{t}]-\nabla f(x_{t}), x_{t}-x_{p}\rangle &\leq 2\eta_{t} \norm{\Exp[\hat{g}_t|x_{t}]-\nabla f(x_t)}\norm{x_{t}-x_{p}} \\\nonumber&\leq
   \frac{\eta_{t}}{\alpha}\norm{\Exp[\hat{g}_t|x_{t}]-\nabla f(x_t)}^2 + \eta_{t} \alpha a_t&\\\label{plh1}&\leq \frac{\eta_t}{\alpha}(L \kappa_\beta)^2 {d} h_{t} ^{2(\beta-1)}+ \eta_{t} \alpha a_t,
\end{align}
where the last inequality is a result of Lemma \ref{lem1new}. Taking total expectation, applying Lemma \ref{lem2new}, and plugging in (\ref{plh1}) in (\ref{juh}), implies
\begin{align*}
    r_{t+1} \leq (1-\eta_{t}\alpha)r_{t} +\frac{\eta_{t}}{\alpha}(L\kappa_{\beta})^2dh_{t}^{2(\beta-1)}+\eta_{t}^2\Big(\frac{3}{2} \kappa\left( \frac{\sigma^2}{h_{t}^2}+ \frac{3 {\bar L}^2}{2} h_{t}^2  \right)d + 9G^2 \kappa\Big),
\end{align*}
where $r_{t} = \Exp[a_{t}]$. Substituting $\eta_{t} = \frac{1}{\alpha t}$, and $h_{t} = t^{-\frac{1}{2\beta}},$ yields
\begin{align*}
    r_{t+1} \leq (1-\frac{1}{t})r_{t} +\mathcal{C}_{1}\frac{d}{\alpha^2}t^{-\frac{2\beta-1}{\beta}}+\frac{\mathcal{C}_{2}}{\alpha^2t^2},
\end{align*}
where $\mathcal{C}_{1} = (L\kappa_{\beta})^2+\frac{3}{2}\kappa(\sigma^2+\frac{3\bar{L}^2}{2})$, and $\mathcal{C}_{2}=9G^2\kappa$. By applying Lemma \ref{lemma:bis}, we get
\begin{align*}
    r_{t+1} \leq \frac{2B}{t}+\beta\mathcal{C}_{1}\frac{d}{\alpha^2}t^{-\frac{\beta-1}{\beta}}+\frac{\mathcal{C}_{2}}{\alpha^2 t}.
\end{align*}
On the other hand, by Assumption \ref{nat}(ii), we have
\begin{align*}
   \Exp[f(x_{t}) - f(x^*)]&\leq\frac{\bar{L}}{2} r_{t}\\& \leq \frac{\bar{L}B}{2t}+\frac{\bar{L}\beta\mathcal{C}_{1}}{4}\frac{d}{\alpha^2}t^{-\frac{\beta-1}{\beta}}+\frac{\bar{L}\mathcal{C}_{2}}{4\alpha^2 t}\\&\leq \frac{\bar{L}B}{2t}+\mathcal{C}\frac{d}{\alpha^2}t^{-\frac{\beta-1}{\beta}},
\end{align*}
where $\mathcal{C} = \frac{\bar{L}\beta\mathcal{C}_1}{4}+\frac{\bar{L}\mathcal{C}_2}{4}$.
\end{proof}

\begin{proof}
Fix an arbitrary $x \in \Theta$. By the definition of the algorithm, we have $\|x_{t+1} - x\|^2 \leq \|x_t-\eta_t \hat g_t - x\|^2$, which is equivalent to
\begin{equation}
\label{eq:GD} \langle {\hat g}_t , x_t - x\rangle \leq \frac{\|x_t-x\|^2- \|x_{t+1}- x]\|^2}{2 \eta_t} + \frac{\eta_t}{2} \|{\hat g}_t\|^2.
\end{equation}
%\mas{the above eq. could also be stated as a lemma if we use it multiple times}

By the strong convexity assumption we have
\begin{equation}
\label{eq:sconv}
f(x_t) - f(x) \leq \langle \nabla f(x_t),x_t - x\rangle -\frac{\alpha}{2} \|x_t - x\|^2.
\end{equation}
Combining the last two displays and setting $a_t = \|x_t-x\|^2$ we obtain
\begin{eqnarray}
%\Exp []
\nonumber
\Exp [ f(x_t) - f(x)  \hspace{.03truecm}|\hspace{.03truecm} x_t] & \leq & \|\Exp [{\hat g_t}  \hspace{.03truecm}|\hspace{.03truecm} x_t]-\nabla f(x_t)\|\|x_t - x\| + \frac{1}{2\eta_t}\Exp [a_t - a_{t+1}  \hspace{.03truecm}|\hspace{.03truecm}x_t] \\
\nonumber
&~& + \frac{\eta_t}{2} \Exp [\|{\hat g}_t\|^2  \hspace{.03truecm}|\hspace{.03truecm}x_t] -  \frac{\alpha}{2} \Exp [a_t  \hspace{.03truecm}|\hspace{.03truecm} x_t] \\ \nonumber
& \leq & \kappa_\beta L \sqrt{d} h_t^{\beta-1} \|x_t - x\| + \frac{1}{2\eta_t}\Exp [a_t - a_{t+1}  \hspace{.03truecm}|\hspace{.03truecm}x_t]\\
&~& + 
\frac{\eta_t}{2} \Exp [\|{\hat g}_t\|^2  \hspace{.03truecm}|\hspace{.03truecm}x_t]\label{eq:main}
%\frac{\eta_t}{2} \left(C L^2 d + \frac{3}{2} \frac{d^2}{h_t^2} \sigma^2 \right)  
-  \frac{\alpha}{2} \Exp [a_t  \hspace{.03truecm}|\hspace{.03truecm} x_t],
\end{eqnarray}
where the second inequality follows from Lemma \ref{lem1new}.  
As $2ab \leq a^2+b^2$ we have
\begin{equation}\label{eq:decouple}
  \sqrt{d} h_t^{\beta-1} \|x_t - x\| \leq \frac{1}{2} \Big( \frac{2\kappa_\beta L}{\alpha} d h_t^{2(\beta-1)}   + \frac{\alpha}{2\kappa_\beta L} \|x_t-x\|^2 \Big).
\end{equation}
%\leq L \frac{d^2}{\alpha} h_t^{2(\beta-1)} + \frac{1}{2L} (f(x_t) - f(x^*)) 
We conclude, taking the expectations and
letting 
$r_t = \Exp [a_t]$, that 
\begin{equation}
\label{eq:A}
%\frac{1}{2} 
\Exp [ f(x_t) - f(x)]  \leq \frac{r_t - r_{t+1}}{2\eta_t} - \frac{\alpha}{4} r_t + (\kappa_\beta L)^2 \frac{d}{\alpha} h_t^{2(\beta-1)} +
\frac{\eta_t}{2} \Exp [\|{\hat g}_t\|^2]%\frac{\eta_t}{2} \left(C L^2 d + \frac{3}{2} \frac{d^2}{h_t^2} \sigma^2 \right).
\end{equation}
%\sasha{Try to sum from $T/2$ to get rid of $\log T$}
Summing both sides over $t$ gives
$$
\sum_{t=1}^T \Exp [ f(x_t) - f(x)] \leq \frac{1}{2} \sum_{t=1}^T \left(\frac{r_t - r_{t+1}}{\eta_t} - \frac{\alpha}{2} r_t \right) + \sum_{t=1}^T \Big( (\kappa_\beta L)^2\frac{d}{\alpha} h_t^{2(\beta-1) }  +
\frac{\eta_t}{2} \Exp [\|{\hat g}_t\|^2]
\Big).
$$
The first sum on the r.h.s. is smaller than 0 for our choice of $\eta_t = \frac{2}{\alpha t}$. Indeed,
$$
%\frac{1}{2} 
\sum_{t=1}^T \left(\frac{r_t - r_{t+1}}{\eta_t} - \frac{\alpha}{2} r_t \right) \leq r_1\Big(\frac{1}{\eta_1}- \frac{\alpha}{2}\Big) + \sum_{t=2}^T r_t\left(\frac{1}{\eta_t} - \frac{1}{\eta_{t-1}} - \frac{\alpha}{2}\right)  = 0.
$$
From this remark and Lemma \ref{lem2new} (where we use that Assumption \ref{nat}(ii) implies $f\in\mathcal{F}_{2}(\bar L/2)$) we obtain 
\begin{eqnarray}
%\Exp []
\label{eq:basic}
 &&\sum_{t=1}^T \Exp [ f(x_t) - f(x)]  \leq  \frac{1}{\alpha} \sum_{t=1}^T 
  \left( (\kappa_\beta L)^2 d h_t^{2(\beta-1)}   + \frac{1}{t}\Exp [\|{\hat g}_t\|^2]\right) 
  \\ \nonumber
  && \qquad \leq  \frac{1}{\alpha} \sum_{t=1}^T 
  \left( (\kappa_\beta L)^2 d h_t^{2(\beta-1)}   + \frac{1}{t}\Big[
  9\kappa\Big(G^2  + \frac{{\bar L}^2dh_t^2}{8} \Big) + \frac{3\kappa d \sigma^2}{2h_t^2}\Big] \right) 
  \\ \label{eq:lll}
  && \qquad \leq  \frac{d}{\alpha} \sum_{t=1}^T \Big[\Big\{ (\kappa_\beta  L)^2 h_t^{2(\beta-1)} + \frac{3}{2} \frac{\kappa\sigma^2}{h_t^2 t}\Big\} + \frac{9\kappa {\bar L}^2h_t^2}{8t}\Big]  +  \frac{9\kappa G^2}{\alpha}  (\log T + 1).
  \label{eq:onl}
  \end{eqnarray}
If $\sigma>0$ then our choice of
$h_t = \left(\frac{3\kappa\sigma^2}{2(\beta-1) (\kappa_\beta L)^2} \right)^{\frac{1}{2\beta}} t^{-\frac{1}{2\beta}}
$ is the minimizer of the main term (in curly brackets in  \eqref{eq:onl}). 
Plugging this $h_t$ in \eqref{eq:onl} and using the fact that $\sum_{t=1}^T t^{-1+1/\beta}\le \beta T^{1/\beta}$
for $\beta\ge 2$
%\arya{I assume it should be $\sum_{t=1}^T t^{-1+1/\beta}\le \beta T^{1/\beta}.$} 
we get \eqref{eq:bound0}.
Inequality \eqref{eq:bound1} follows from \eqref{eq:bound0} in view of the convexity of $f$. 
If $\sigma=0$ the stochastic variability term in \eqref{eq:onl} disappears and one can choose $h_t$ as small as desired, in particular, such that the sum in \eqref{eq:onl} is smaller than $\frac{\kappa G^2}{\alpha} \log T$. This yields the bounds for $\sigma=0$.
%\eqref{eq:bound0a} and \eqref{eq:bound1a}. 
\end{proof}
\begin{lemma}
Let $f$ be Lipschitz continuous with constant $G>0$ in a Euclidean $h_t$-neighborhood of the set $\com$, and let Assumption \ref{ass1} (i) hold. Let ${\hat g}_t$ and $x_t$ be defined by Algorithm \ref{algo}.
Then
$$
\Exp [\|{\hat g}_t \|^2 \hspace{.04truecm}|\hspace{.04truecm} x_t] \leq \kappa\Big(C^* G^2 d +     \frac{3d^2}{2h_t^2}\sigma^2\Big),
$$
where $C^*>0$ is a numerical constant and $\kappa=\int K^2(u)du$. 
\label{lem:2}
\end{lemma}
\begin{proof}
We have 
\begin{align*}
 \|{\hat g}\|^2 &=  \frac{d^2}{4h^2} \|(f(x+h r\zeta) - f(x-hr\zeta) + \xi - \xi')\zeta K(r) \|^2 \\
 &= \frac{d^2}{4h^2} (f(x+h r\zeta) - f(x-hr\zeta) + \xi - \xi')^2 K^2(r).   
\end{align*}
Using the inequality $(a+b+c)^2 \leq 3 (a^2+b^2+c^2)$ we get
\begin{equation*}\label{var}
   \Exp [\|\hat g\|^2 \hspace{.03truecm}|\hspace{.03truecm} x] \leq \frac{3d^2}{4h^2} \left( \Exp[(f(x+hr \zeta) - f(x-hr\zeta) )^2K^2(r)] + 2 \kappa\sigma^2 \right). 
\end{equation*}
The lemma now follows by using  \cite[Lemma 10]{Shamir17}, which shows by a concentration argument that if $x\in\com$, $r\in [-1,1]$ are fixed, $\zeta$ is uniformly distributed on the unit sphere and $f$ is Lipschitz continuous with constant $G>0$ in a Euclidean $h$-neighborhood of the set $\com$, then
 $$
 \Exp[(f(x+hr \zeta) - f(x-hr\zeta) )^2] \leq c \frac{(hr)^2 G^2}{d}, 
$$
where $c>0$ is a numerical constant.
\end{proof}



%
%\mas{I think this lemma could be removed}

\begin{lemma}
%{sxthlemma}
\label{lem6.2}
	Let $f(\cdot)$ be a convex function on $\mathbb{R}^d$ and $h_t>0$. Then the following holds.
	\begin{itemize}
		\item[(i)] Function $\hat f_t(\cdot)$ is convex on $\mathbb{R}^d$.
		\item[(ii)] $\hat f_t(x)\ge f(x)$ for all $x\in \mathbb{R}^d$.
		\item[(iii)] Function $\hat f_t(\cdot)$ is differentiable on $\mathbb{R}^d$ and for the conditional expectation given $x_t$ we have
		$$
		\Exp[\hat g_t| x_t] = \nabla \hat f_t(x_t).
		$$
	\end{itemize}
\end{lemma}
\begin{proof}
	Item (i) is straightforward.  To prove item (ii), consider $g_t \in\partial f(x)$. Then,
	$$\hat f_t(x)\ge	\Exp \big[f(x)+ h_t\langle g_t, \tilde \zeta \rangle\big]
	= f(x)+ h_t\langle g_t, \Exp [\tilde \zeta] \rangle = f(x).
	$$
	For item (iii) we refer to \cite[][pg. 350]{NY1983}, or \cite{flaxman2004}. It is based on the fact that for any $x\in \mathbb{R}^d$ using Stokes formula we have
	\begin{align*}
	\nabla \hat f_t(x) &= \frac{1}{V(\mathbb{B}_{d})h_t^d} \int_{\norm{v}=h_t}f(x+v)\frac{v}{\norm{v}} {\rm d}s_{h_t}(v)= \frac{d}{V(S_d)h_t}\int_{\norm{u}=1}f(x+h_tu)u\, {\rm d}s_1(u) \\
	& = \frac{d}{V(S_d)h_t} \int_{\norm{u}=1}f(x+h_tu)u \,{\rm d}s_1(u) = \Exp \Big[  \frac{d}{h_t} f(x+h_t \zeta_t)\zeta_t \Big]%\\ 
	\end{align*}	
	where $V(\mathbb{B}_{d})$ is the volume of the unit ball $\mathbb{B}_{d}$,  ${\rm d}s_r(\cdot)$ is the element of spherical surface of raduis $r$ in $\mathbb{R}^d$, and $V(S_d)=d V(\mathbb{B}_{d})$ is the surface area of the unit sphere in $\mathbb{R}^d$. Since $f(x+h_t \zeta_t)\zeta_t $ has the same distribution as $f(x-h_t \zeta_t)(-\zeta_t)$ we also get  
	$$
	\Exp \Big[  \frac{d\big(f(x+h_t \zeta_t)-f(x-h_t \zeta_t)\big)\zeta_t }{2h_t}\Big] = \nabla \hat f_t(x).
	$$
\end{proof}

\begin{lemma}
%{svbthlemma}
\label{lem6.4}
If $f$ is $\alpha$-strongly convex then $ \hat  f_t$ is $\alpha$-strongly convex. 
	If $f\in \mathcal{F}_2(L)$ then for any $x\in\mathbb{R}^d$ and $h_t>0$ we have
	\begin{align}\label{lem6.4_1}
	| \hat f_t(x)- f(x)|  %\le \Exp| f(x+h_t \tilde \zeta)- f(x)| 
	\le  Lh_t^{2}. 
	\end{align}
	and
	\begin{align}\label{lem6.4_2}
	| \Exp  f(x\pm h_t\zeta_t) - f(x) | \le  Lh_t^{2}.
	\end{align}
\end{lemma}
\begin{proof}
Using the fact that $\Exp [\tilde \zeta] =0$ we have
$$
 |\Exp \big[f(x+h_t \tilde \zeta)- f(x)\big] | =  
 |\Exp \big[f(x+h_t \tilde \zeta)- f(x) - \langle\nabla f(x), h_t \tilde \zeta\rangle\big] |  \le  Lh_t^{2} \Exp [\|\tilde \zeta\|^{2}] \le Lh_t^{2}.
$$
Thus, \eqref{lem6.4_1} follows. The proof of \eqref{lem6.4_2} is analogous.
The $\alpha$-strong convexity of $\hat  f_t$ is equivalent to the relation 
\begin{align}\label{lem6.4_4}
\langle\nabla \hat f_t(x) - \nabla \hat f_t(x'), x-x'\rangle  \ge \alpha \norm{x- x'}^{2}, \quad \forall x,x'\in \mathbb{R}^d,  
\end{align}
which is proved as follows:
\begin{align}\label{lem6.4_5}
\langle\nabla \hat f_t(x) - \nabla \hat f_t(x'), x-x'\rangle & = \langle\Exp \big[\nabla f(x+h_t\tilde\zeta) - \nabla f(x'+h_t\tilde\zeta)\big], x-x'\rangle  \\ \nonumber
& =  \Exp \big[\langle \nabla f(x+h_t\tilde\zeta) - \nabla f(x'+h_t\tilde\zeta), (x+h_t\tilde\zeta)-(x'+h_t\tilde\zeta)\rangle \big]  \\
& \ge     \alpha \norm{x- x'}^{2}, \quad \forall x,x'\in \mathbb{R}^d, \nonumber
\end{align}
due to the $\alpha$-strong convexity of $f$.
%
\end{proof}
\eiththeorem*
\begin{proof}
Fix $x\in \com$. Due to the $\alpha$-strong convexity  of $\hat f_t$ (cf. Lemma \ref{lem6.4}) we have 
$$
\hat f_t(x_t) - \hat f_t(x) \le  \langle\nabla \hat f_t(x_t), x_t-x\rangle - \frac{\alpha}{2} \norm{x_t- x}^{2}.
$$
 Using \eqref{lem6.4_1} and Lemma \ref{lem6.2}(ii) we obtain
$$
f(x_t) - f(x) \le L h_t^2 + \langle\nabla \hat f_t(x_t), x_t-x\rangle - \frac{\alpha}{2} \norm{x_t- x}^{2}.
$$
Using this property and exploiting inequality~\eqref{eq:GD} we find, with an argument similar to the proof of Theorem \ref{thm:1}, that
\begin{align}\label{ef5a:th6.3}
\forall x\in \Theta: \qquad 	\Exp \big[f(x_t) - f(x)\big]  \le L h_t^2   + \frac{r_t-r_{t+1}}{2\eta_t} - \frac{\alpha}{2} r_t + \frac{\eta_t}{2} \Exp [\|{\hat g}_t \|^2 ].
\end{align}
By assumption, $\eta_t = \frac{1}{\alpha t}$. Summing up from $t=1$ to $T$ and reasoning again analogously to the proof of Theorem~\ref{thm:1} we obtain  
\begin{align}\label{ef6:th6.3}
\forall x\in \Theta: \qquad \Exp \sum_{t=1}^{T} \big(f(x_t) - f(x)\big)  
&\le \sum_{t=1}^{T} \Big( L h_t^2 +  \frac{1}{2\alpha t} \Exp [\|{\hat g}_t \|^2 ]\Big). 
\end{align}
Now, inspection of the proof of Lemma \ref{lem:2unco} shows that it remains valid with $\kappa=1$ when $K(\cdot)\equiv 1$ in Algorithm \ref{algo}. This yields 
$$
\Exp [\|{\hat g}_t \|^2 ] \leq 
9  \left(G^2 d + \frac{L^2d^2h_t^2}{2} \right) + \frac{3 d^2 \sigma^2}{2h_t^2}. 
$$
Thus,
\begin{align}\label{ef7:th6.3}
\forall x\in \Theta: \qquad \Exp \sum_{t=1}^{T} \big(f(x_t) - f(x)\big)  
&\le \sum_{t=1}^{T} \Big[ \Big( L +  \frac{9L^2d^2}{4\alpha t} \Big)h_t^2 
+ \frac{3 d^2 \sigma^2}{4h_t^2\alpha t}+
 \frac{9G^2d}{2\alpha t} \Big]. 
\end{align}
The chosen value $h_t= \left(\frac{3d^2\sigma^2}{4L\alpha t+9L^2d^2}\right)^{1/4}$ minimizes the r.h.s. and yields
\begin{align*}
\label{ef8:th6.3}
\forall x\in \Theta: \ \ \Exp \sum_{t=1}^{T} \big(f(x_t) - f(x)\big)  
&\le  \frac{3}{2}\sum_{t=1}^{T} 
\frac{d^2\sigma^2}{\alpha t}
\left(\frac{4L\alpha t+9L^2d^2}{3d^2\sigma^2}\right)^{1/2} + \frac{9G^2}{2}\frac{d}{\alpha} (1+\log T)
\nonumber \\
&\le 
\sum_{t=1}^{T} \sqrt{3} \Big[
\frac{d\sigma\sqrt{L}}{\sqrt{\alpha t}} + \frac{3Ld^2\sigma}{2\alpha t}  \Big]+ 9G^2 \frac{d}{\alpha} (1+\log T) \nonumber \\
& \le  2 \sqrt{3 L} \sigma 
\frac{d}{\sqrt{\alpha}} \sqrt{T} +  \Big(\frac{3\sqrt{3}}{2} \sigma L  +  \frac{9G^2}{d}  \Big) \frac{d^2}{\alpha} (1+\log T).
\end{align*}
As $1+\log T\le ((\log 2)^{-1}+1)\log T$ for any $T\ge 2$, we obtain  \eqref{eq1:th6.3}. On the other hand, we have the straightforward bound
\begin{equation}
\label{ef8:th6.3}
\forall x\in \Theta: \qquad \Exp \sum_{t=1}^{T} \big(f(x_t) - f(x)\big)  \le GBT.
\end{equation}
The remaining part of the proof follows the same lines as in Theorem \ref{thm:1}.  
%The bound \eqref{ef8:th6.3} is non-trivial only if $C'_4 \frac{d}{\sqrt{\alpha}} \sqrt{T}\le GBT$. In this case,  
\end{proof}
\begin{lemma}\label{gamma}
Suppose that $\zeta$ is a uniformly distributed random variable on the $(d-1)$-simplex. Then for any $0\leq\ell \leq 1$, we have $\Exp \norm{\zeta}^\ell \leq \Big(\frac{2}{d}\Big)^\frac{\ell}{2}.$
\end{lemma}
\begin{proof}
Note that if $Z_1,\dots,Z_d \sim^{i.i.d} \Gamma (1,1)$, then $\big(\frac{Z_1}{\sum_{j=1}^{d}Z_j},\dots,\frac{Z_d}{\sum_{j=1}^{d}Z_j}\big) =^{d} \zeta$. Also, we have $\big(\frac{Z_1}{\sum_{j=1}^{d}Z_j},\dots,\frac{Z_d}{\sum_{j=1}^{d}Z_j}\big)$ and $\sum_{j=1}^{d}Z_j$ are independent random variables. Therefore, we can write\evg{jensen in a wrong direction here}
\begin{align*}
    \Exp[\norm{\zeta}^\ell] &\leq \big(\Exp[\norm{\zeta}]^2\big)^\frac{\ell}{2}\\&= \Big(\sum_{i=1}^{d}\Exp\frac{Z_i^2}{\big(\sum_{j=1}^{d}Z_j\big)^2}\Big)^\frac{\ell}{2}\\&=\Big(\sum_{i=1}^{d}\Exp\frac{Z_i^2}{\big(\sum_{j=1}^{d}Z_j\big)^2}\Big)^\frac{\ell}{2}\Big(\frac{\big(\Exp\sum_{j=1}^{d}Z_j\big)^2}{\big(\Exp\sum_{j=1}^{d}Z_j\big)^2}\Big)^\frac{\ell}{2}\\&=\Big(\Exp\Big[\frac{\sum_{i=1}^{d} Z_i^2}{\big(\sum_{j=1}^{d}Z_j\big)^2}.\big(\sum_{j=1}^{d}Z_j\big)^2\Big]\Big)^\frac{\ell}{2}\Big(\frac{1}{\big(\sum_{j=1}^{d}\Exp Z_j\big)^2}\Big)^\frac{\ell}{2}\\&=\Big(\frac{d\Exp Z_{1}^2}{d(d-1)\Exp [Z_1]\Exp[Z_2] + d\big(\Exp Z_1\big)^2}\Big)^\frac{\ell}{2}\\&= \Big(\frac{2}{d}\Big)^\frac{\ell}{2},
\end{align*}
where the first inequality is ordained from Jensen's inequality and we used the fact that $\Exp Z_1^2 = 2$, $(\Exp Z_1)^2 = 1$ and $\Exp Z_1\Exp Z_2 =1$.
\end{proof}
\end{comment}





\newpage
\section{Lower bounds}
\begin{proof}[Proof of Lemma~\ref{lem:hellinger_lower}]
Observe that since the noise $\xi_1, \ldots, \xi_T$ is assumed to be independent, the following decomposition holds
\begin{align*}
    \d\mathbf{P}_f = \d F(y_1 - f(\bz_1))\prod_{t = 2}^T \d F\bigg(y_t - f\Big(\Phi_{t}(\bz_1, y_1, \ldots, y_{t - 1})\Big) \bigg)\enspace.
\end{align*}

Introduce for compactness
\begin{align*}
    \d F_{f, t} \triangleq \d F\bigg(y_t - f\Big(\Phi_{t}(\bz_1, y_1, \ldots, y_{t - 1})\Big) \bigg)\enspace,
\end{align*}
then in this notation we have $\d\mathbf{P}_f = \prod_{t = 1}^T \d F_{f, t}$.
Analogously, the same holds for $\mathbf{P}_{f'}$.
Using the definition of the Hellinger distance we can write
\begin{align*}
   1 {-} \frac{1}{2}H^2(\mathbf{P}_{f} , \mathbf{P}_{f'})
    &=
    \int\sqrt{\d\mathbf{P}_{f}\d\mathbf{P}_{f'}}
    =\prod_{t=1}^{T}\int \sqrt{\d F_{f, t}}\sqrt{\d F_{f', t}}
    =
    \prod_{t = 1}^T\parent{1 - \frac{H^2\parent{\d F_{f, t}, \d F_{f', t}}}{2}}\enspace.
    % \\
    % &=\Big(1- \prod_{i=1}^{T}\big(1 - \frac{H^2(\d F_{\omega, i}, \d F_{\omega', i})}{2}\big)\Big)\\&\leq \Big(1-\min_{1 \leq i \leq T}\big(1-\frac{H^{2}(\d F_{\omega,i},dF_{\omega^{'},i})}{2}\big)^{T}\Big)\\&\leq \Big(1-\min_{u \in \com^{'}}\big(1-\frac{I_{0}|f_{\omega}(u)-f_{\omega'}(u)|^2}{2}\big)^{T}\Big) \\&= \Big(1-\big(1-\max_{u\in\com^{'}}\frac{I_{0}|f_{\omega}(u)-f_{\omega'}(u)|^2}{2}\big)^{T}\Big)\\&\AK{\leq \Big(1 - \big(1-\frac{I_{0}r^{2}h^{2\beta}\eta(1/\sqrt{d})}{2}\big)\Big)}
\end{align*}
Finally, invoking the assumption on the cumulative distribution of the noise, we get
\begin{align*}
    \prod_{t = 1}^T\parent{1 - \frac{H^2\parent{\d F_{f, t}, \d F_{f', t}}}{2}}
    &\geq
    \min_{1 \leq t \leq T}\parent{1 - \frac{H^2\parent{\d F_{f, t},  \d F_{f', t}}}{2}}^T\\
    &\geq
    \parent{1 - \max_{\bu \in \Theta}\frac{I_0|f(\bu) - f'(\bu)|}{2}}^T\enspace.
\end{align*}
Substituting into the penultimate equality and rearranging we conclude.
\end{proof}



\begin{proof}[Proof of Theorem~\ref{lb}]
We first assume that $\alpha\ge T^{-1/2+1/\beta}$.

Let $\eta_{0} : \mathbb{R} \to \mathbb{R}$ be an infinitely many times differentiable function such that
\begin{equation*}
   \eta_{0}(x) = \begin{cases}
      =1 & \text{if $|x|\leq 1/4$},\\
      \in (0,1) & \text{if $1/4 < |x| < 1$},\\
      =0 & \text{if $|x| \geq 1$}.
    \end{cases} 
\end{equation*}
Set $\eta(x) = \int_{-\infty}^{x} \eta_{0}(\tau)d\tau$. Let $\Omega = \big\{-1,1\big\}^{d}$ be the set of binary sequences of length $d$. 
Consider the finite set of functions $f_{\omega}: \mathbb{R}^{d}\to \mathbb{R}, \bomega = (\omega_1, \ldots, \omega_d)\in\Omega$, defined as follows:
\[
f_{\bomega}(\bu) = \alpha(1+\delta) \norm{\bu}^{2}/2 + \sum_{i=1}^{d}\omega_{i}rh^{\beta}\eta(u_{i}h^{-1}),
\qquad \bu=(u_1,\dots,u_d),
\]
where $\omega_i\in \{-1,1\}$, 
 $h =\min\big((\alpha^2/d)^{\frac{1}{2(\beta-1)}}, T^{-\frac{1}{2\beta}}\big)$ and $r>0, \delta >0$ are fixed numbers that will be chosen small enough. 
 
 Let us prove that $f_{\bomega}\in\mathcal{F}'_{\alpha,\beta}$
 for $r>0$ and $\delta >0$ small enough. It is straightforward to check that if $r$ is small enough the functions $f_{\bomega}$ are $\alpha$-strongly convex
 and belong to $\mathcal{F}_{\beta}(L)$.
 
 Next, the components of the gradient $\nabla f_{\bomega}$ have the form
 $$( \nabla f_{\bomega}(\bu))_{i} = \alpha (1 + \delta)u_{i}+\omega_{i}r h^{\beta-1}\eta_0(u_{i}h^{-1}).$$
 Thus, 
 $$\norm{\nabla f_{\bomega} (\bu)}^2\le 2\alpha^2 (1 + \delta)^2\norm{\bu}^{2} + 2 r^2 \alpha^2
 $$
and the last  expression can be rendered smaller than $G^2$ uniformly in $\bu\in \com$ by the choice of $\delta$ and $r$ small enough since $G^2> 4\alpha^2 $. 

Finally, we check that the minimizers of functions $f_{\bomega}$ belong to $\com$.  
Notice that we can choose $r$ small enough to have
$\alpha^{-1}(1+\delta)^{-1}rh^{\beta-2}<1/4$
and that under this condition 
 the equation $\nabla f_{\omega}(\bx) = 0$
has the solution $$\bx_{\bomega}^{*} = (x^*(\omega_1), \dots, x^*(\omega_d)), $$
where $x^*(\omega_i)=-\omega_{i}\alpha^{-1}(1+\delta)^{-1}r h^{\beta-1}$.
Using the definition of $h$ we obtain
$$
\norm{\bx_{\bomega}^{*}}\le d^{1/2}  \alpha^{-1}(1+\delta)^{-1}r h^{\beta-1} \le d^{1/2}  \alpha^{-1}(1+\delta)^{-1}r (\alpha^2/d)^{1/2}\le (1+\delta)^{-1}r <1
$$
for $r>0$ small enough, which means that $\bx_{\bomega}^{*}$ belongs to the interior of $\com$.

Combining all the above remarks we conclude that the family of functions $\{f_{\bomega} \,:\, \bomega\in\Omega\}$ is a subset of $\mathcal{F}'_{\alpha,\beta}$ for $r>0$ and $\delta >0$ small enough. 


%In what follows, assume that $\omega_i\in \{-1,1\}$, $i=1,\dots,d$, are independent random variables taking values in $\{-1,1\}$ with probability $1/2$. We also assume that the random vector $(\omega_{1},\dots,\omega_{d})$ is independent from  $(x_{1},\dots,x_{T}, y_{1},\dots,y_{T})$.

For any fixed $\bomega\in\Omega$, we denote by $\mathbf{P}_{\bomega,T}$ the probability measure corresponding to the joint distribution of $(\bz_1,y_{1},\dots,y_{T})$ where $y_{t}=f_{\bomega} (\bz_{t})+\xi_{t}$ with independent identically distributed $\xi_{t}$'s such that \eqref{distribution} holds and $\bz_t$'s chosen by a sequential strategy in $\Pi_T$. 
% We have
% $$
% d\mathbf{P}_{\omega,T}(z_1,y_{1},\dots,y_{T})
% =dF\big(y_{1}-f_\omega(z_{1})\big)\prod_{i=2}^{T}\d F\Big(y_{i}-f_\omega\big(\Phi_i(z_1, y_1,\dots,y_{i-1})\big)\Big).
% $$
% Without loss of generality, we omit here the dependence of $\Phi_{i}$ on $z_{2},\dots,z_{i-1}$ since $z_{i}, i\ge 2,$ is a Borel function of $z_1,y_{1},\dots,y_{i-1}$.
% Let $\mathbf{E}_{\omega,T}$ denote the expectation w.r.t. $\mathbf{P}_{\omega,T}$.%, and $\Exp_{\omega}$ the expectation w.r.t. the  distribution of $\omega=(\omega_1,\dots,\omega_d)$.

Consider the statistic
$$\hat{\bomega} \in \argmin_{\bomega \in \Omega} \norm{\bz_{T}-\bx^{*}_{\bomega}}.$$
Since
$\norm{\bx^{*}_{\hat{\bomega}}-\bx^{*}_{{\bomega}}}\leq \norm{\bz_{T}-\bx^{*}_{{\bomega}}}+\norm{\bz_{T} - \bx^{*}_{\hat{\bomega}}}\leq 2\norm{\bz_{T}-\bx^{*}_{\bomega}}$
for all $\bomega \in \Omega$ we obtain
\begin{align*}
    \mathbf{E}_{\bomega,T}\big[\norm{\bz_{T}-\bx^{*}_{\bomega}}^{2}\big] &\geq \frac{1}{4}\mathbf{E}_{\bomega,T}\big[\norm{\bx_{\bomega}^{*}-\bx_{\hat{\bomega}}^{*}}^{2}\big]
    =\alpha^{-2}r^{2} h^{2\beta-2}\mathbf{E}_{\bomega,T}\rho(\hat{\bomega},\bomega)\enspace,
\end{align*}
where $\rho(\hat{\bomega},\bomega)= \sum_{i=1}^{d}\mathbb{I}(\hat{\omega}_i\ne\omega_i)$ is the Hamming distance between $\hat{\bomega}$ and $\bomega$. Taking the maximum over $\Omega$ and then the minimum over all statistics $\hat{\bomega}$ with values in $\Omega$ we obtain
$$\max_{\bomega \in \Omega}\mathbf{E}_{\bomega,T}\big[\norm{\bz_{T}-\bx^{*}_{\bomega}}^{2}\big] \geq \alpha^{-2}r^{2} h^{2\beta-2}\inf_{\hat{\bomega}}\max_{\bomega \in \Omega}\mathbf{E}_{\bomega,T} \rho(\hat{\bomega},\bomega).$$
 By \cite[Theorem 2.12]{Tsybakov09}, if for some $0<\gamma\leq 2$ and all $\bomega, \bomega'\in \Omega$ such that $\rho(\bomega, \bomega')=1$ we have $H^2(\mathbf{P}_{\bomega,T} , \mathbf{P}_{\bomega',T})\leq \gamma$, where  $H^2(\cdot,\cdot)$ denotes the Hellinger distance, then 

\begin{align}
    \label{eq:Tsybakov_hellinger}
    \inf_{\hat{\bomega}}\max_{\bomega \in \Omega}\mathbf{E}_{\bomega, T}\left[ \rho(\hat{\bomega},\bomega) \right]\geq \frac{d}{2}\Big(1-\sqrt{\gamma(1-\gamma/4)}\Big)\enspace.
\end{align}
 Note that for all $\bomega, \bomega'\in \Omega$ such that $\rho(\bomega, \bomega')=1$ we have
\[
\max_{\bu\in\mathbb{R}^d}{|f_{\bomega}(\bu)-f_{\bomega'}(\bu)|}\leq 2rh^{\beta} \eta(1) \leq 2rT^{-1/2} \eta(1)\enspace.
\]
Thus, letting $2r<\big(v_{0}/\eta(1)\big)T^{1/2}$ to ensure that $2rT^{-1/2} \eta(1) \leq v_0$ we apply Lemma~\ref{lem:hellinger_lower} and deduce for such $\bomega, \bomega' \in \Omega$ that
\begin{align*}
    H^2(\mathbf{P}_{\bomega,T} , \mathbf{P}_{\bomega',T})&\leq 2\Big(1 - \big(1 - T^{-1}\big)^T\Big)
    \leq
    2\left(1-\frac{1}{
    4}\right)= 3/2\enspace.
\end{align*}
 Thus, by Eq.~\eqref{eq:Tsybakov_hellinger} we deduce that
\[
\inf_{\hat{\bomega}}\max_{\bomega \in \Omega}\mathbf{E}_{\bomega, T} [\rho(\hat{\bomega},\bomega)]\geq 0.01 \times d\enspace.
\]
Therefore, we have proven that if $\alpha\ge T^{-1/2+1/\beta}$ then there exist $r>0$ and $\delta >0$ small enough such that  
\begin{equation}\label{eq3:lb}
 \max_{\bomega \in \Omega}\mathbf{E}_{\bomega,T}\big[\norm{\bz_{T}-\bx^{*}_{\bomega}}^{2}\big]\geq 0.001 \times d\alpha^{-2}r^{2} h^{2\beta-2} = 0.01 \times r^{2}\min\Big(1, 
\,\frac{d}{\alpha^{2}}T^{-\frac{\beta-1}{\beta}}
\Big)\enspace.   
\end{equation}
This implies \eqref{eq2:lb} for $\alpha\ge T^{-1/2+1/\beta}$. In particular, if $\alpha=\alpha_0:= T^{-1/2+1/\beta}$ the bound \eqref{eq3:lb} is of the order $\min\Big(1, {d}{T^{-\frac{1}{\beta}}}
\Big)$. Then for $0<\alpha<\alpha_0$ we also have the bound of this order since the classes $\mathcal{F}'_{\alpha,\beta}$ are nested: $\mathcal{F}'_{\alpha_0,\beta}\subset \mathcal{F}'_{\alpha,\beta}$. This completes the proof of \eqref{eq2:lb}. 

We now prove \eqref{eq1:lb}. From \eqref{eq3:lb} and $\alpha$-strong convexity of $f$ we get that, for $\alpha\ge T^{-1/2+1/\beta}$,
\begin{equation}\label{eq4:lb}
\max_{\bomega \in \Omega}\mathbf{E}_{\bomega,T}
\big[f(\bz_T)-f(x_{\bomega}^*)\big]\geq
0.005 \times r^{2}\min\Big(\alpha, 
\,\frac{d}{\alpha}T^{-\frac{\beta-1}{\beta}}
\Big)\enspace.  
\end{equation}
This implies \eqref{eq1:lb} in the zone $\alpha\ge T^{-1/2+1/\beta}$ since for such $\alpha$ we have
\[
\min\Big(\alpha, 
\,\frac{d}{\alpha}T^{-\frac{\beta-1}{\beta}}
\Big)
=
\min\Big(\max(\alpha, T^{-1/2+1/\beta}), \frac{d}{\sqrt{T}}, \,\frac{d}{\alpha}T^{-\frac{\beta-1}{\beta}}\Big)\enspace.
\]
On the other hand, 
\[
\min\Big(\alpha_0, 
\,\frac{d}{\alpha_0}T^{-\frac{\beta-1}{\beta}}
\Big)
=
\min\Big(T^{-1/2+1/\beta}, \frac{d}{\sqrt{T}} \Big)\enspace,
\]
and the same lower bound holds for $0<\alpha<\alpha_0$  by the nestedness argument that we used to prove \eqref{eq2:lb} in the zone $0<\alpha<\alpha_0$. Thus, \eqref{eq1:lb} follows.

\end{proof}

\begin{proof}[Proof of Theorem~\ref{thm:lower_quadratic}]

\evg[inline]{Todo: erase upperscript for $'$; refer to to lemma; make things bold (done)}
Let $\Pi_{T}'$ be the class of sequential strategies such that $\pi{'} \in \Pi_{T}'$ if and only if for all $1 \leq i \leq T$, $\bz'_{i} \in \Theta$, where $\bz'_{i}$ is the $i$-th output of $\pi$. By projecting the outputs on $\Theta$ it is clear that for any $\pi \in \Pi_{T}$, there exists $\pi{'} \in \Pi{'}_{T}$, such that 
\[
\sup_{f \in L^{'}}\Exp[f(\bz_{T})-f^{\star}] \geq \sup_{f \in L{'}}\Exp[f(\bz'_{T})-f^{\star}]\enspace,
\]
\evg[inline]{What is $L'$??}
where $\bz_{T}$ and $\bz'_{T}$ are the outputs of $\pi$ and $\pi'$, respectively.

Let $\bomega = \{-1,1\}^d$ be the set of binary sequences with length $d$. Consider the set of quadratic functions $f_{\bomega}:\mathbb{R}^d \to \mathbb{R}$, be defined as follows:
$$f_{\bomega}(\bu) = \frac{\alpha}{2}\norm{\bu}^2 + hr\sum_{i=1}^{d}\omega_{i}u_{i},$$
where $\omega_{i} \in\{-1, 1\}$, $h = \min\Big(\frac{\alpha}{\sqrt{d}}, \frac{1}{\sqrt{T}}\Big)$, and $r>0$ is a fixed number that will be chosen small enough. First note that $f_{\bomega}$ is $\alpha$-strongly convex for all $\bomega \in \Omega$. Also, the components of the gradient have the form
\[
\Big(\nabla f_{\bomega}(\bu)\Big)_{j} = \alpha u_{j} + hr\omega_{j}\enspace.
\]
Therefore, $\bx_{\bomega}^{*} = \Big(-\frac{hr\omega_{1}}{\alpha},\dots, -\frac{hr\omega_{d}}{\alpha}\Big).$ By the choice of $h$, we have $\bx_{\bomega}^{*}$ belongs to the interior of $\Theta$. 

For any fixed $\bomega\in\Omega$, we denote by $\mathbf{P}_{\omega,T}$ the probability measure corresponding to the joint distribution of $(\bz_1,y_{1},\dots,y_{T})$ where $y_{t}=f_{\bomega} (\bz_{t})+\xi_{t}$ with independent identically distributed $\xi_{t}$'s such that \eqref{distribution} holds and $\bz_t$'s chosen by a sequential strategy in $\Pi_T^{'}$. 
We have
$$
\d\mathbf{P}_{\omega,T}(\bz_1,y_{1},\dots,y_{T})
=\d F\big(y_{1}-f_\omega(\bz_{1})\big)\prod_{i=2}^{T}\d F\Big(y_{i}-f_\omega\big(\Phi_i(\bz_1, y_1,\dots,y_{i-1})\big)\Big).
$$
Without loss of generality, we omit here the dependence of $\Phi_{i}$ on $\bz_{2},\dots,\bz_{i-1}$ since $\bz_{i}, i\ge 2,$ is a Borel function of $\bz_1,y_{1},\dots,y_{i-1}$.
Let $\mathbf{E}_{\bomega,T}$ denote the expectation w.r.t. $\mathbf{P}_{\bomega,T}$.%, and $\Exp_{\omega}$ the expectation w.r.t. the  distribution of $\omega=(\omega_1,\dots,\omega_d)$.

Consider the statistic
$$\hat{\bomega} \in \argmin_{\bomega \in \Omega} \norm{\bz_{T}-\bx^{*}_{\bomega}}.$$
Since
$\norm{\bx^{*}_{\hat{\bomega}}-\bx^{*}_{{\bomega}}}\leq \norm{\bz_{T}-\bx^{*}_{{\bomega}}}+\norm{\bz_{T} - \bx^{*}_{\hat{\bomega}}}\leq 2\norm{\bz_{T}-\bx^{*}_{\bomega}}$
for all $\bomega \in \Omega$ we obtain
\begin{align*}
    \mathbf{E}_{\bomega,T}\big[\norm{\bz_{T}-\bx^{*}_{\bomega}}^{2}\big] &\geq \frac{1}{4}\mathbf{E}_{\bomega,T}\big[\norm{\bx_{\bomega}^{*}-\bx_{\hat{\bomega}}^{*}}^{2}\big]
    =\alpha^{-2}r^{2} h^{2}\mathbf{E}_{\omega,T}[\rho(\hat{\bomega},\bomega)]\enspace,
\end{align*}
where $\rho(\hat{\bomega},\bomega)= \sum_{i=1}^{d}\mathbb{I}(\hat{\omega}_i\ne\omega_i)$ is the Hamming distance between $\hat{\bomega}$ and $\bomega$. Taking the maximum over $\Omega$ and then the minimum over all statistics $\hat{\bomega}$ with values in $\Omega$ we obtain
\begin{align}
\label{eq:lower_bound_quadratic1}
\max_{\bomega \in \Omega}\mathbf{E}_{\bomega,T}\big[\norm{\bz_{T}-\bx^{*}_{\bomega}}^{2}\big] \geq \alpha^{-2}r^{2} h^{2}\inf_{\hat{\bomega}}\max_{\bomega \in \Omega}\mathbf{E}_{\bomega}[] \rho(\hat{\bomega},\bomega)]\enspace.
\end{align}
%  By \cite[Theorem 2.12]{Tsybakov09}, if for some $0<\gamma\leq 2$ and all $\omega, \omega'\in \Omega$ such that $\rho(\omega, \omega')=1$ we have $H^2(\mathbf{P}_{\omega,T} , \mathbf{P}_{\omega',T})\leq \gamma$, where  $H^2(\cdot,\cdot)$ denotes the Hellinger distance, then 
% $$\inf_{\hat{\omega}}\max_{\omega \in \Omega}\mathbf{E}_{\omega, T} \rho(\hat{\omega},\omega)\geq \frac{d}{2}\Big(1-\sqrt{\gamma(1-\gamma/4)}\Big).$$
% For the sake of simplicity, let $F_{\omega, 1} = F(y_{1} - f_{\omega}(z_{1}))$, and $F_{\omega, i}=F(y_{i}-f_{\omega}\big(\Phi_{i}(z_1, y_{1}^{i-1})\big))$, for all $\omega \in \Omega$, and $2\leq i\leq T$.
For all $\bomega, \bomega'\in \Omega$ such that $\rho(\bomega, \bomega')=1$, we have $\max_{\bu\in\com}{|f_{\omega}(\bu)-f_{\omega'}(\bu)|^2}\leq r^2T^{-1} \leq v_0$ with the last inequality being satisfied as long as $r < v_0 T^{1/2}$. Therefore, applying Lemma~\ref{lem:hellinger_lower} we deduce that 
\begin{align*}
    H^2(\mathbf{P}_{\omega,T} , \mathbf{P}_{\omega',T})
    \leq
    % &= 2\Big(1-\int\sqrt{d\mathbf{P}_{\omega,T}d\mathbf{P}_{\omega',T}}\Big) \\
    % &=2\Big(1 - \prod_{i=1}^{T}\int \sqrt{dF_{\omega, i}}\sqrt{dF_{\omega', i}}\Big)\\
    % &=2\Big(1- \prod_{i=1}^{T}\big(1 - \frac{H^2(\d F_{\omega, i}, \d F_{\omega', i})}{2}\big)\Big)\\&\leq 2\Big(1-\min_{1 \leq i \leq T}\big(1-\frac{H^{2}(\d F_{\omega,i},dF_{\omega^{'},i})}{2}\big)^{T}\Big)\\&\leq 2\Big(1-\min_{u \in \com}\big(1-\frac{I_{0}|f_{\omega}(u)-f_{\omega'}(u)|^2}{2}\big)^{T}\Big) \\&= 2\Big(1-\big(1-\max_{u\in\com}\frac{I_{0}|f_{\omega}(u)-f_{\omega'}(u)|^2}{2}\big)^{T}\Big)\\
    2\left(1 - \left(1 - \frac{I_{0}r^2T^{-1}}{2}\right)^T\right)\enspace,
\end{align*}
% where the last inequality is granted if $r< v_{0}T^{1/2}$ due to \eqref{distribution}. 
Letting $r^{2} \leq 2/I_{0}$, we deduce that
\begin{align*}
    H^2(\mathbf{P}_{\omega,T} , \mathbf{P}_{\omega',T})&\leq 2\Big(1 - \big(1 - T^{-1}\big)^T\Big)
    \leq
    % 2(1-\frac{1}{
    % 4})=
    3/2\enspace.
\end{align*}
 Thus, \cite[Theorem 2.12]{Tsybakov09} yields
\[
\inf_{\hat{\bomega}}\max_{\bomega \in \Omega}\mathbf{E}_{\bomega, T} [\rho(\hat{\bomega},\bomega)] \geq 0.01 \times d \enspace.
\]
Substituting the above into Eq.~\eqref{eq:lower_bound_quadratic1} we conclude that
\begin{equation*}
 \max_{\bomega \in \Omega}\mathbf{E}_{\bomega,T}\big[\norm{\bz_{T}-\bx^{*}_{\bomega}}^{2}\big]\geq 0.01 \times d\alpha^{-2}r^{2} h^{2} = 0.01 \times r^{2}\min\Big(1, 
\,\frac{d}{\alpha^{2} T}
\Big)\enspace.   
\end{equation*}
Finally, from $\alpha$-strong convexity of $f$ and the above bound, we derive the announced result
\begin{equation*}
\max_{\bomega \in \Omega}\mathbf{E}_{\bomega,T}
\big[f(\bz_T)-f(\bx_\omega^*)\big]\geq
0.005 \times r^{2}\min\Big(\alpha,\frac{d}{\alpha T}\Big)\enspace. 
\end{equation*}

\end{proof}

% \evg[inline]{Todo: make things bold}
\begin{proof}[Proof of Theorem~\ref{thm:lower_grad}]
Clearly, $\mathcal{F}^{'}_{1, \beta} \subset \mathcal{F}_{\beta}$, where $\mathcal{F}^{'}_{1, \beta}$ is the class of Theorem \ref{lb}. As the functions in $\mathcal{F}^{'}_{1, \beta}$ are 1-strongly convex, for $t\geq 1$,
\begin{align*}
    \norm{\nabla f(\bz_t)}^2\geq 2(f(\bz_t) -f^{\star}).
\end{align*}
Using Theorem \ref{lb}, for $T\geq 1$, we have
\begin{align}\label{lbpook1}
    \sup_{f \in \mathcal{F}^{'}_{1,\beta}}\Exp[f(\bz_t)-f^{\star}]\geq \mathcal{C}^{'}dT^{-\frac{\beta-1}{\beta}},
\end{align}
where $\mathcal{C}^{'}>0$ does not depend on $d, T$, and $\beta$.
We have for any random variable $S$ that we consider
$\Exp[\norm{\nabla f(\bz_S)}^2]=\sum_{t=1}^{T}p_{t}\Exp[\norm{\nabla f(\bz_t)}^2],$
where $(p_1,\dots,p_T)$ is a probability vector: $p_t\geq 0$, and $\sum_{t=1}^{T}p_t=1$. Thus,
\begin{align}\label{lbpook2}
   \Exp[\norm{\nabla f(\bz_S)}^2]&\geq 2\sum_{t=1}^{T}p_t\Exp[f(\bz_t)-f^{\star}]
   \geq
   2\Exp\left[f\left(\sum_{t=1}^{T}p_t\bz_t\right)-f^{\star}\right]\enspace.
\end{align}
Note that $\tilde{\bz}_T=\sum_{t=1}^{T}p_t\bz_t$ is an estimator depending only on the past, that is in the same class of estimators as $\bz_T$. Therefore, the bound (\ref{lbpook1}) holds for $\tilde{\bz}_T$ as well. Combining (\ref{lbpook1}) and (\ref{lbpook2}) gives (\ref{lb}).
\end{proof}











% \stopcontents[appendices]
